# Supplementary material for: Expected Improvement versus Predicted Value in Surrogate-Based Optimization
Source: arXiv:2001.02957 ancillary file (2020-02-17)

# Sphere

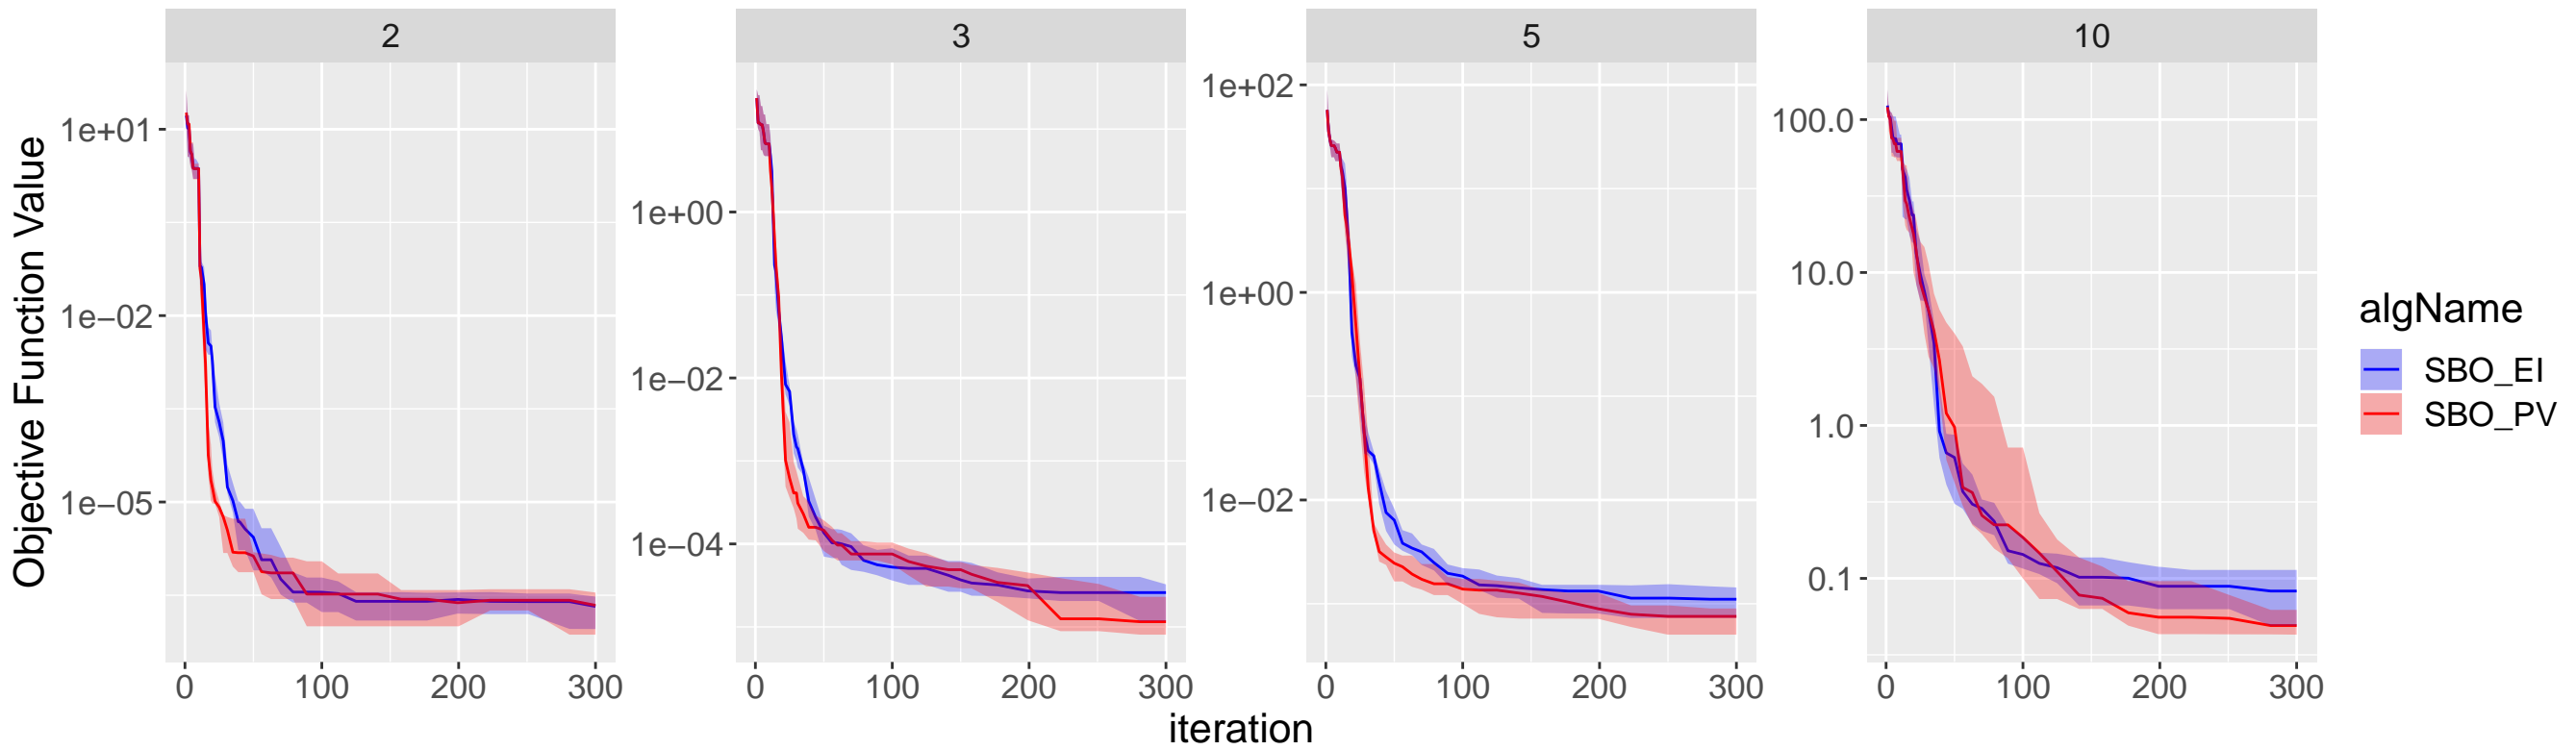

# Ellipsoidal

Objective Function Value

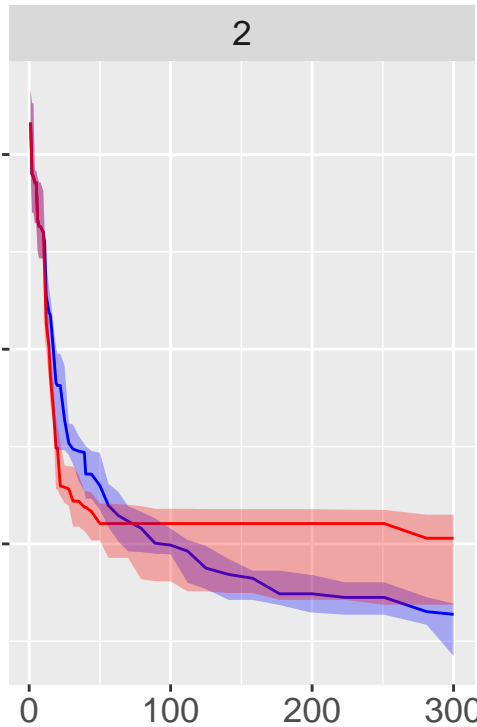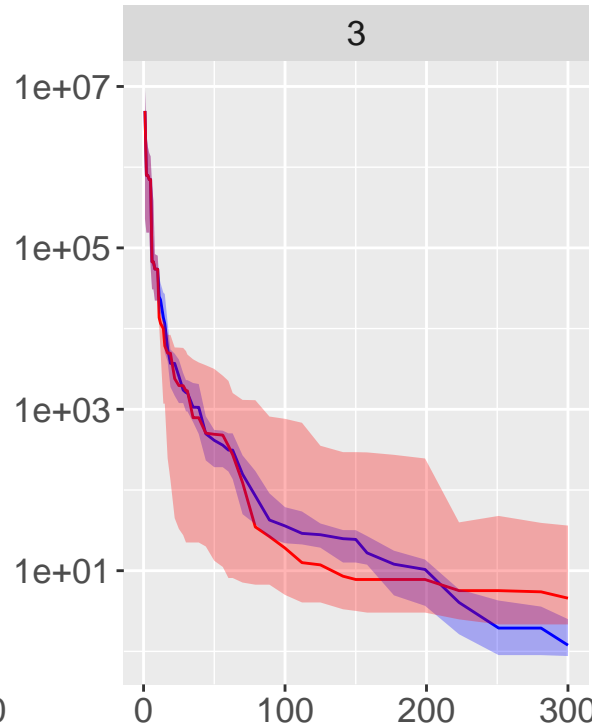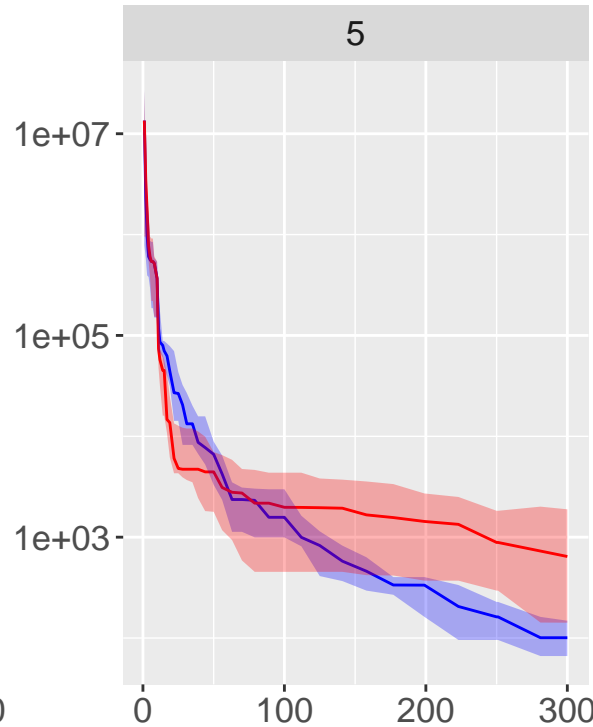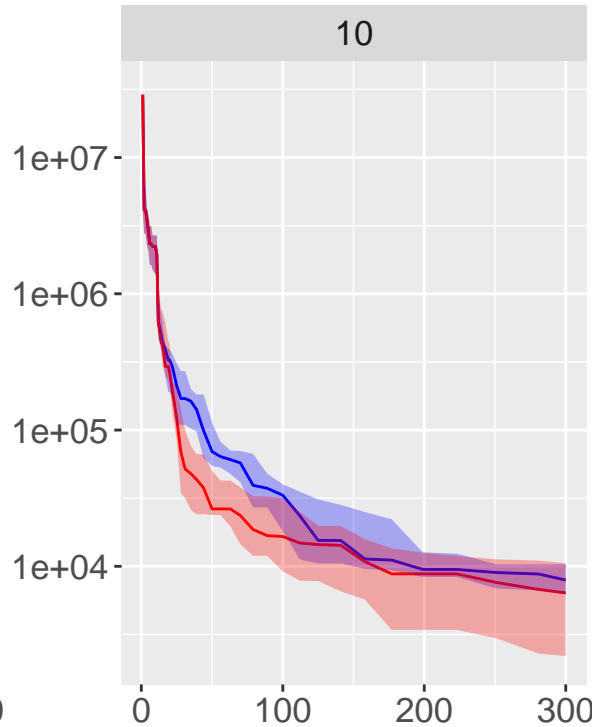

algName

- SBO\_EI
- SBO\_PV

# Rastrigin

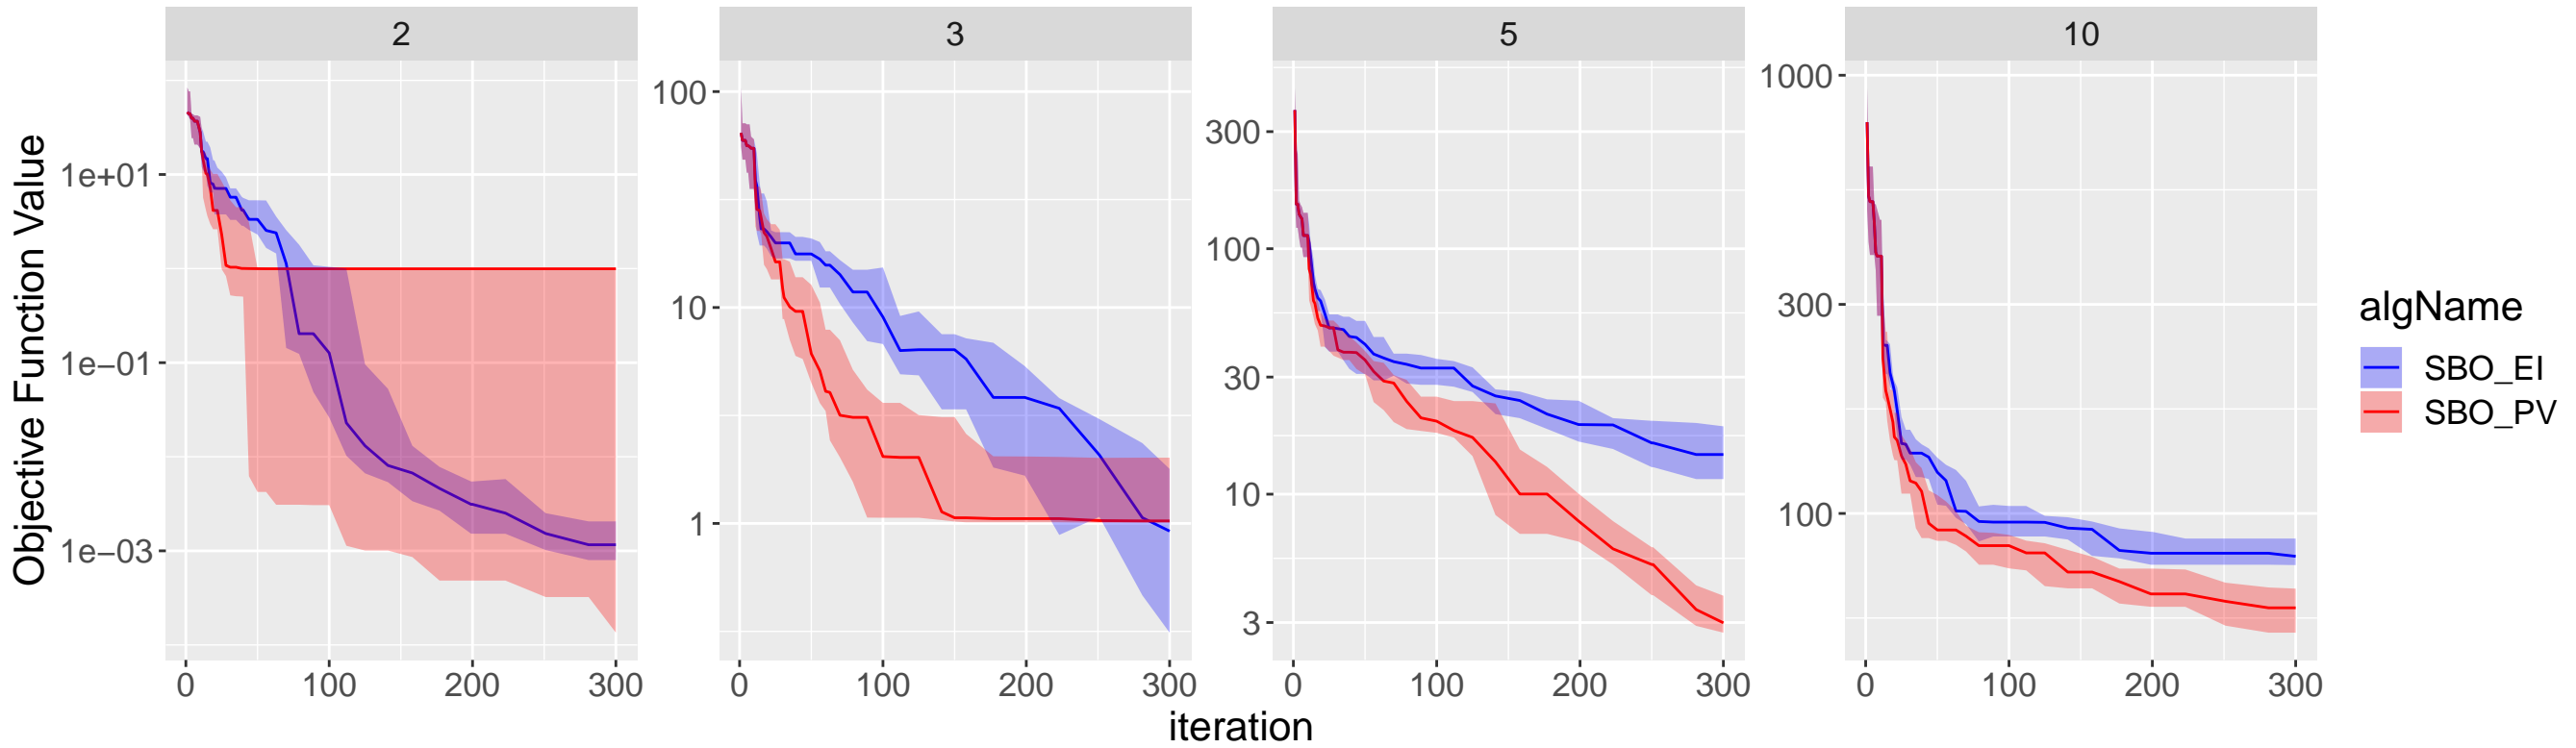

# Büche–Rastrigin

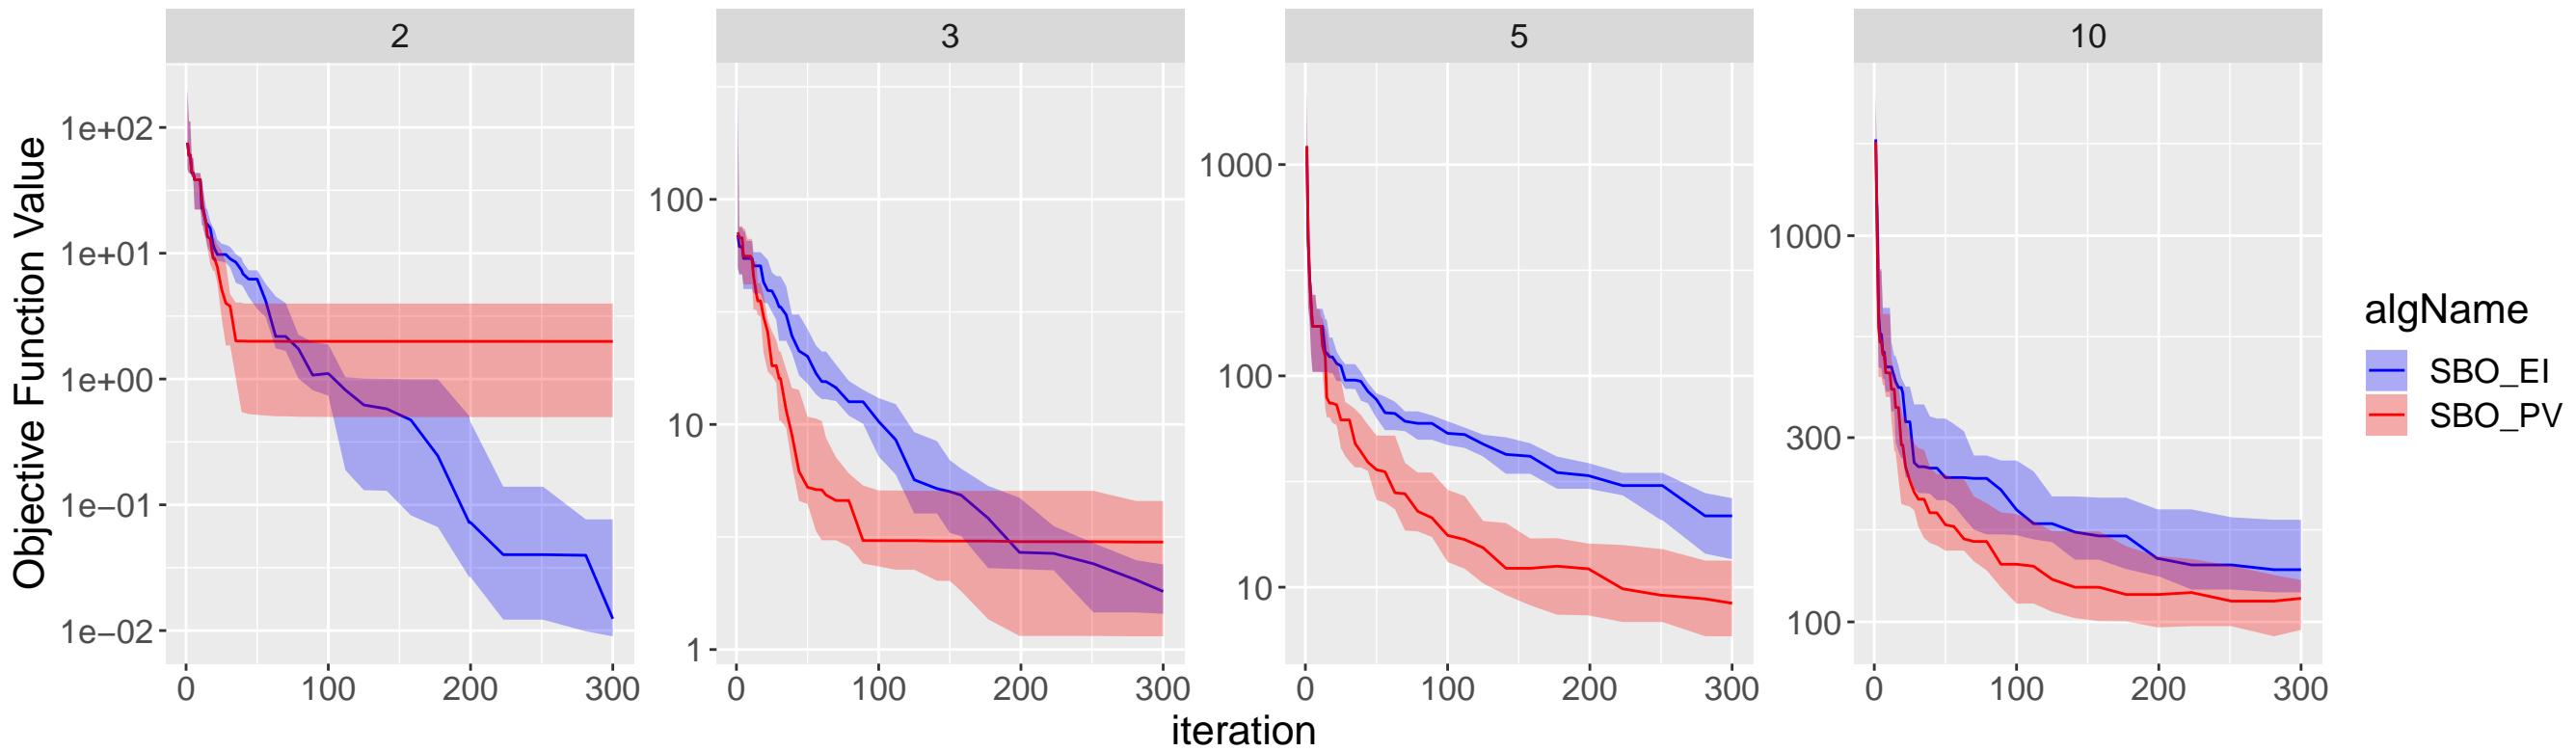

# Linear Slope

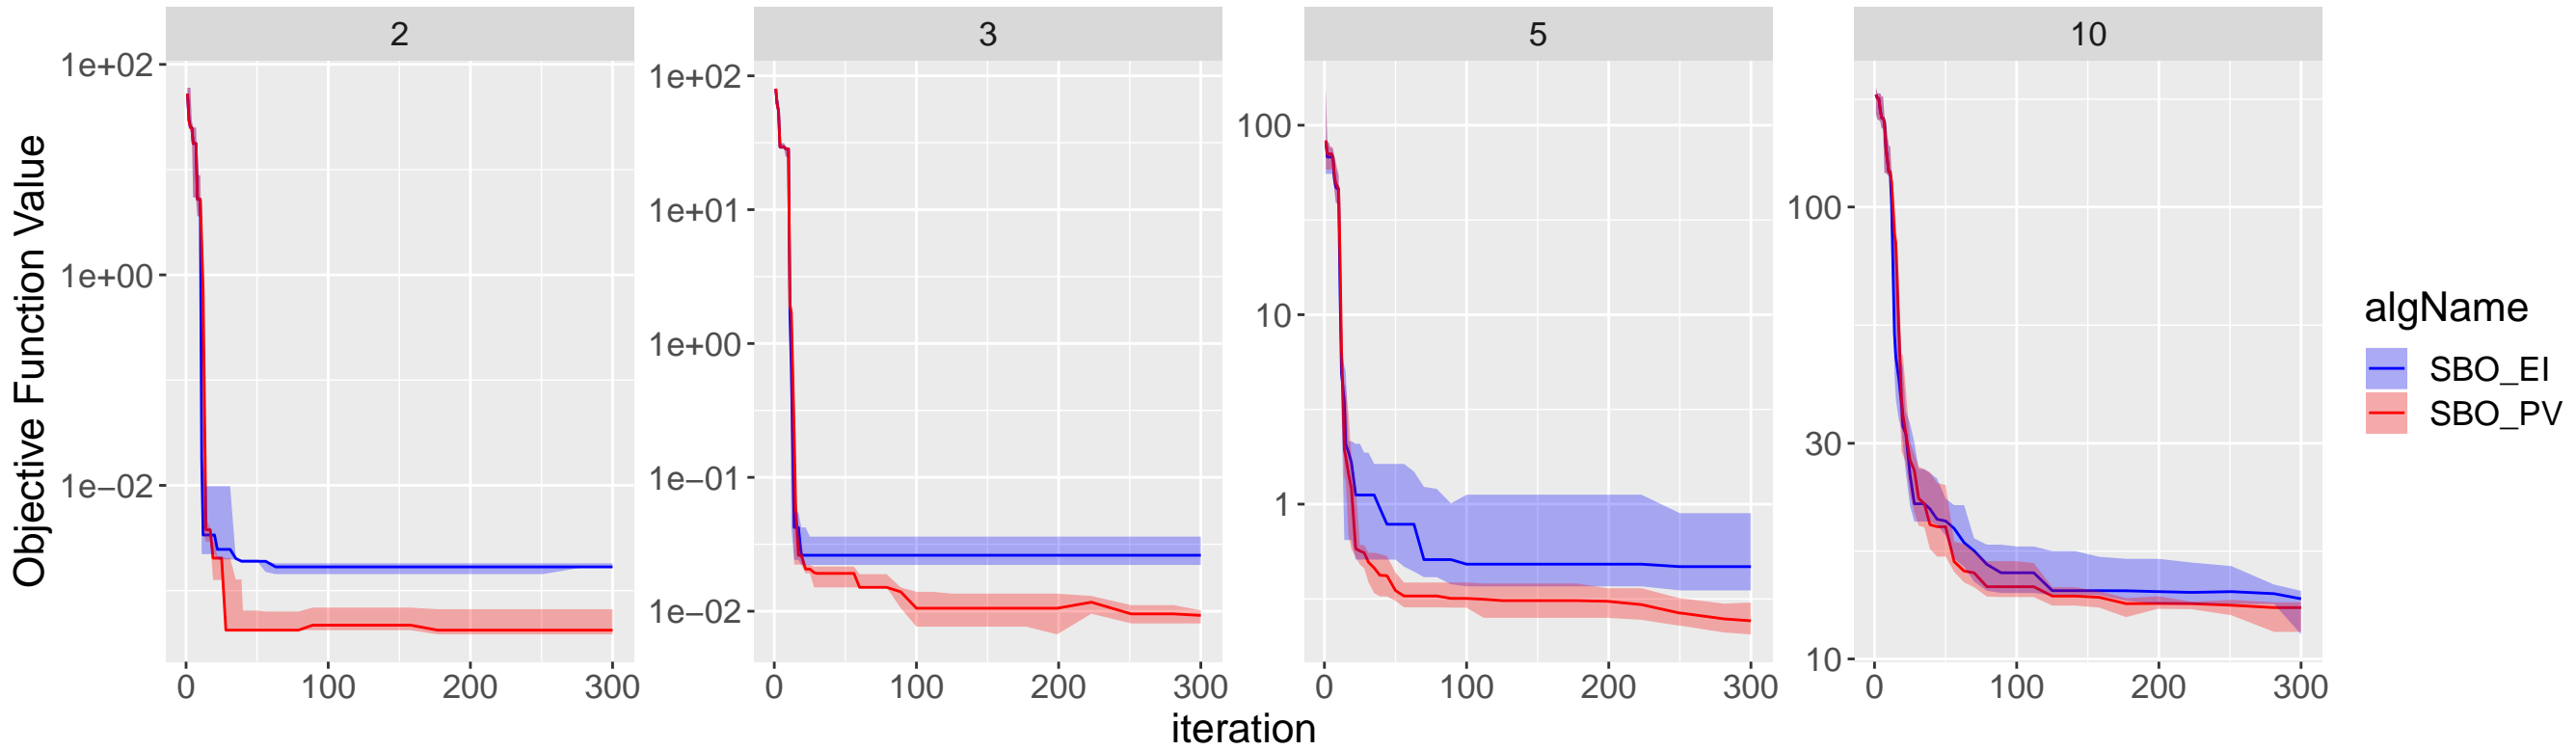

# Attractive Sector

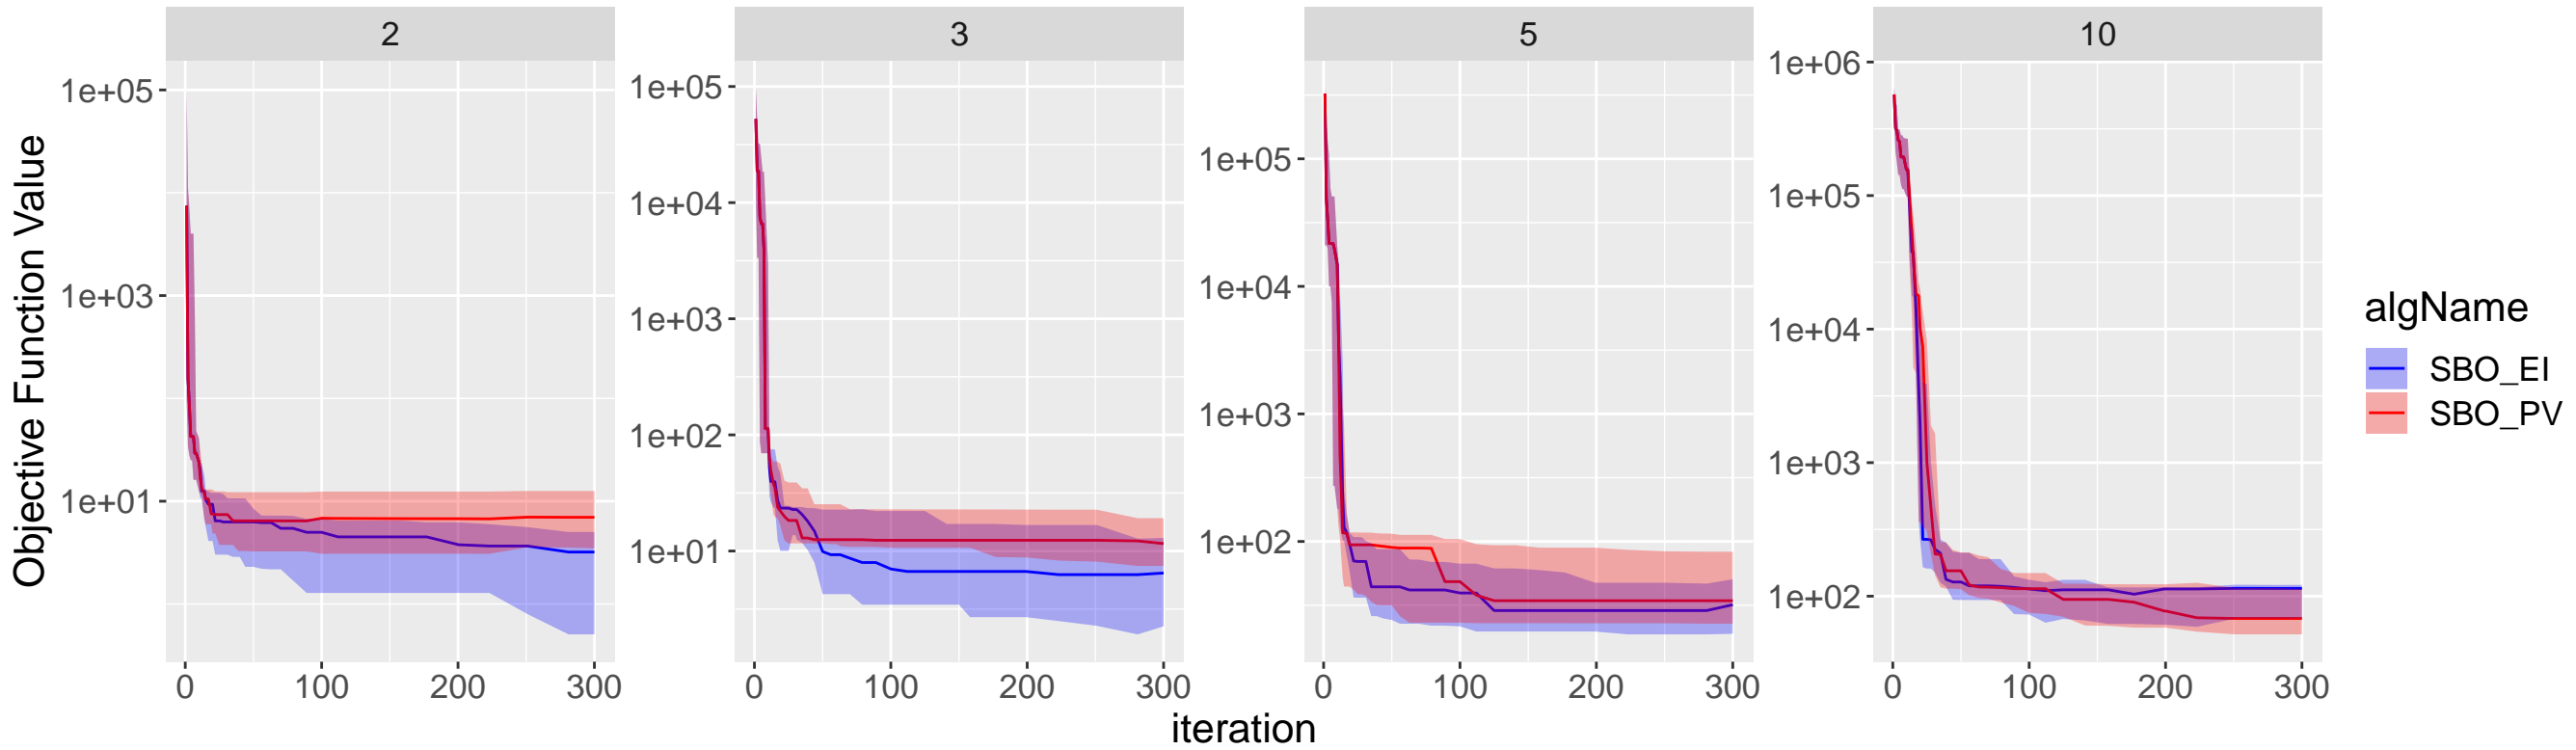

# Step Ellipsoidal

Objective Function Value

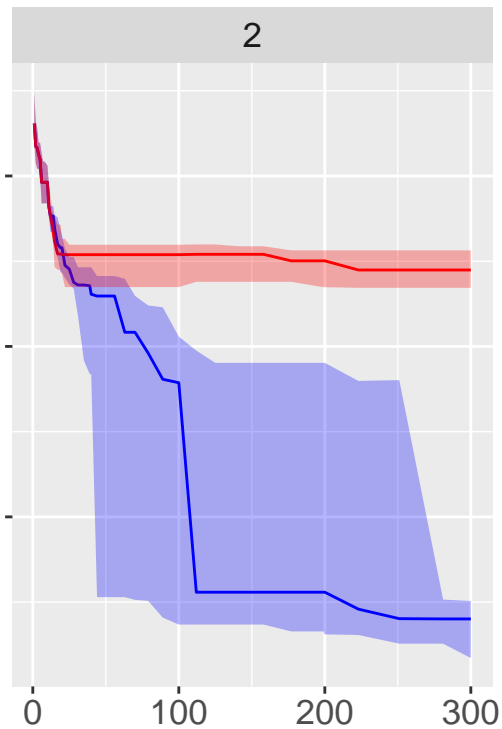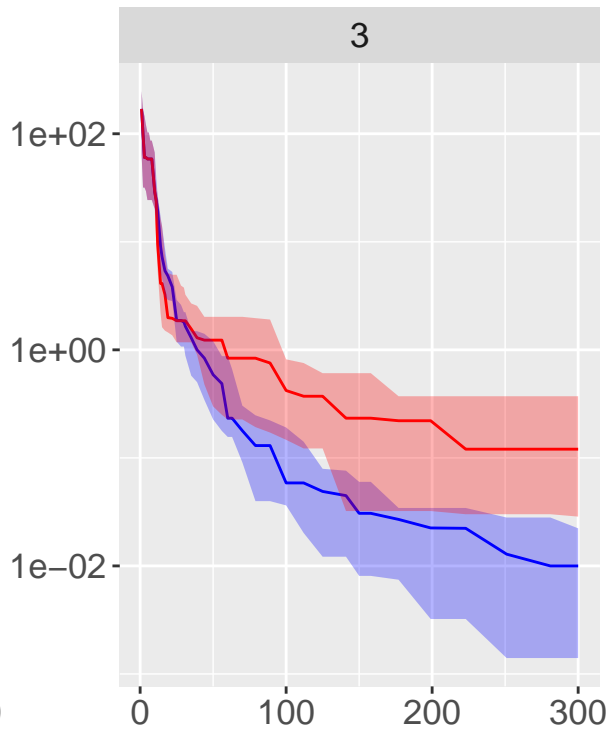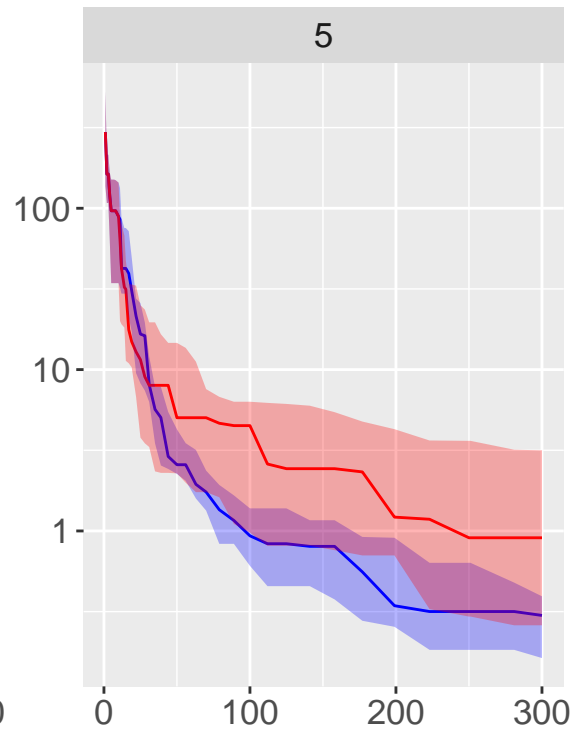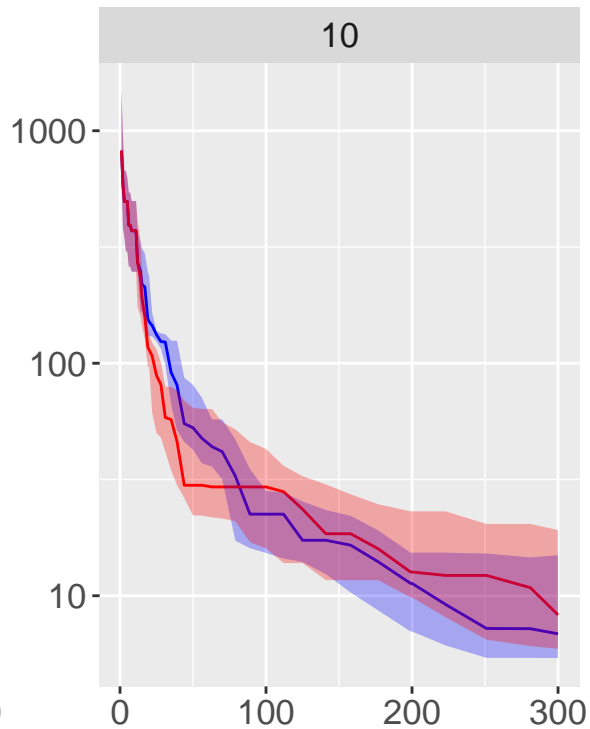

algName

SBO\_EI

SBO\_PV

iteration

# Rosenbrock

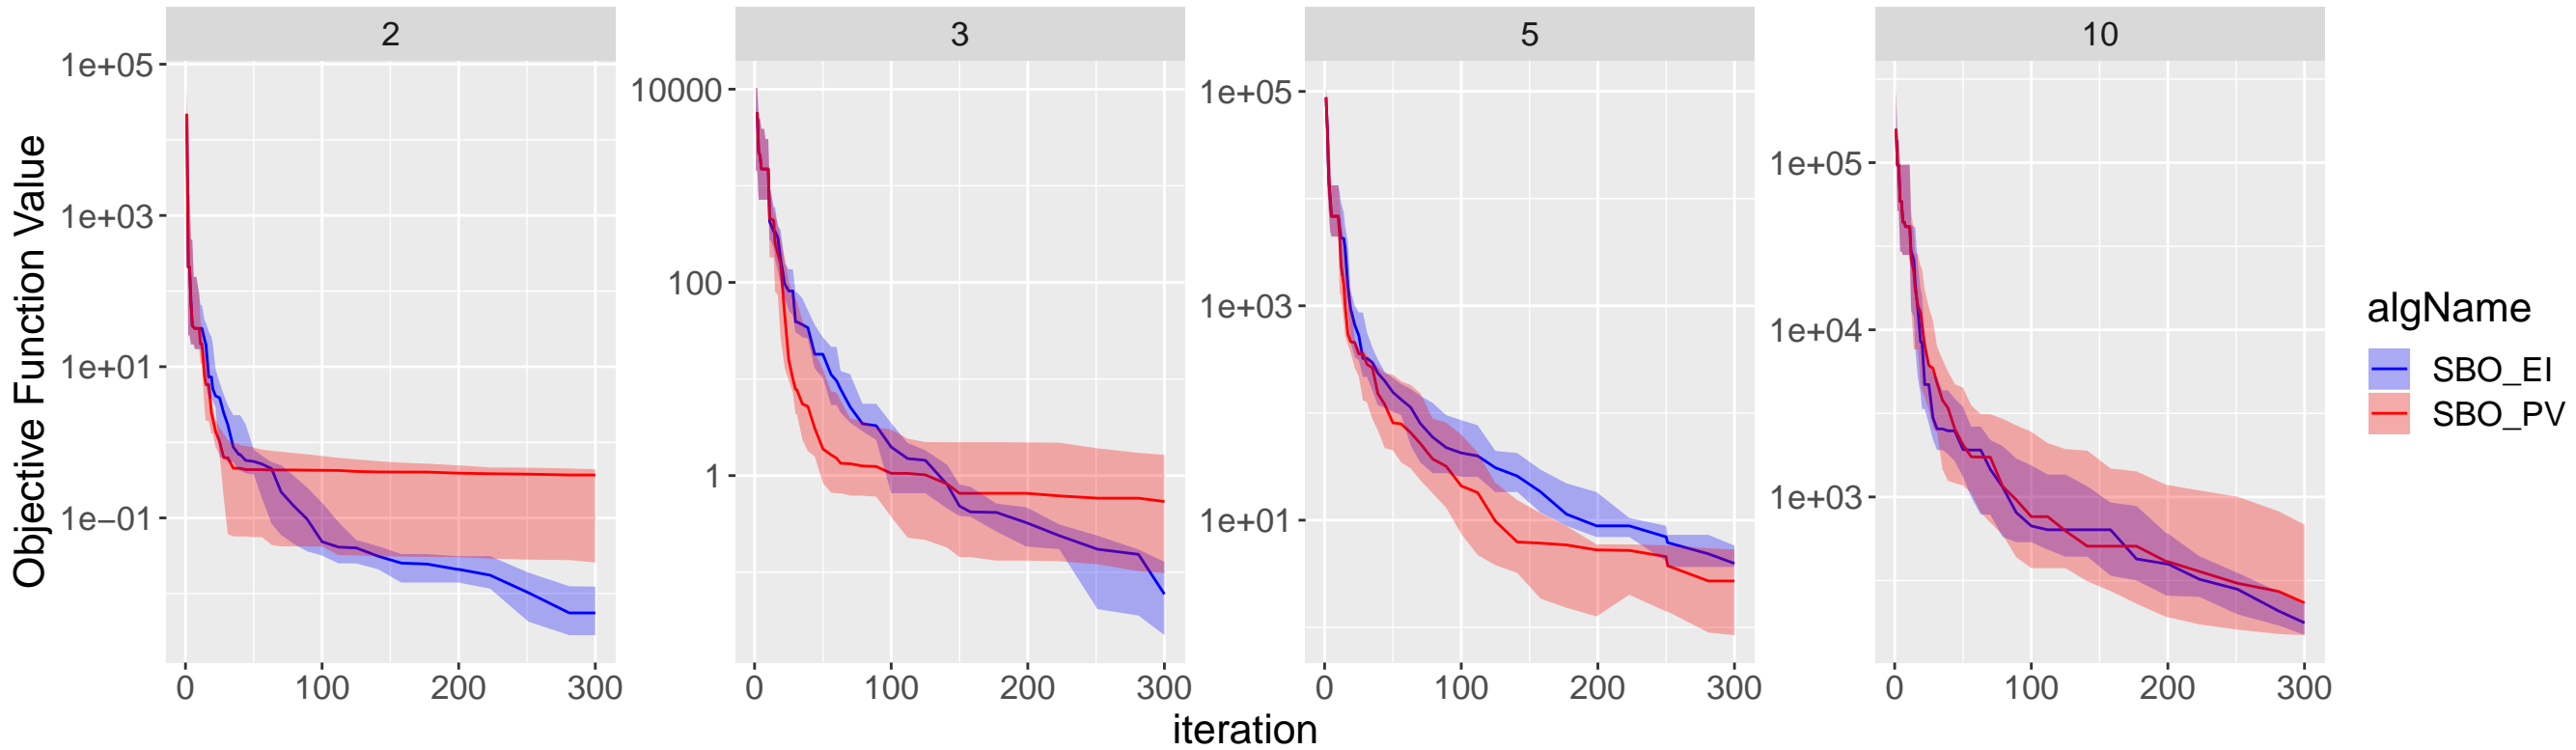



# Rosenbrock, rotated

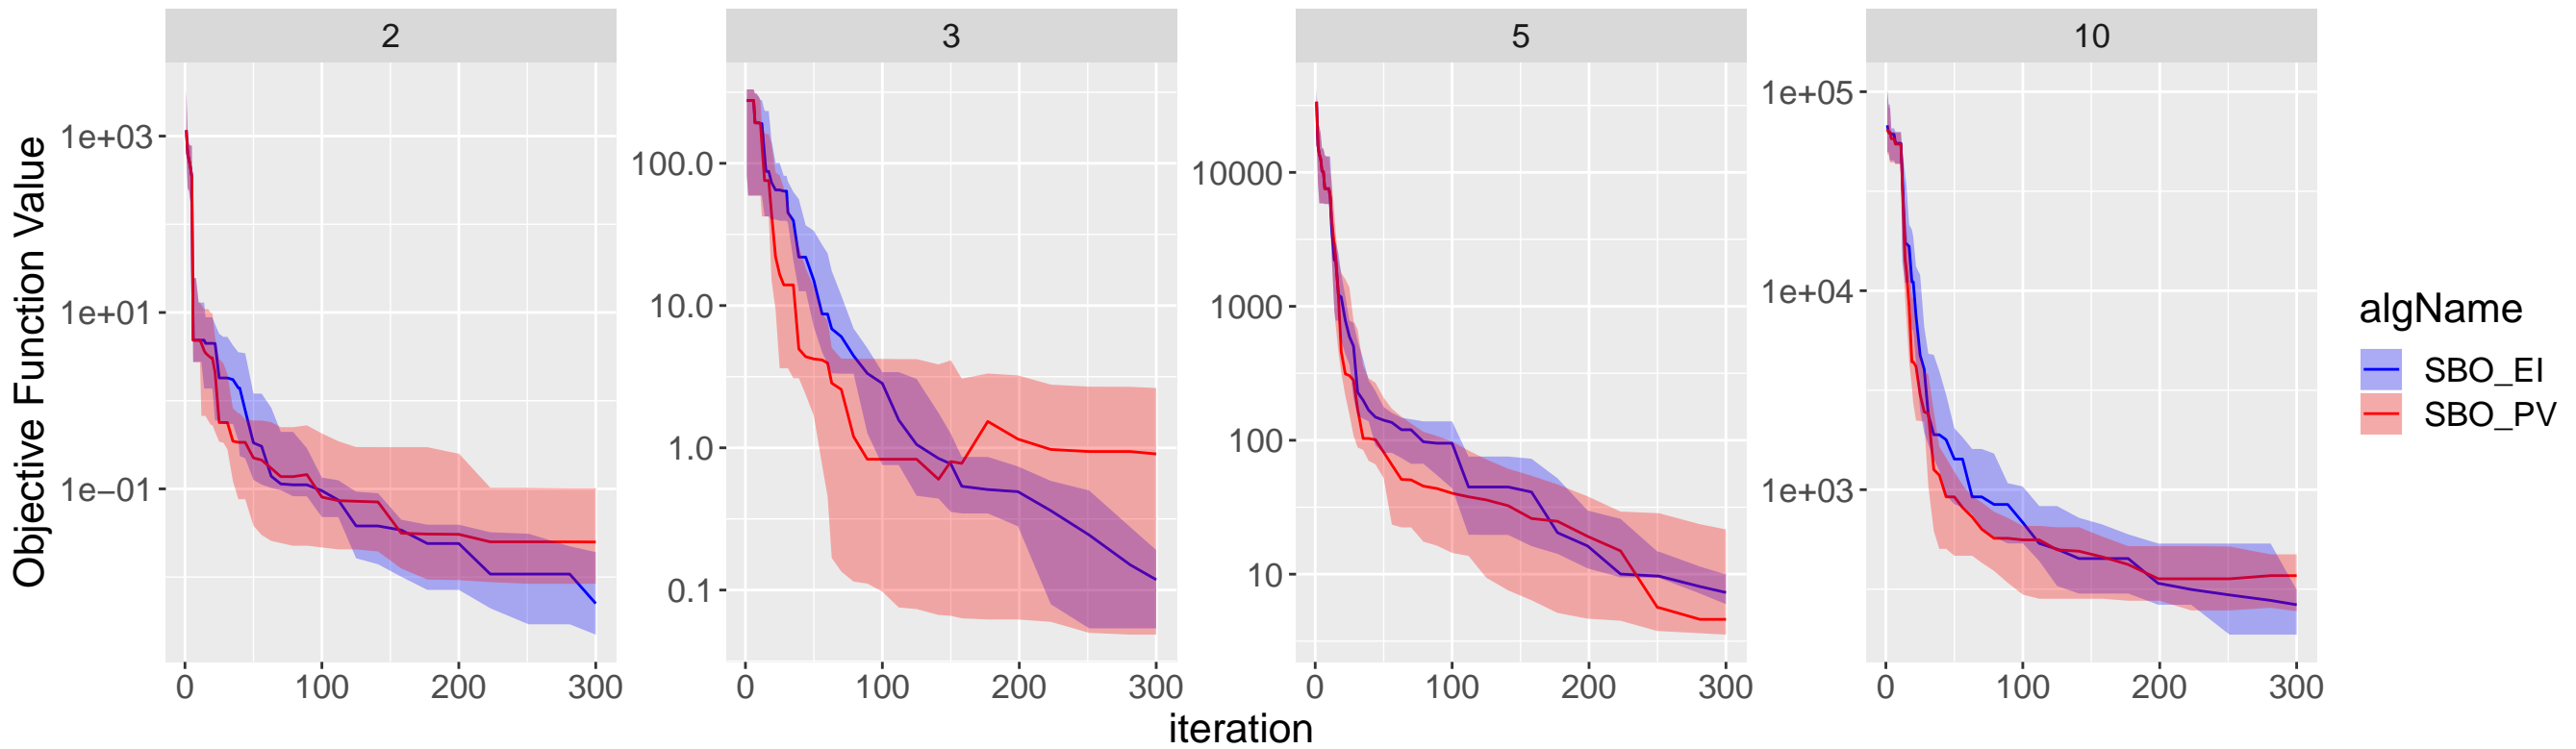

# Ellipsoidal

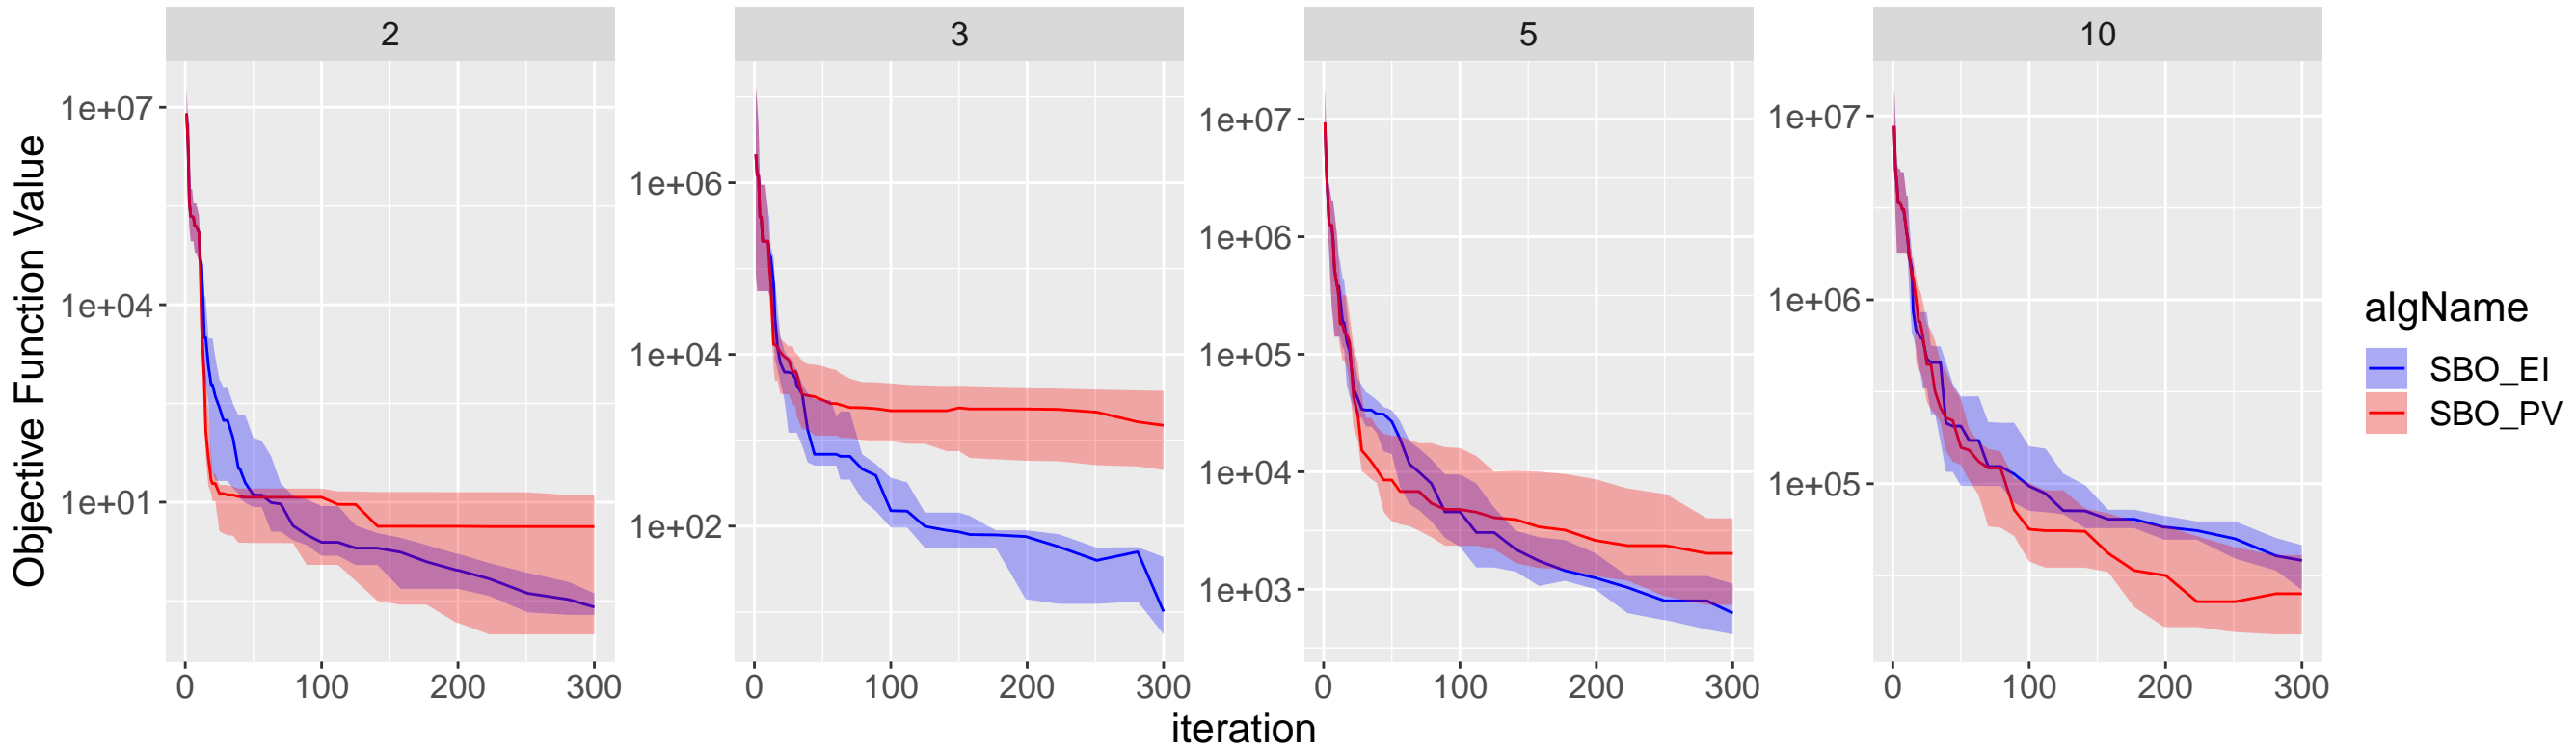

# Discus

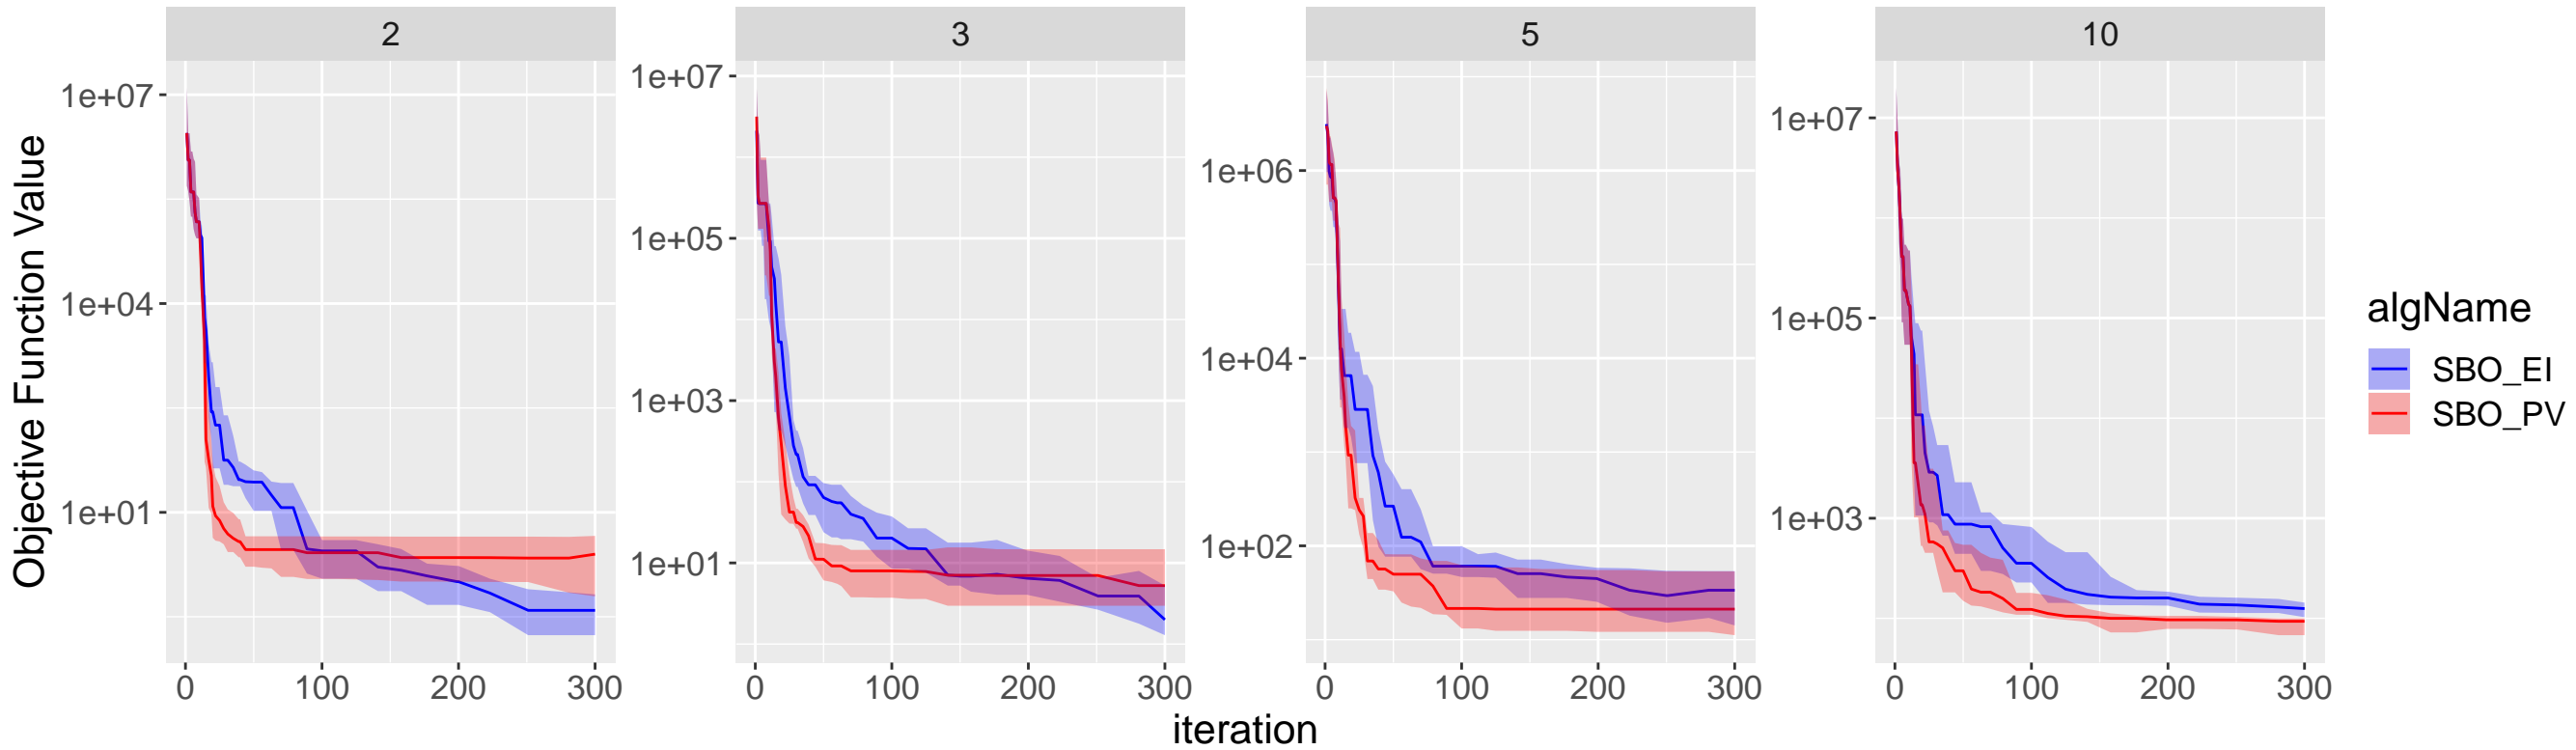

# Bent Cigar

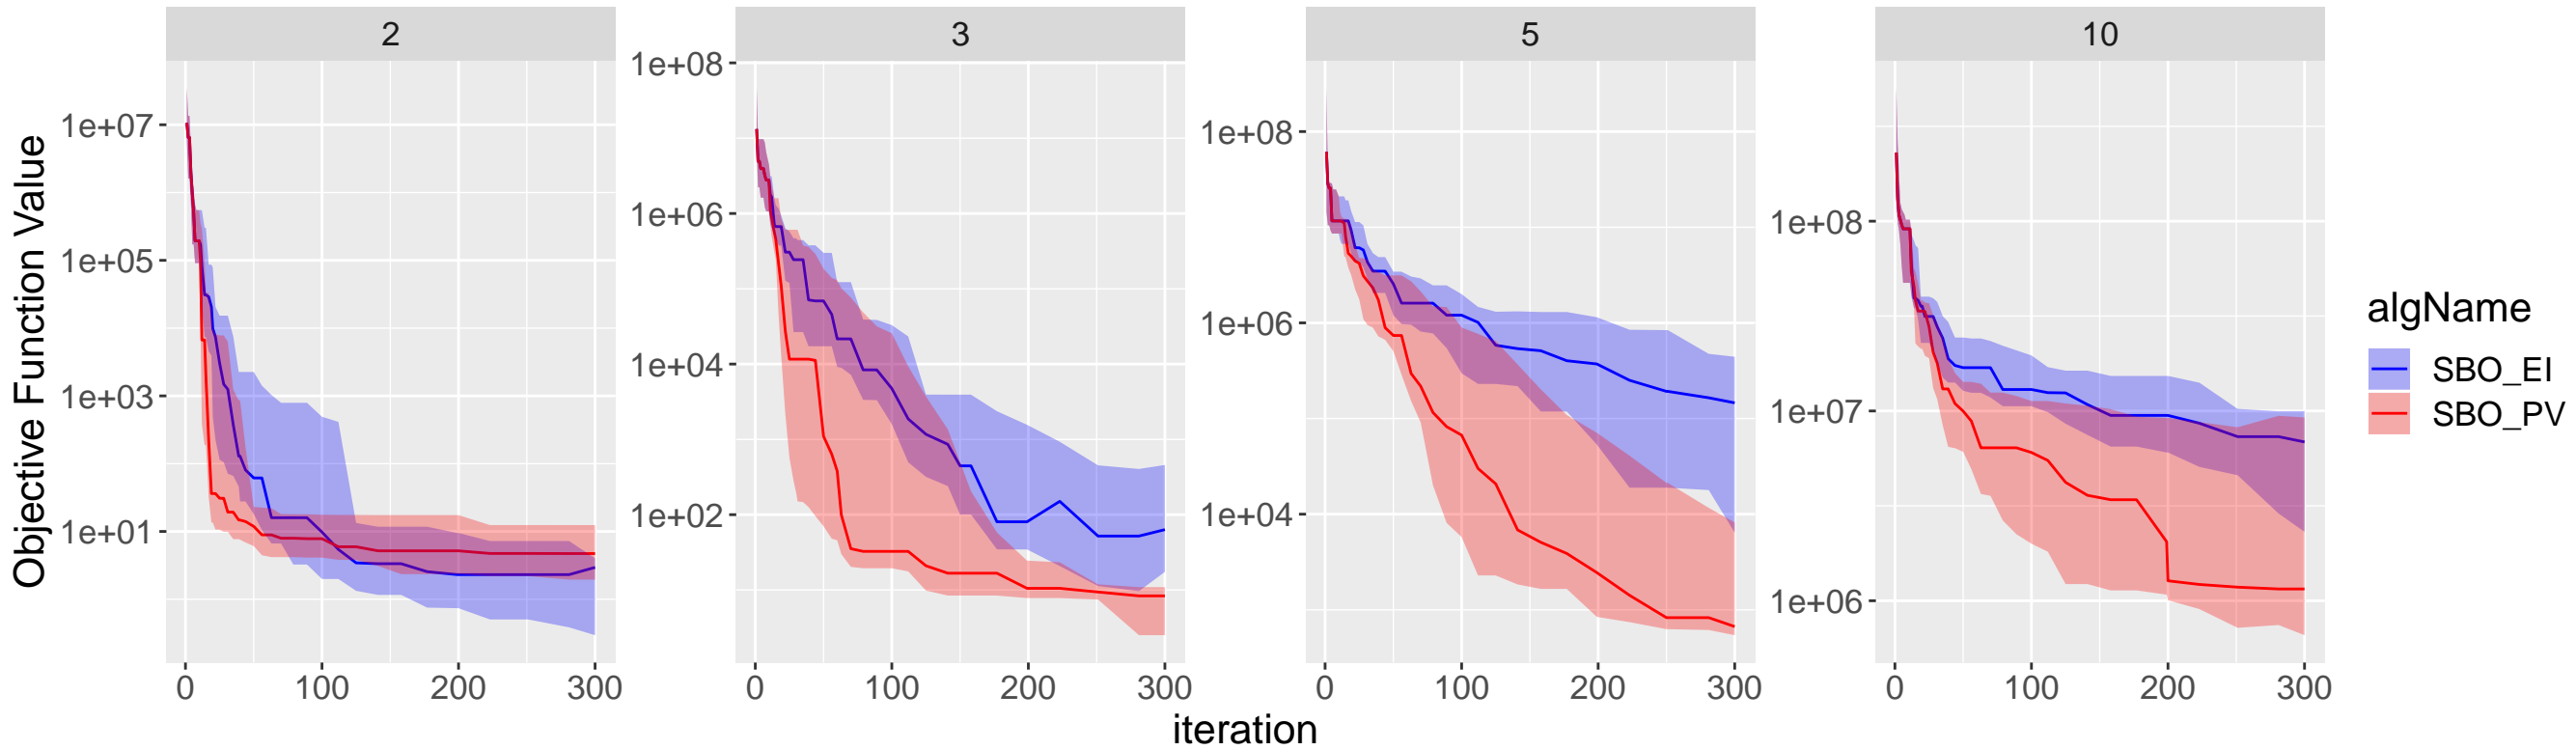

# Sharp Ridge

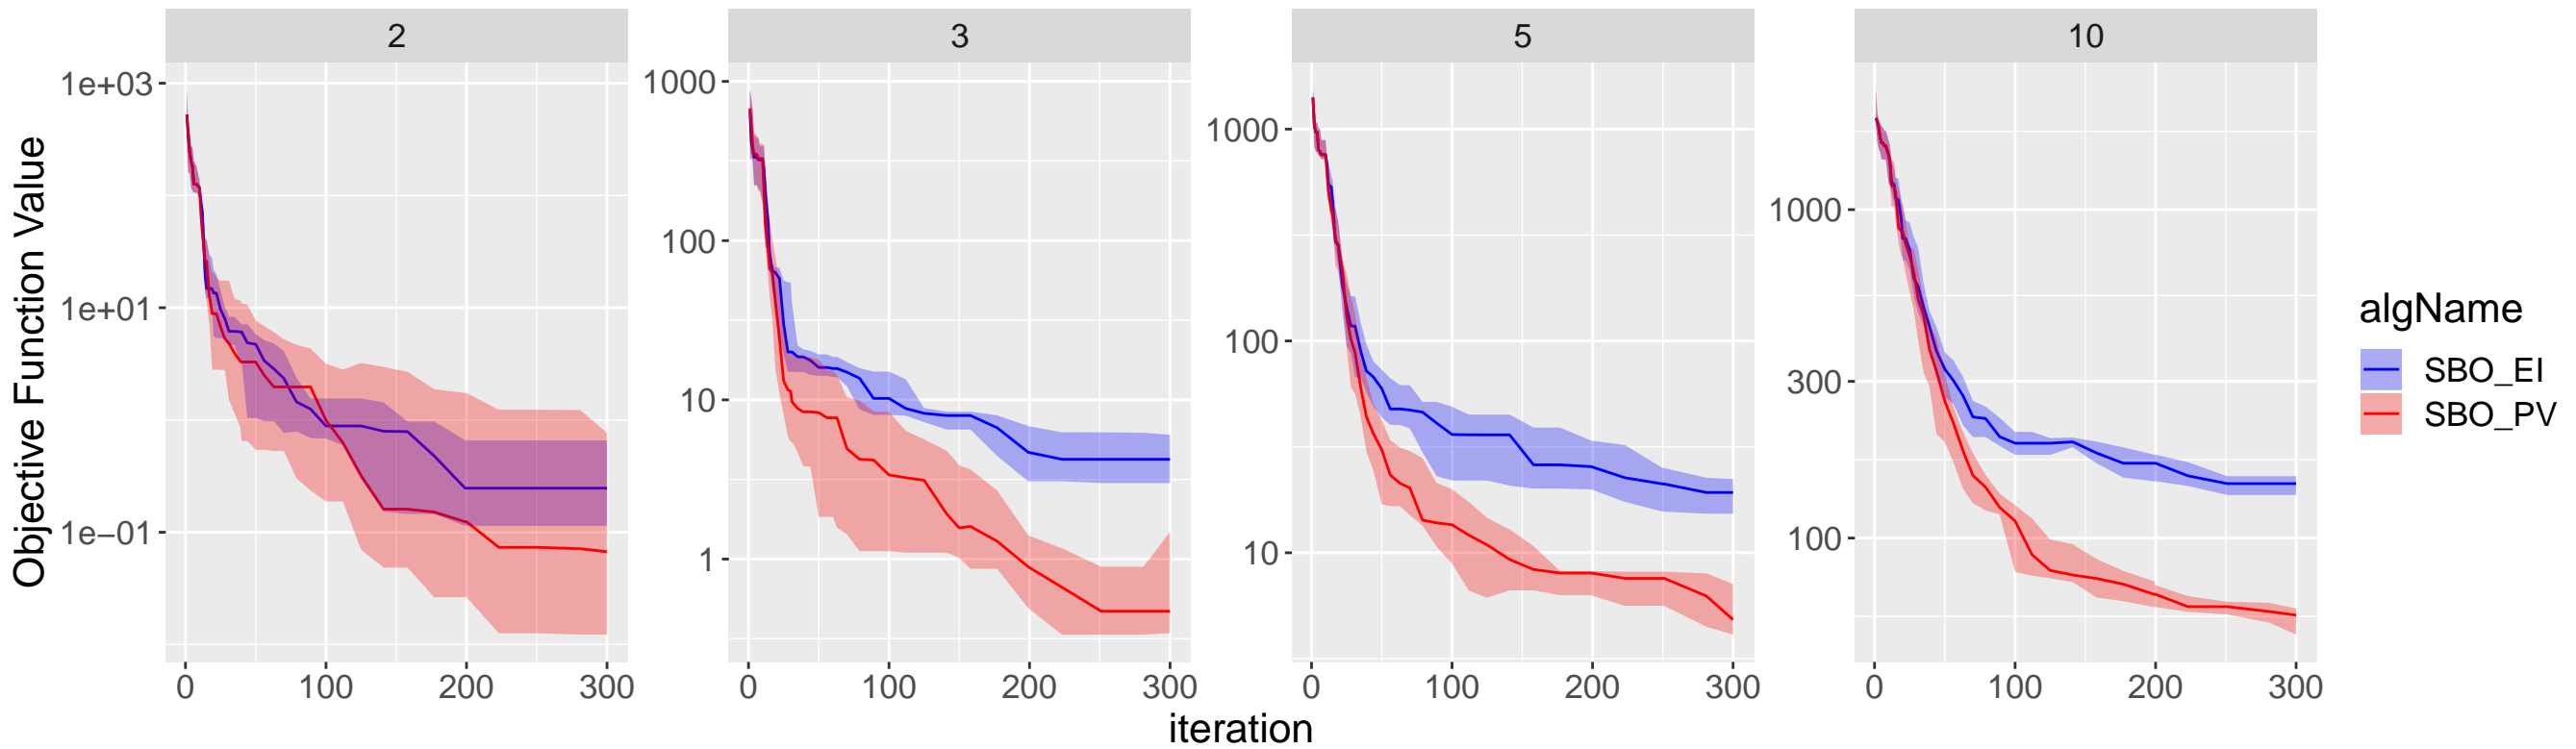

# Different Powers

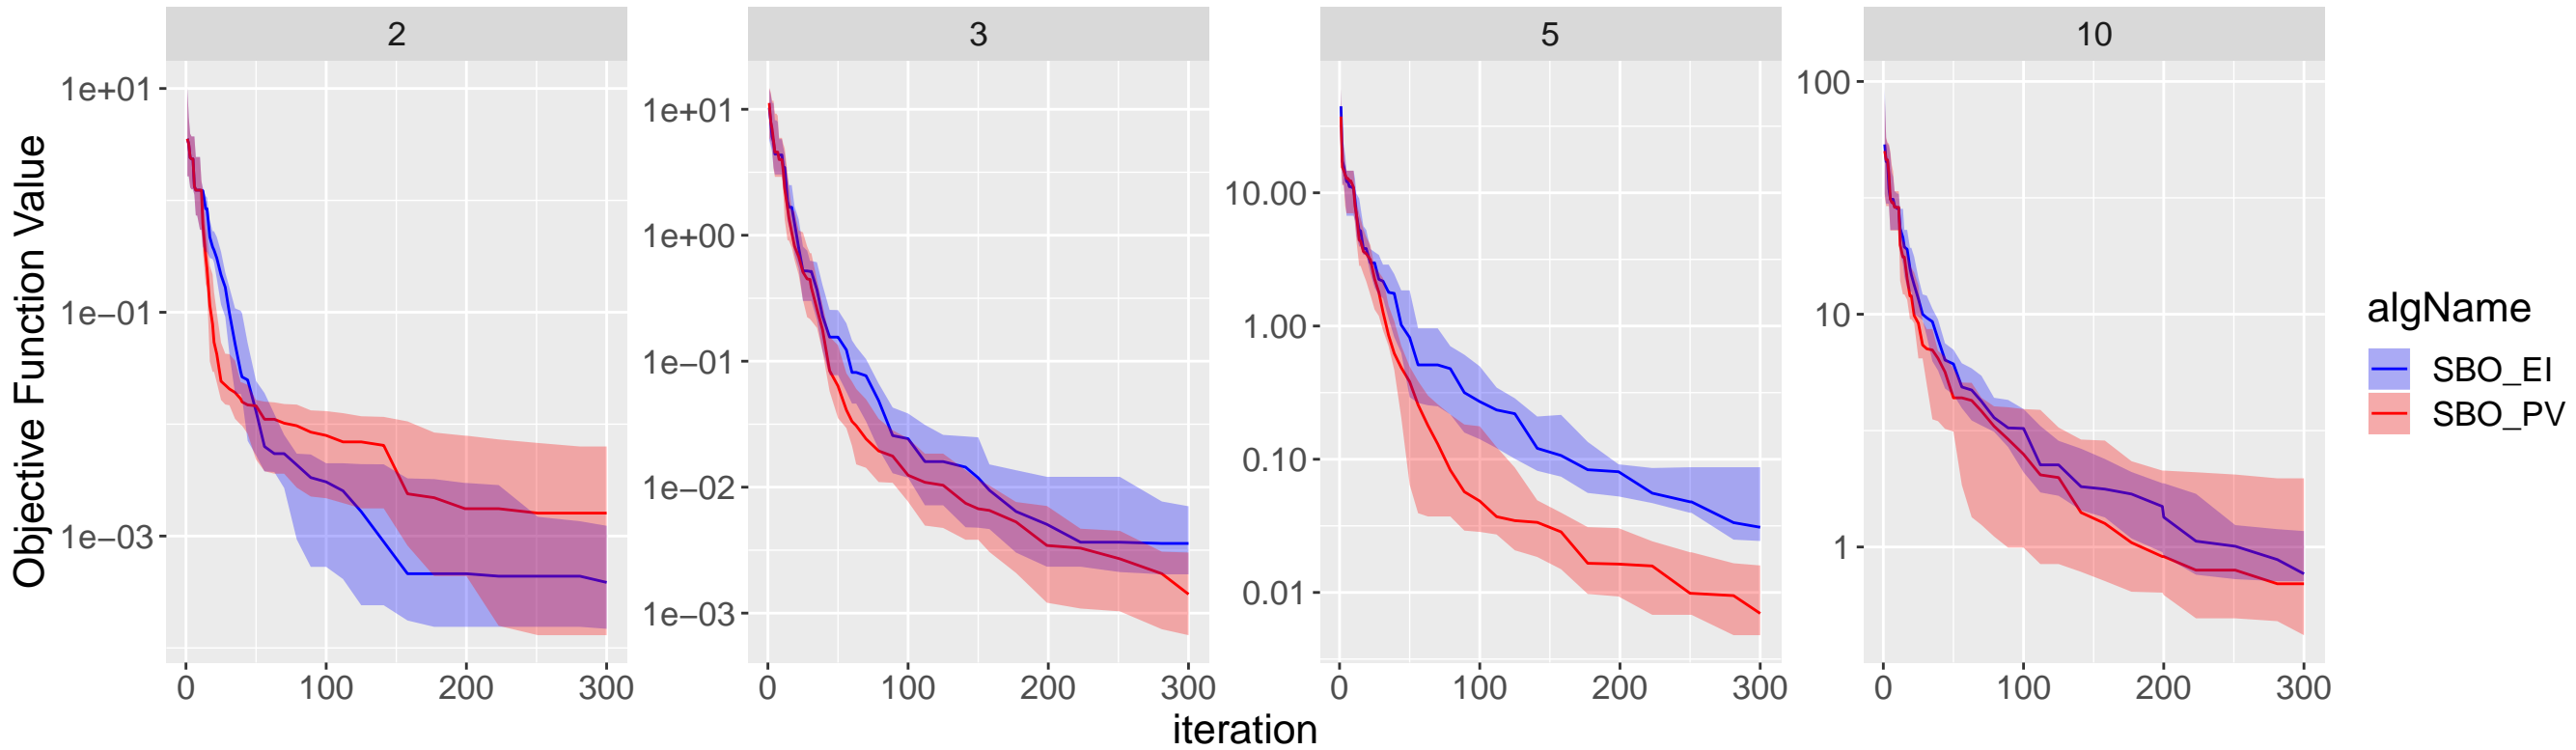

# Rastrigin

Objective Function Value

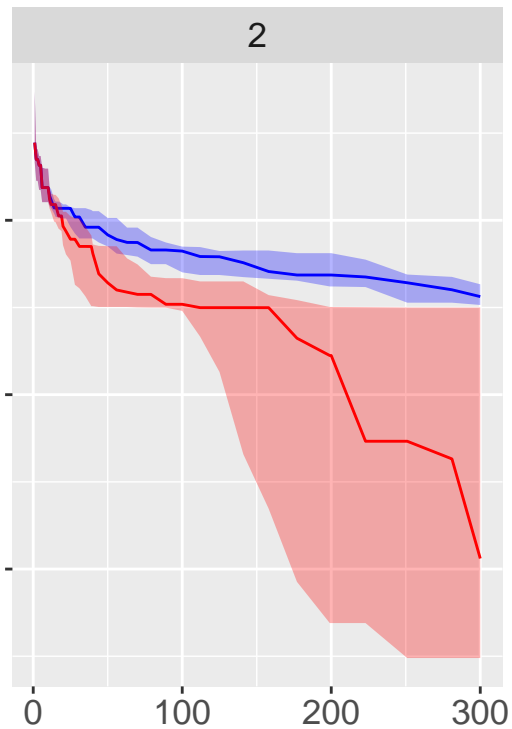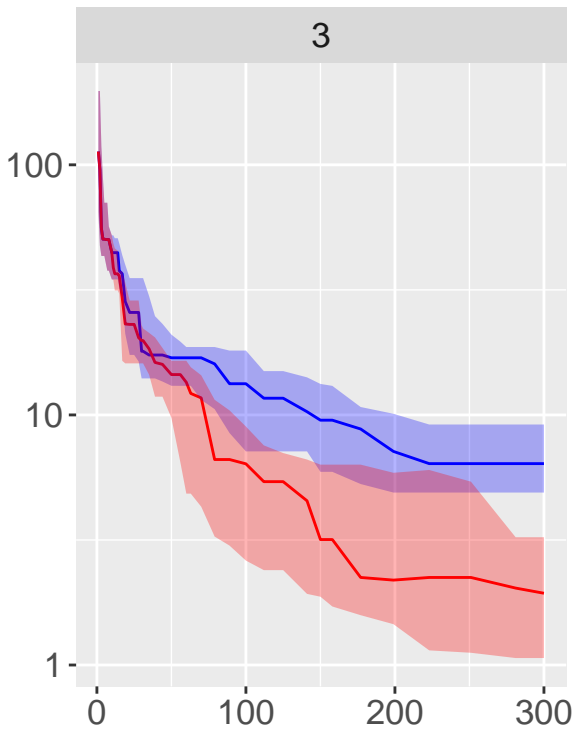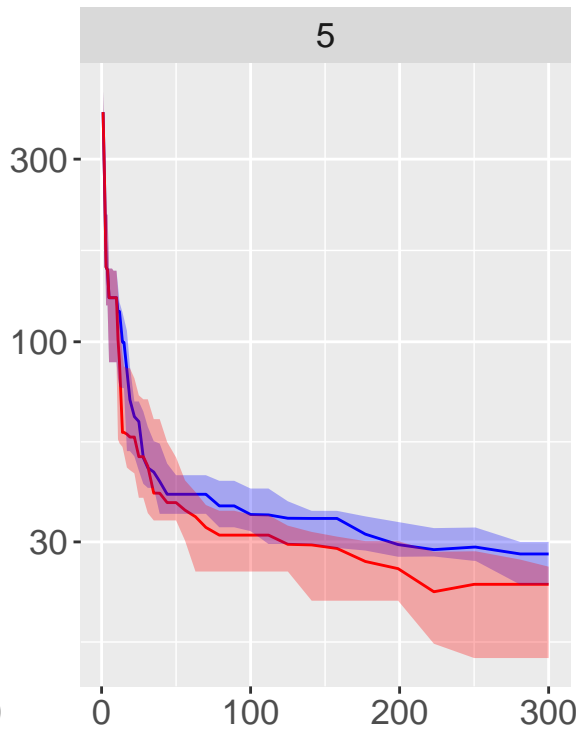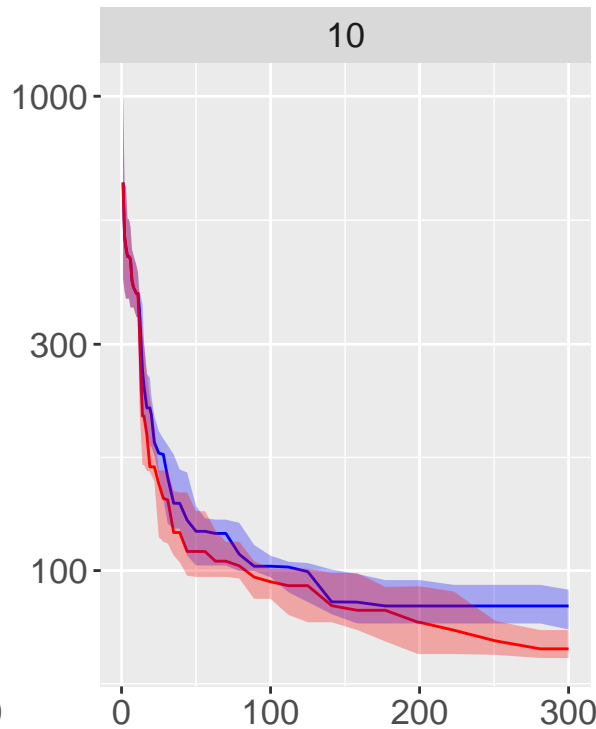

algName

SBO\_EI  
SBO\_PV

# Weierstrass

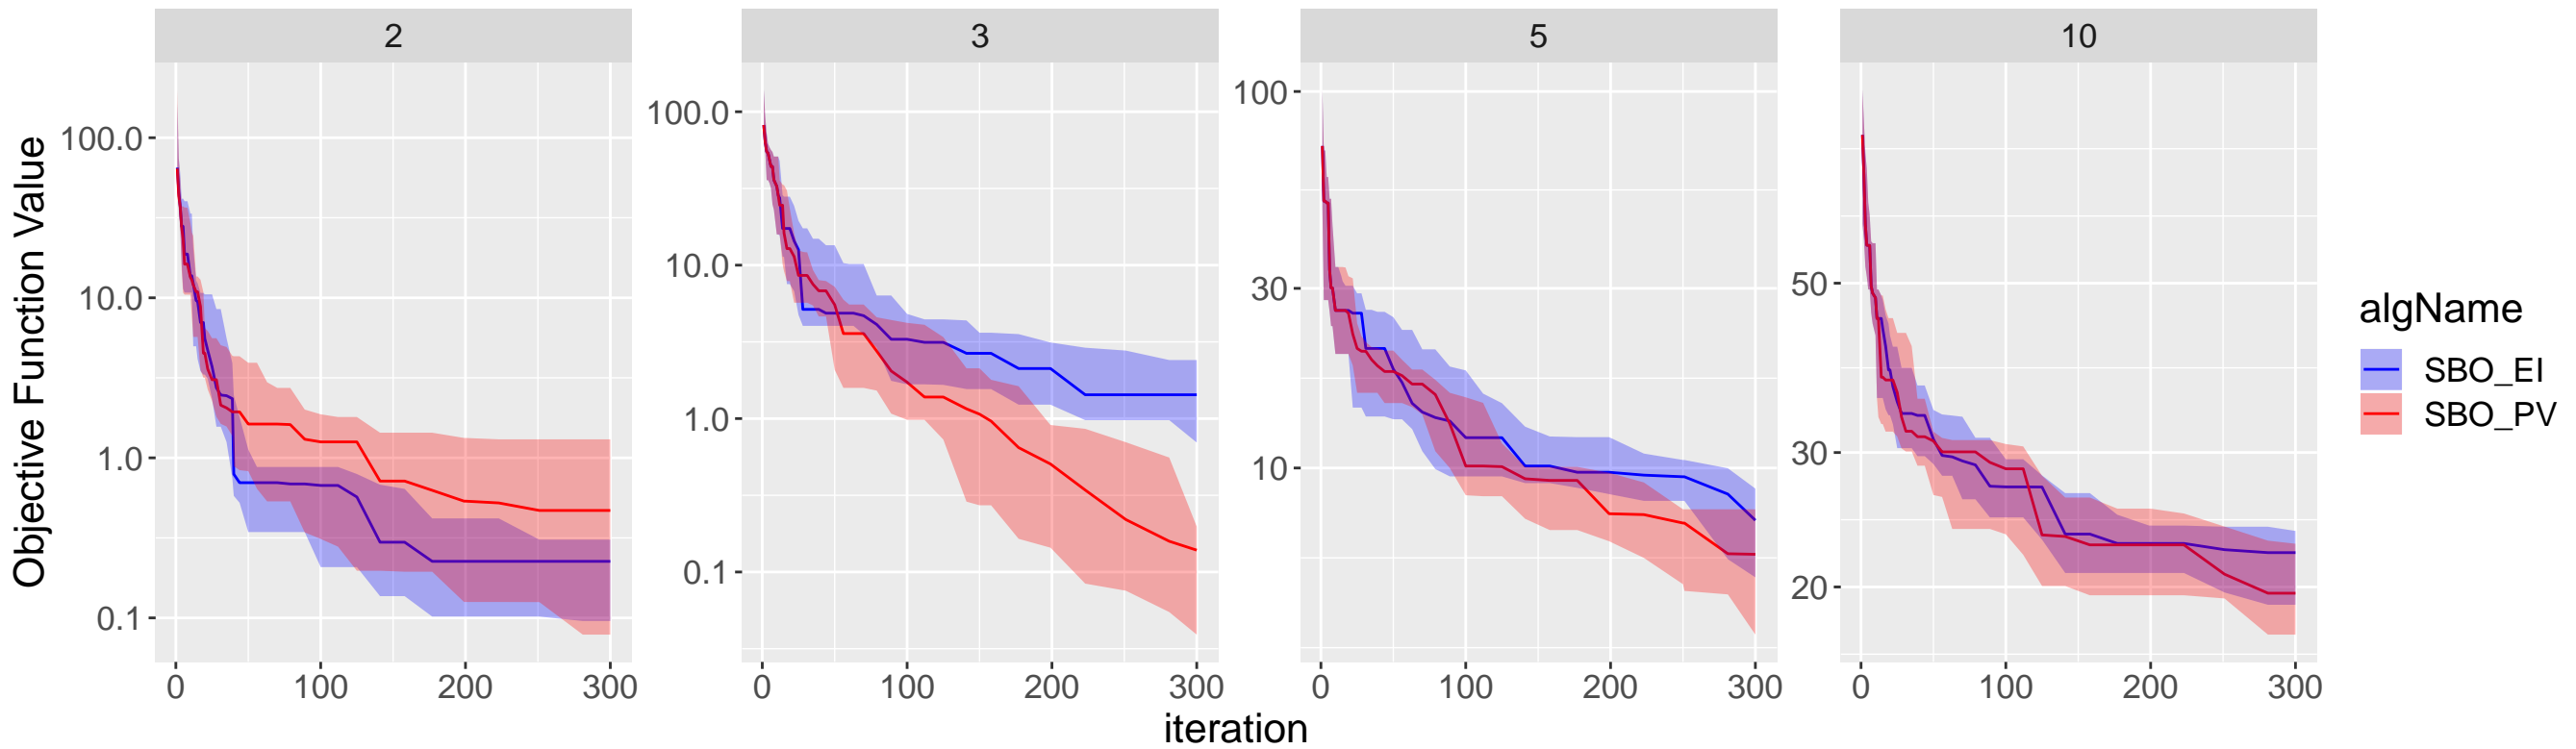



Schaffers F7

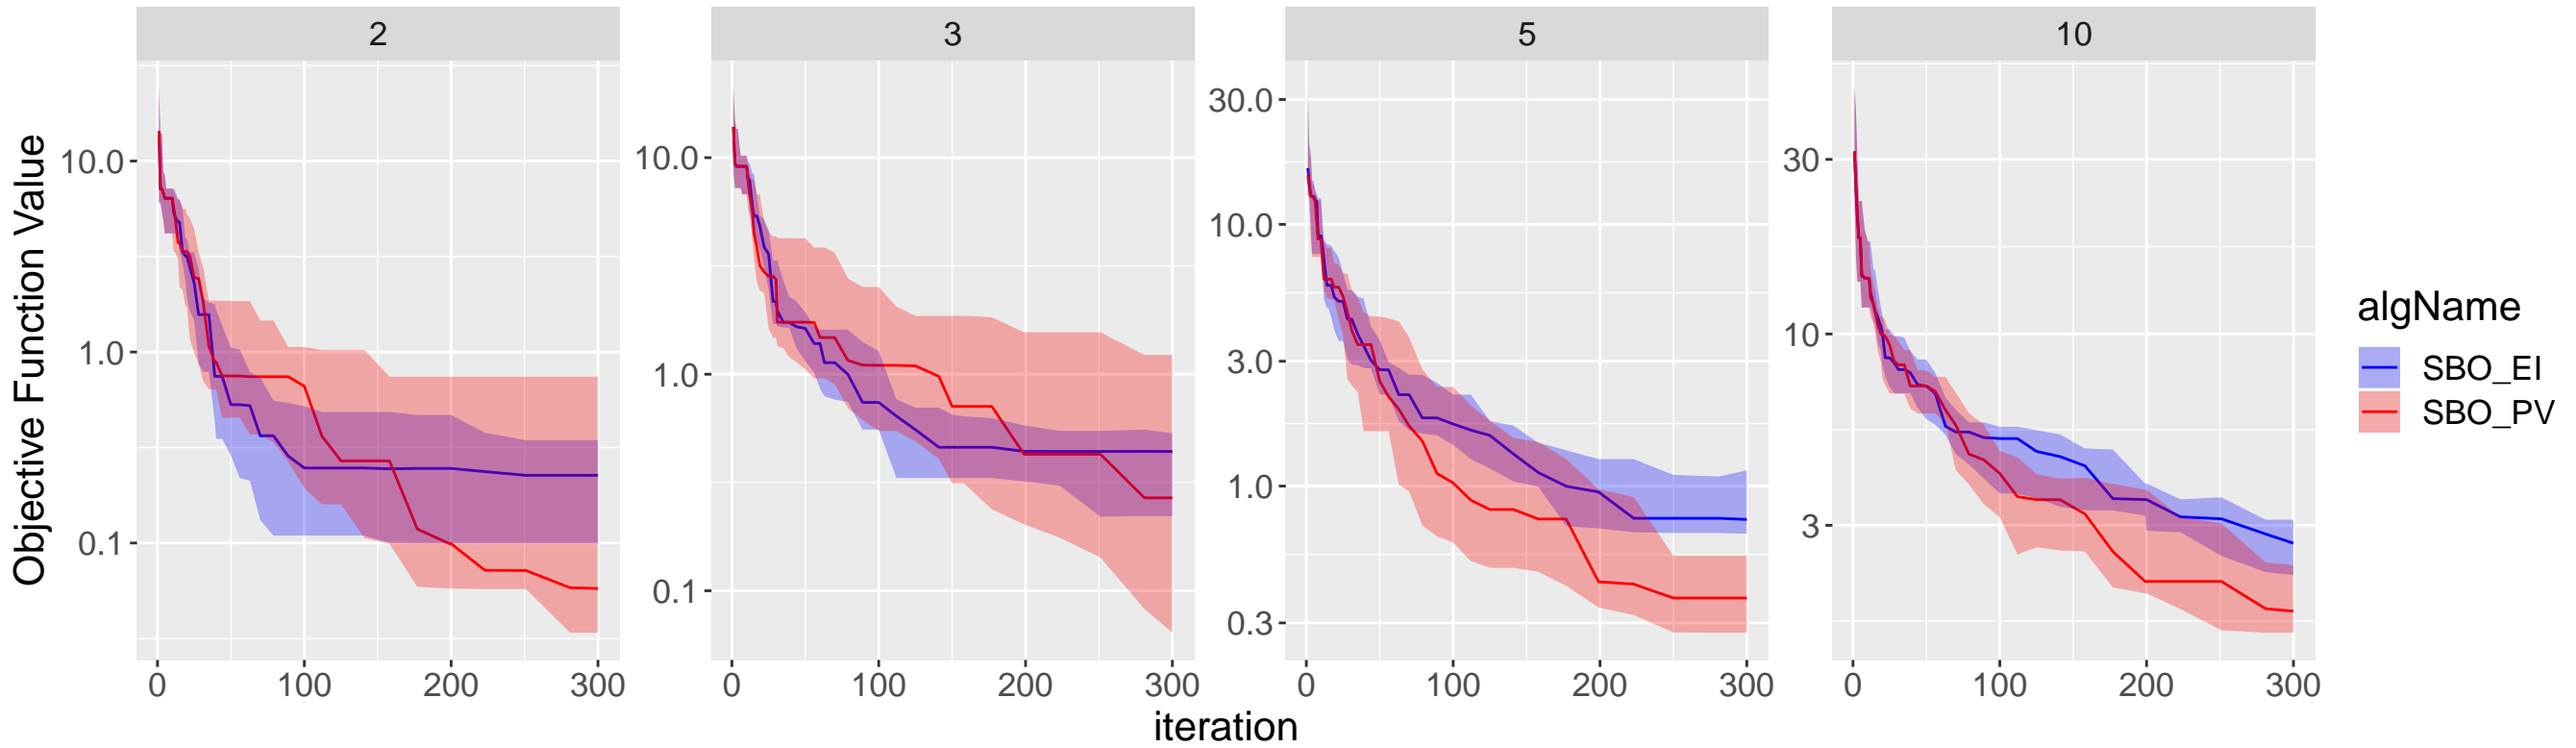

Schaffers F7

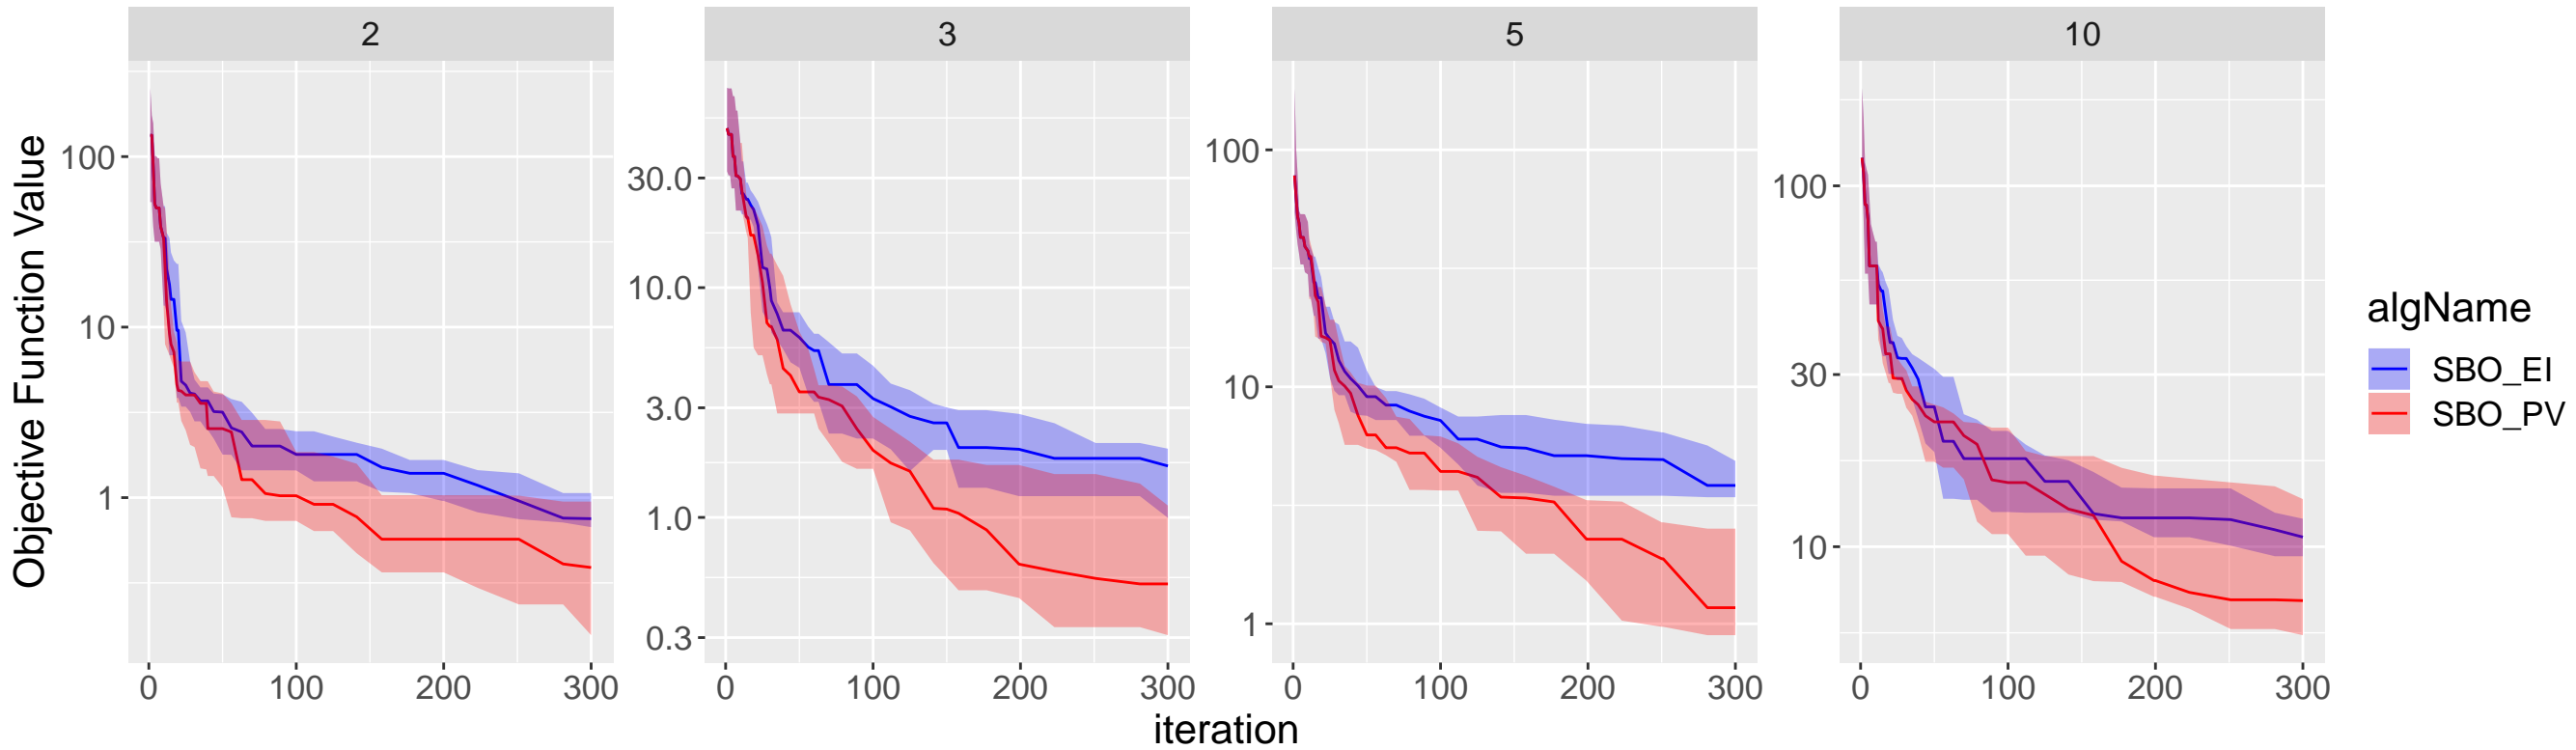

# Griwank–Rosenbrock

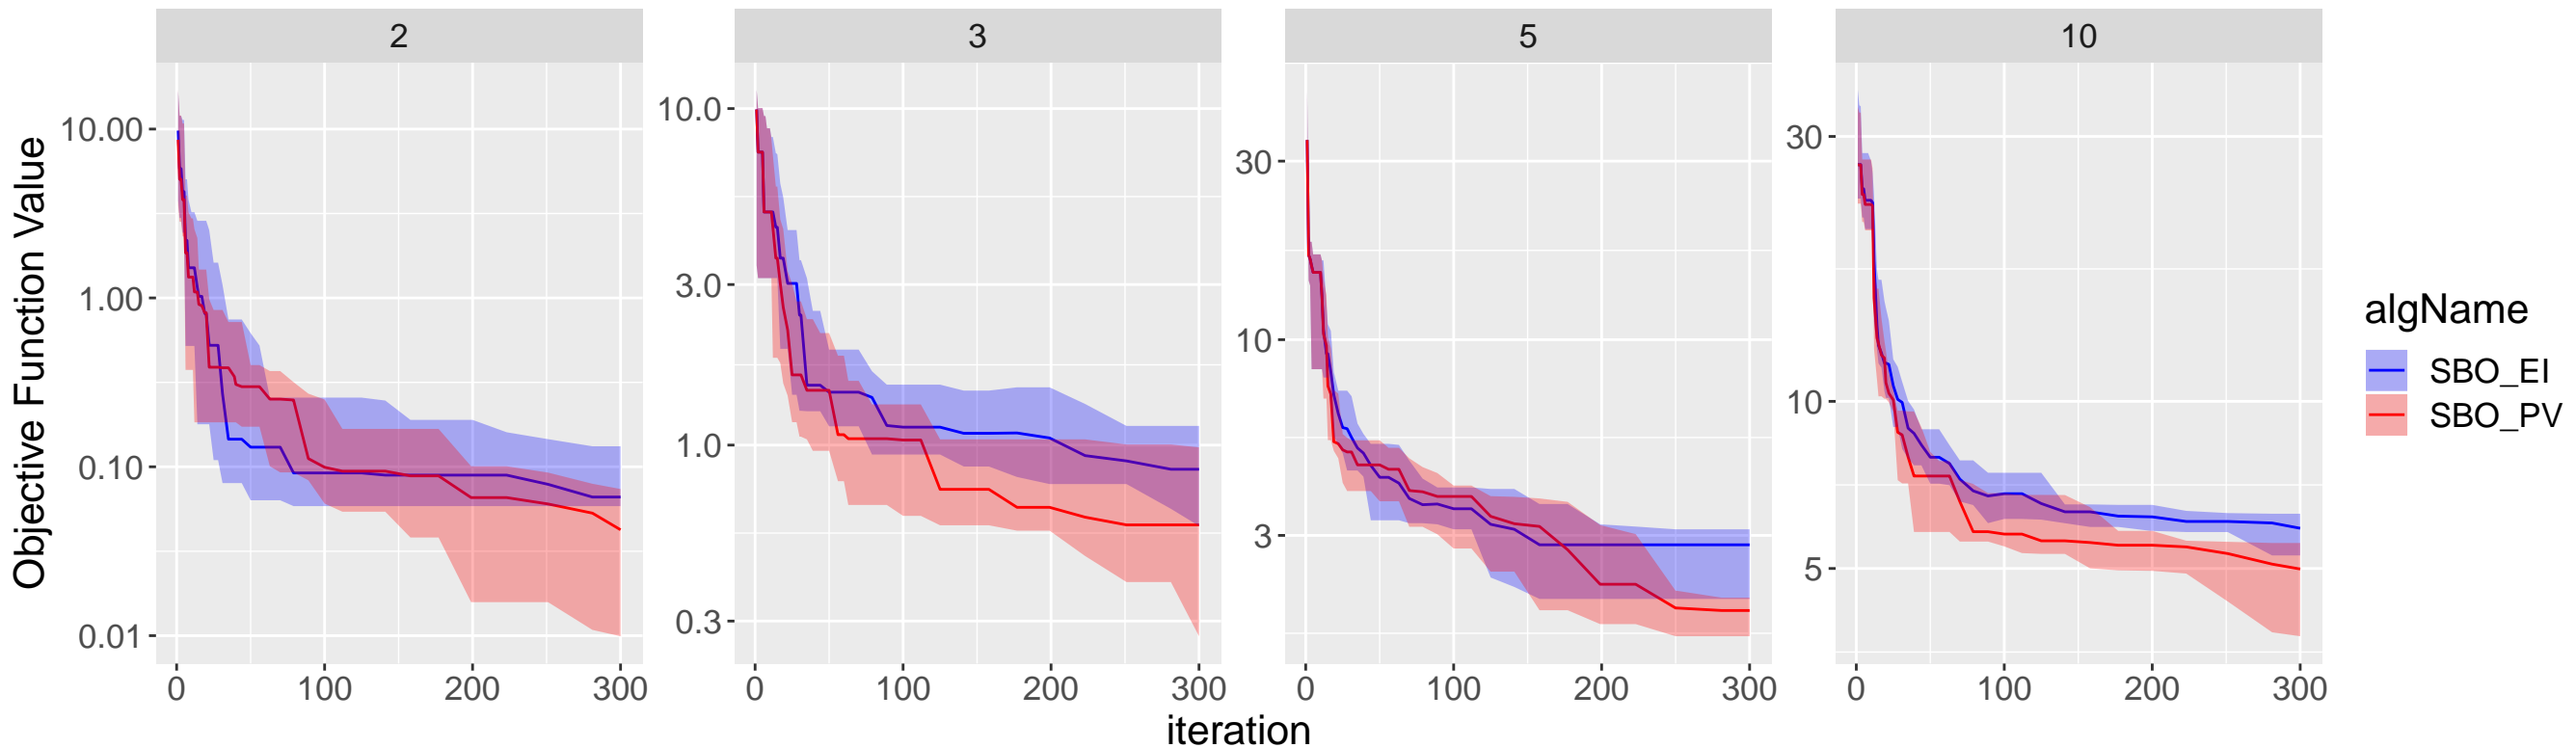

# Schwefel

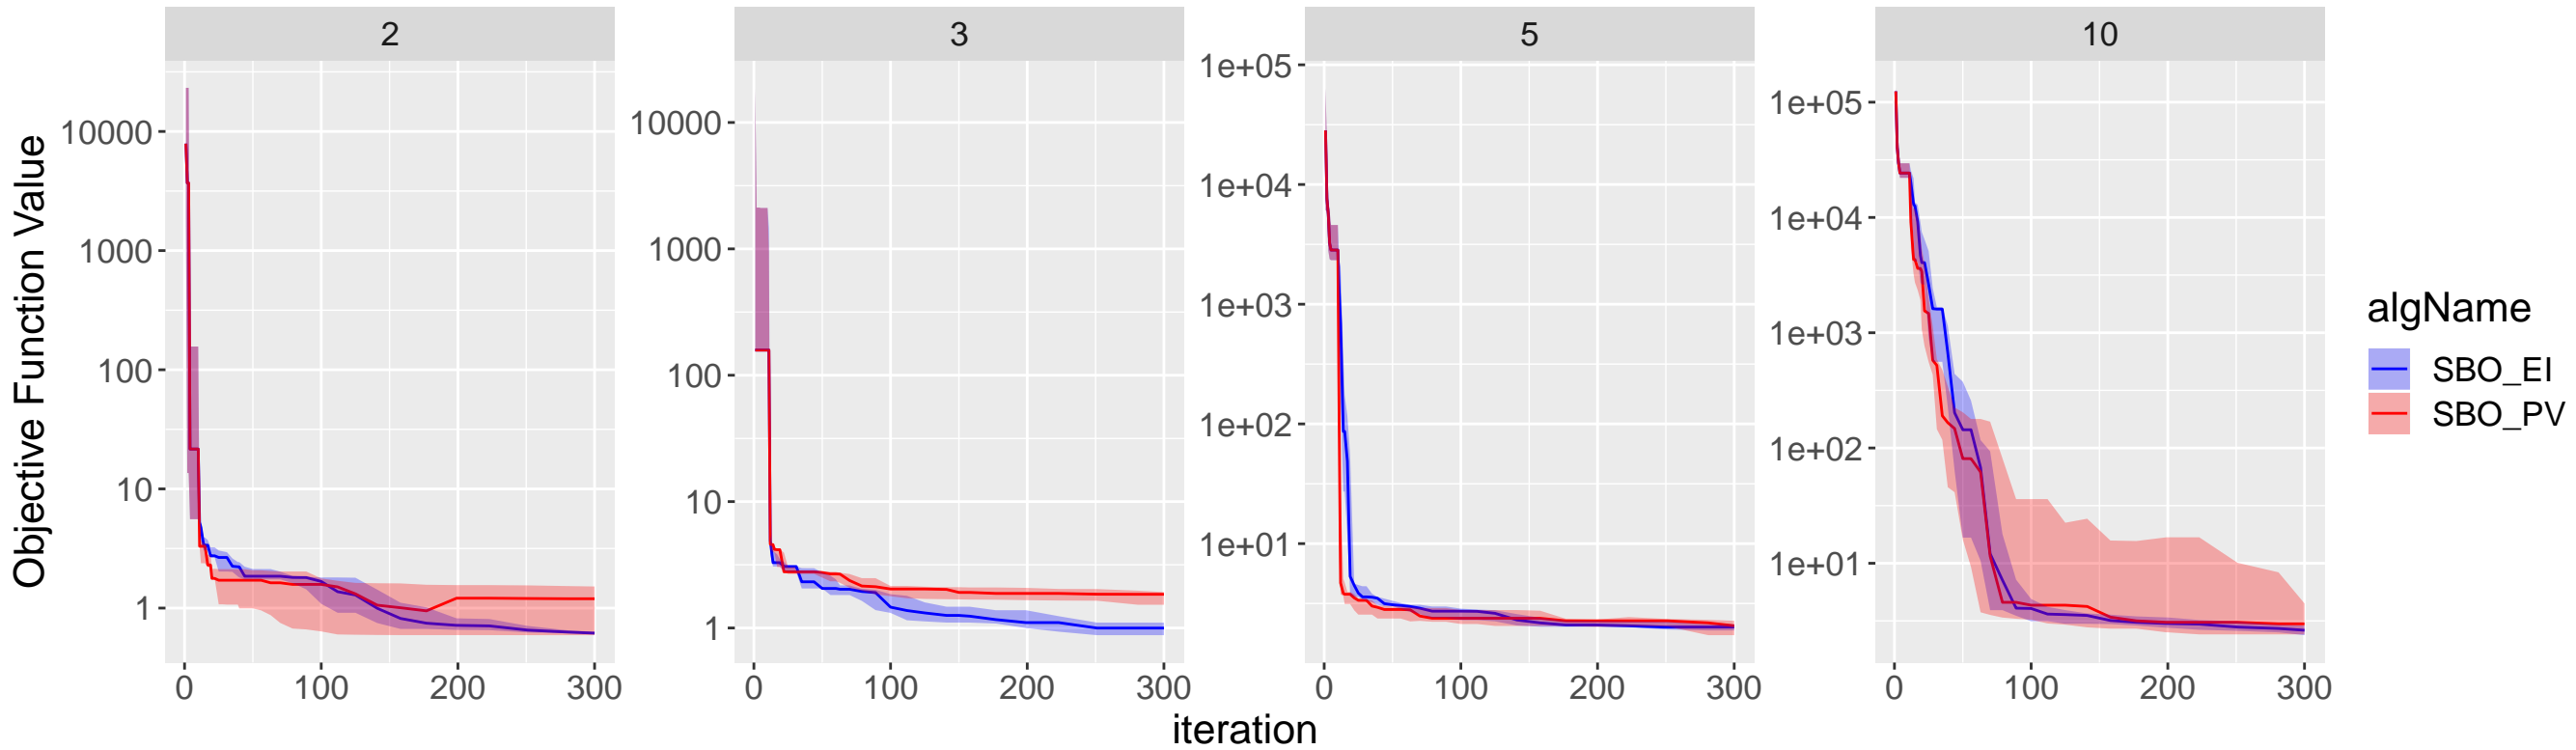

# Gallagher Gaussian 101-me Peaks

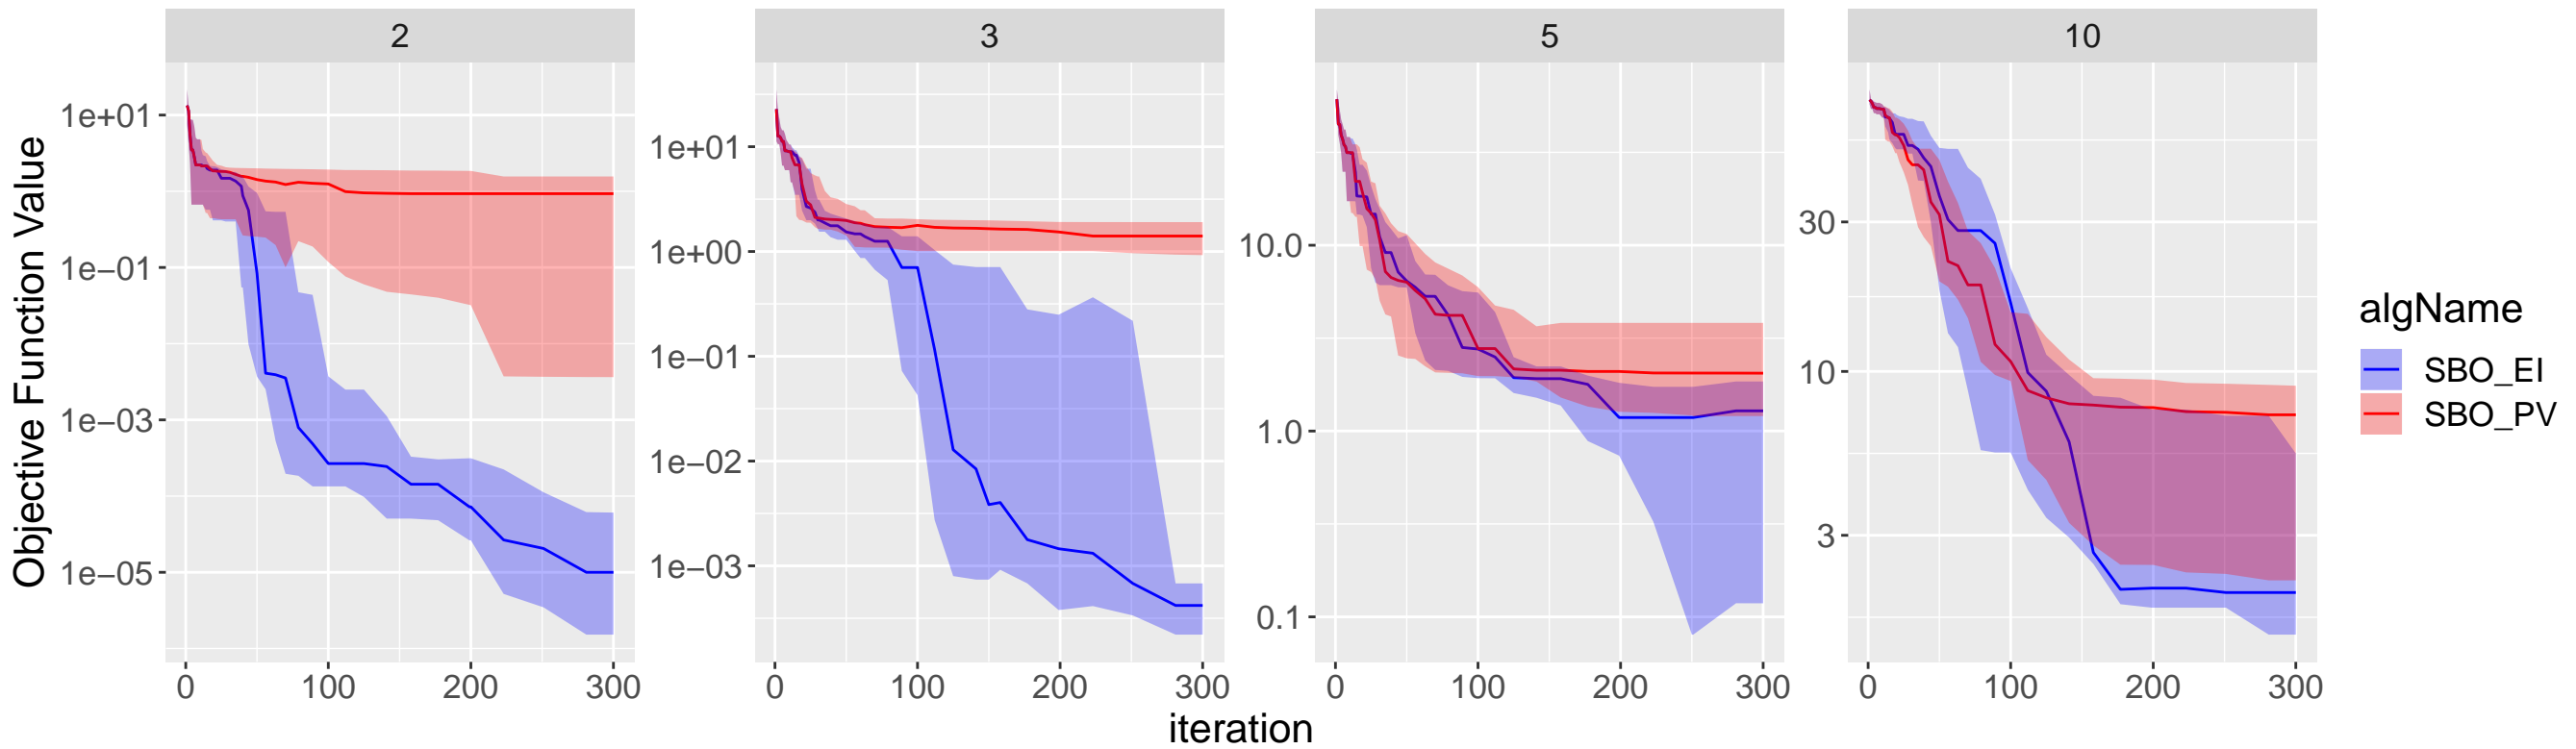

# Gallagher Gaussian 21-hi Peaks

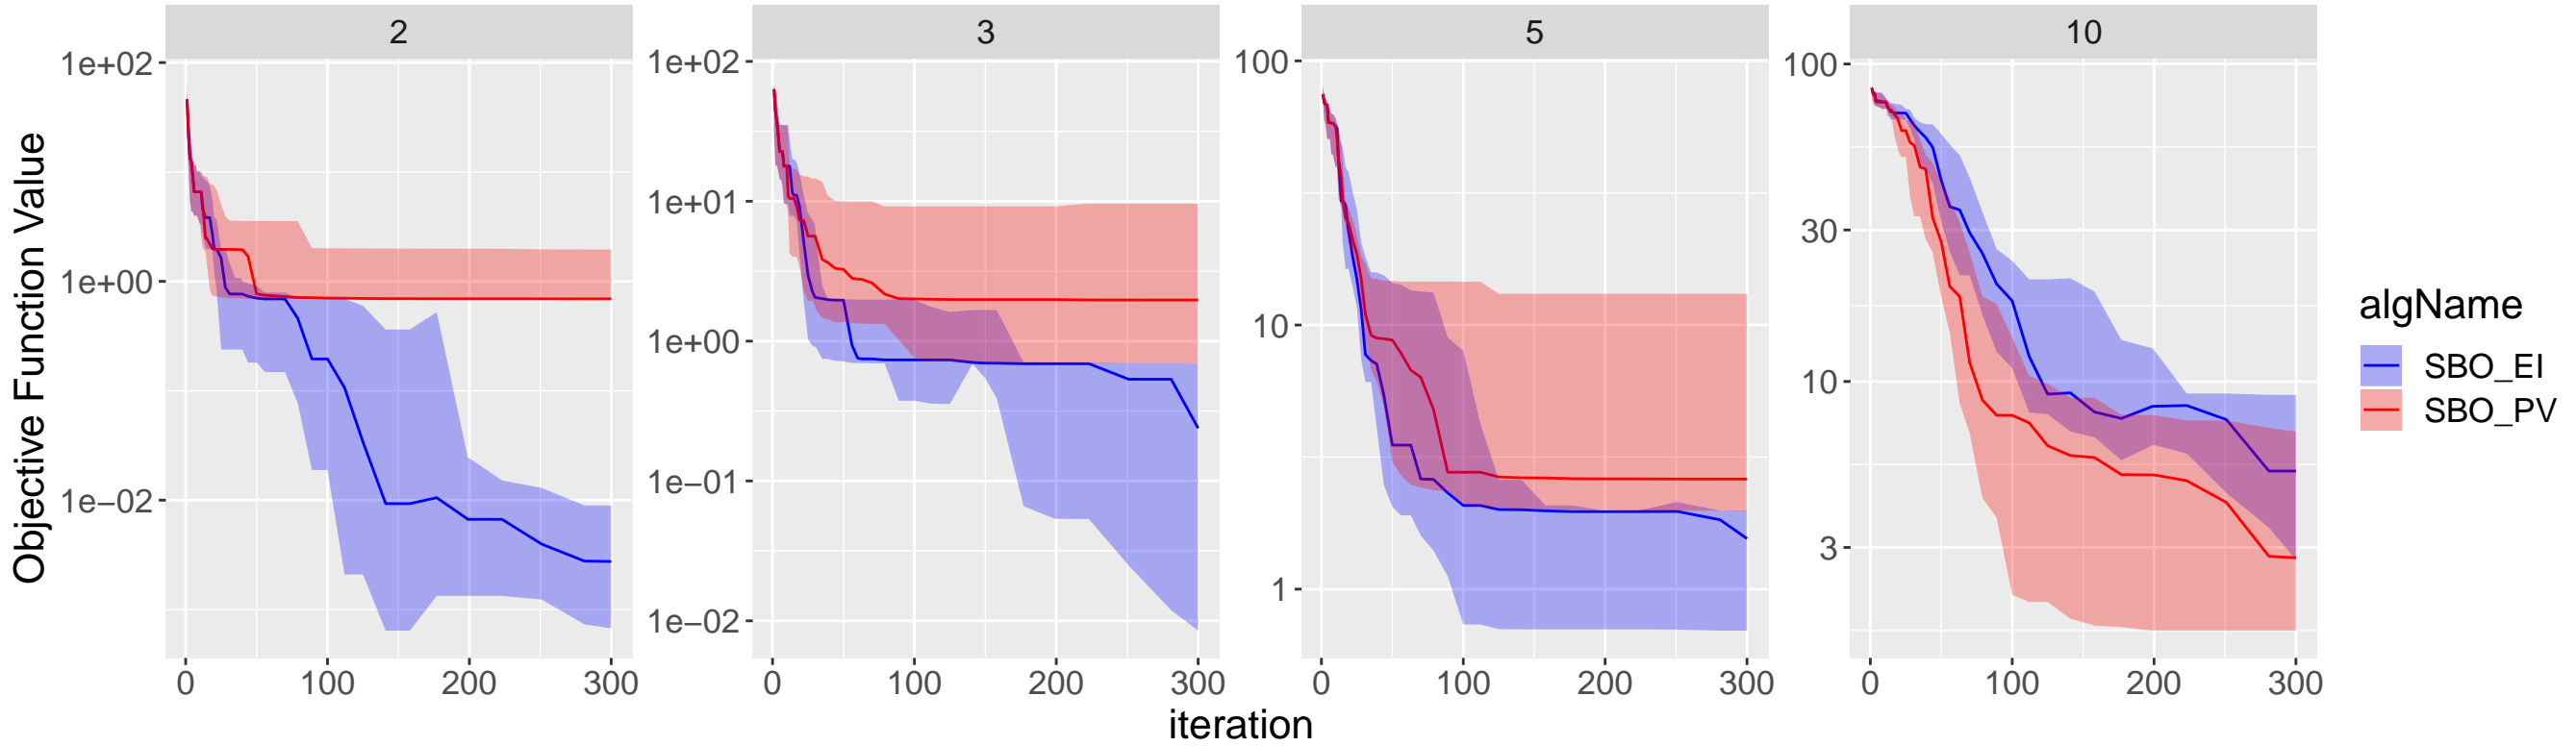

# Katsuura

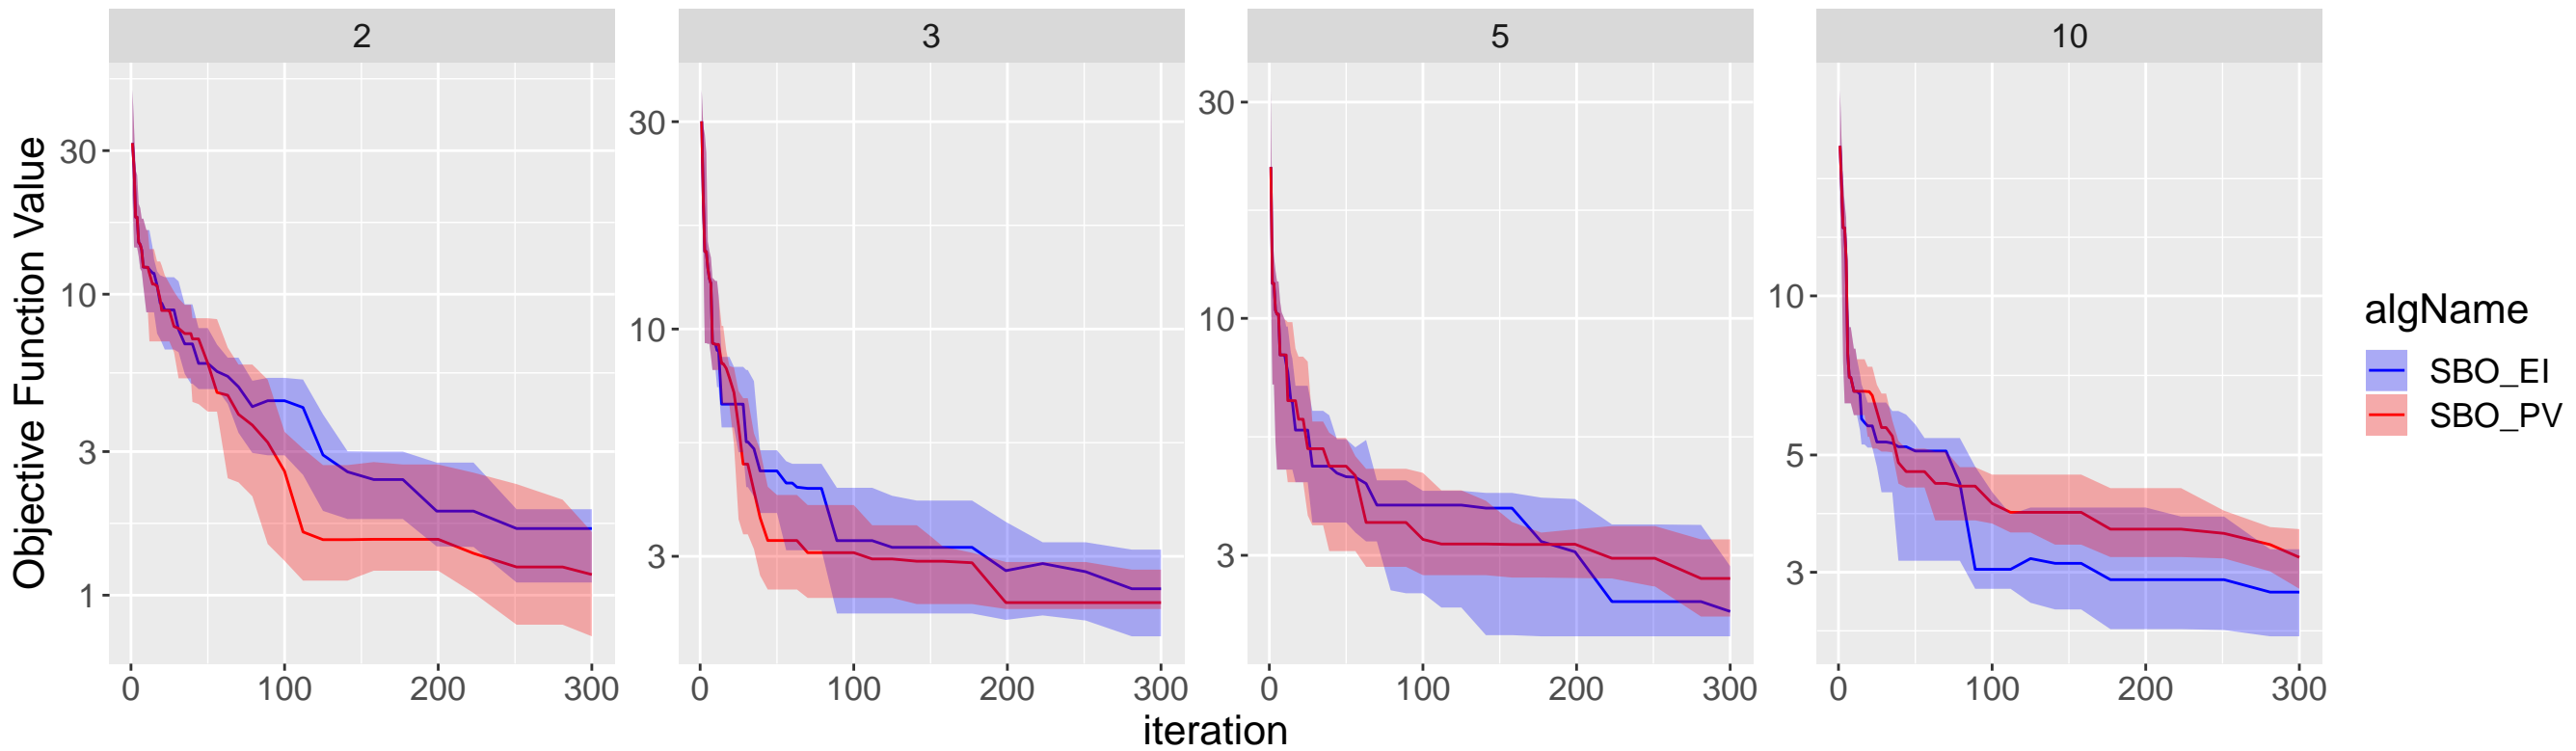

# Lunacek bi-Rastrigin

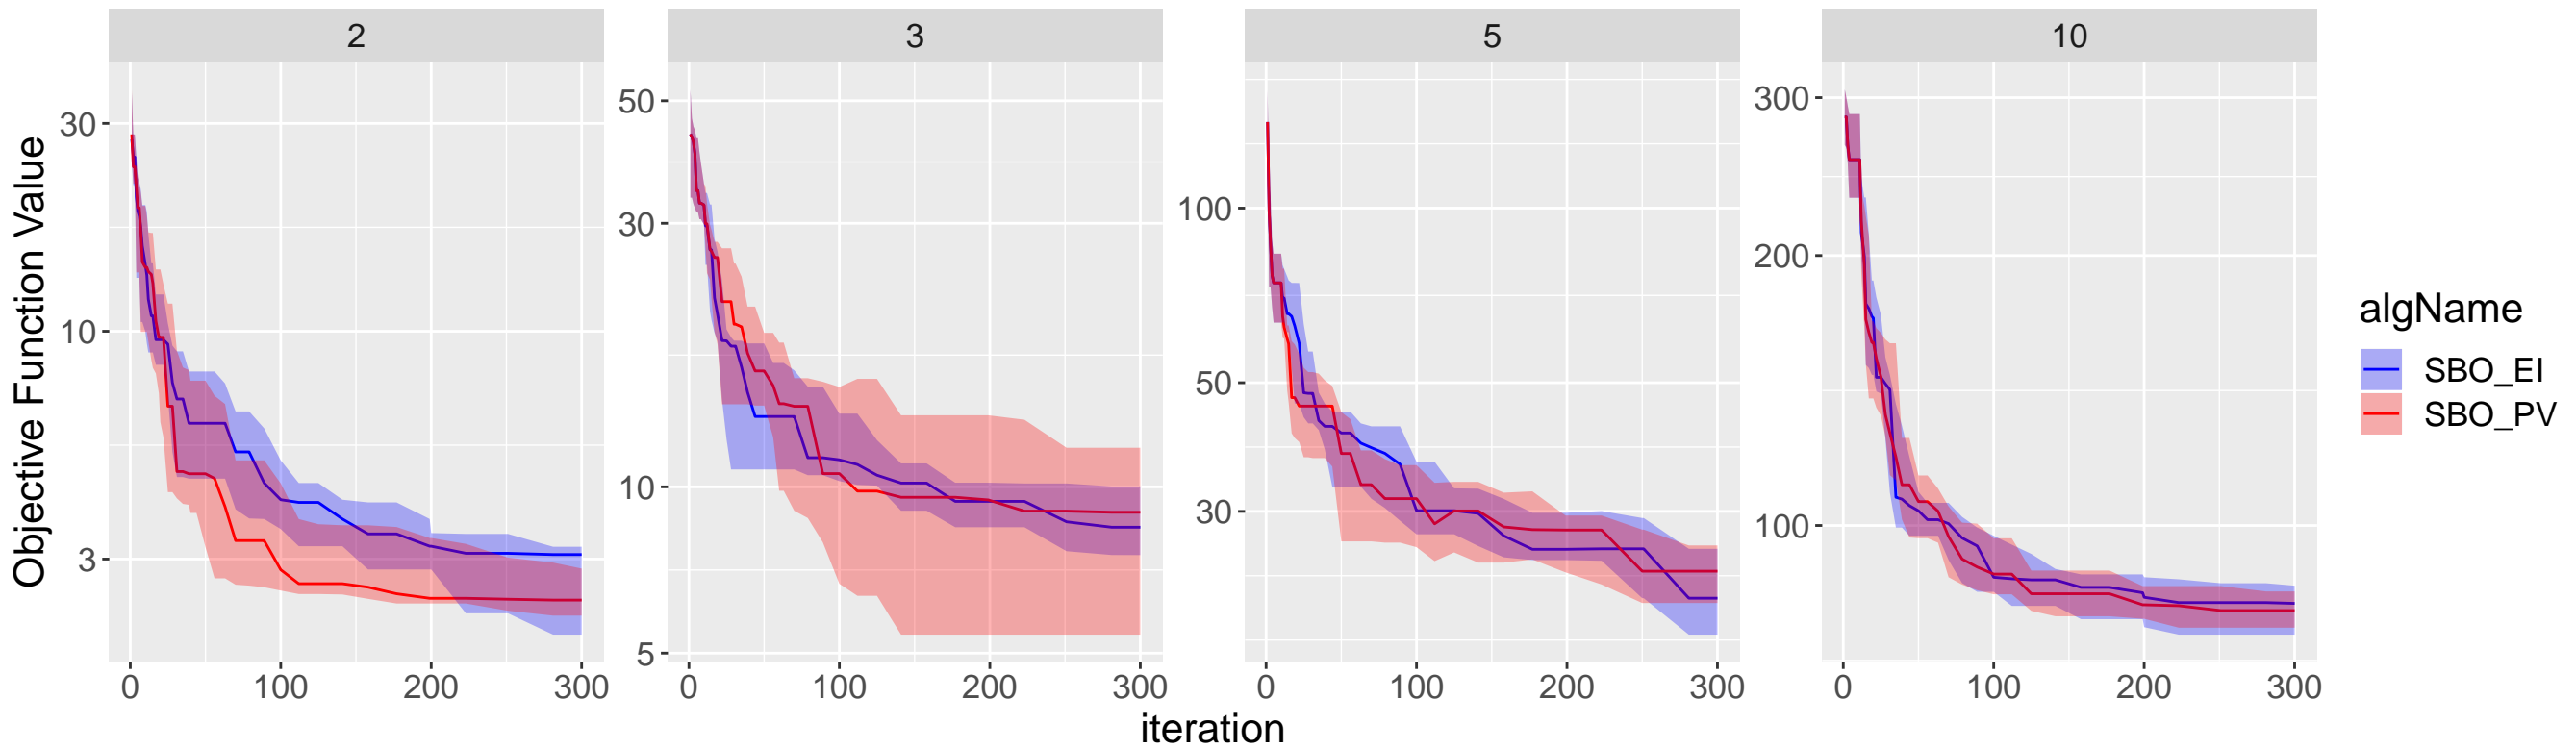

Supplement: Supplementary file 1 [file convergenceMlrOnBBOB.pdf]
