# Supplementary material for: Expected Improvement versus Predicted Value in Surrogate-Based Optimization
Source: arXiv:2001.02957 ancillary file (2020-02-17)

# Sphere

Objective Function Value

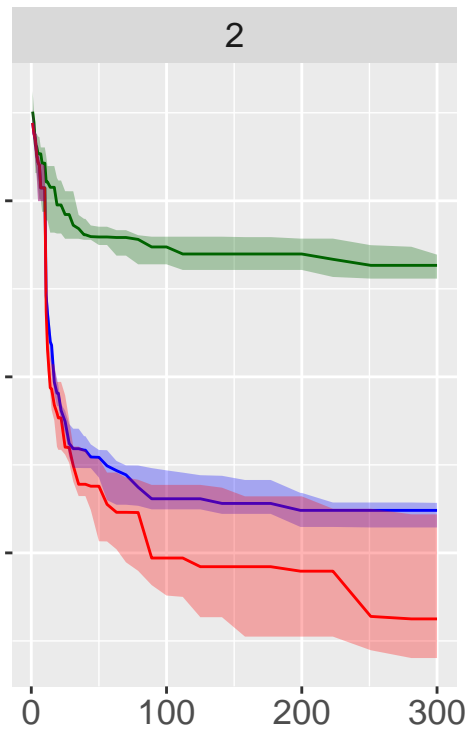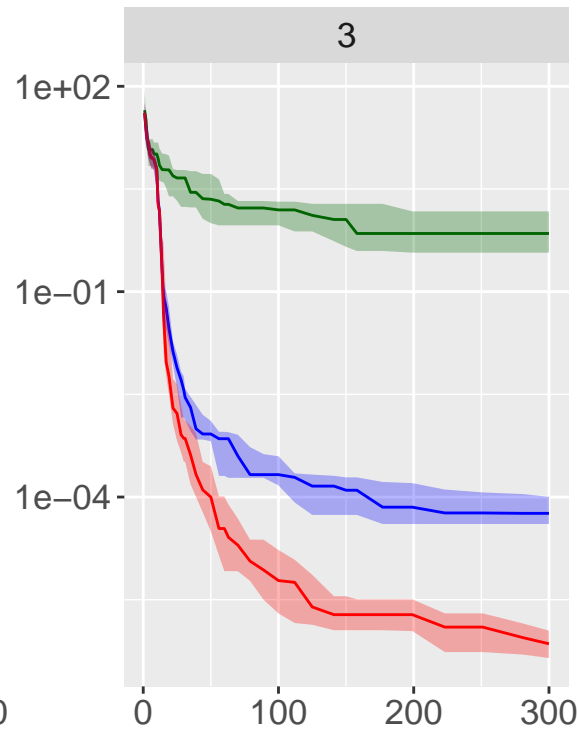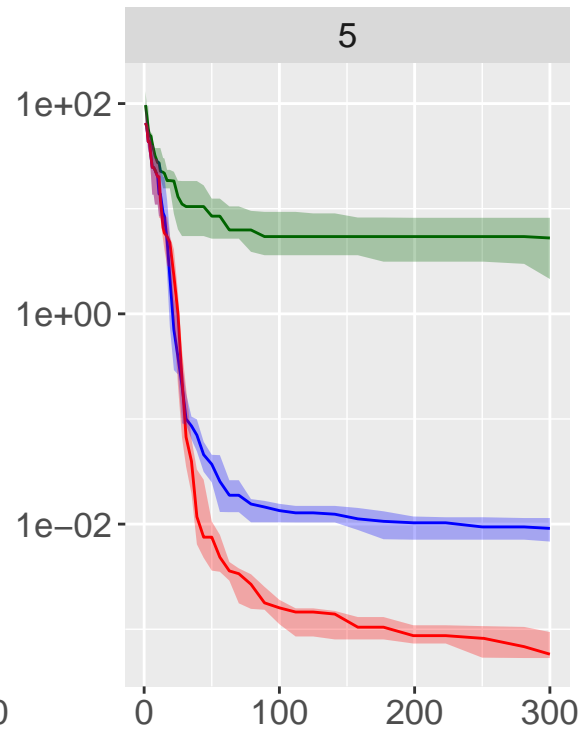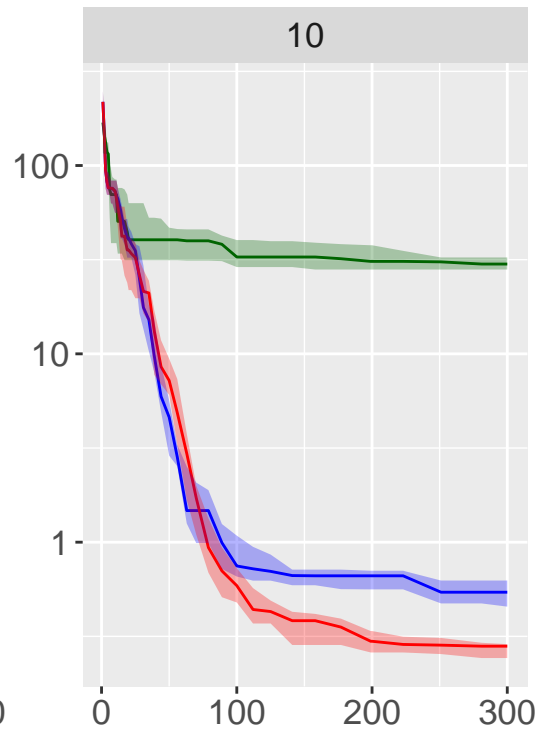

iteration

algName

- RandomSearch\_
- SBO\_EI
- SBO\_PV

# Ellipsoidal

Objective Function Value

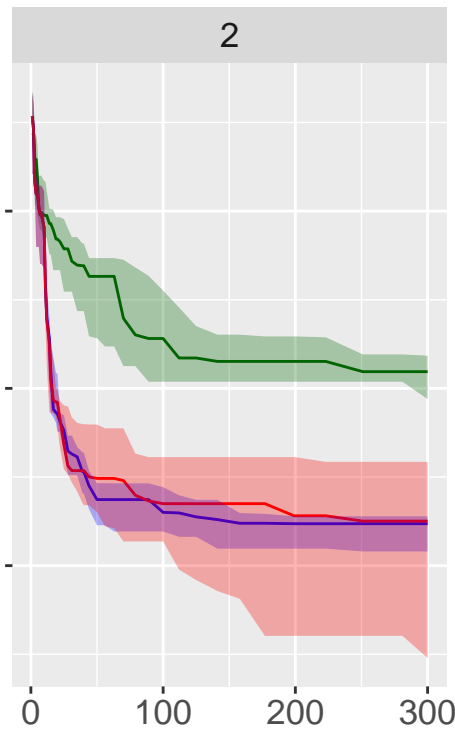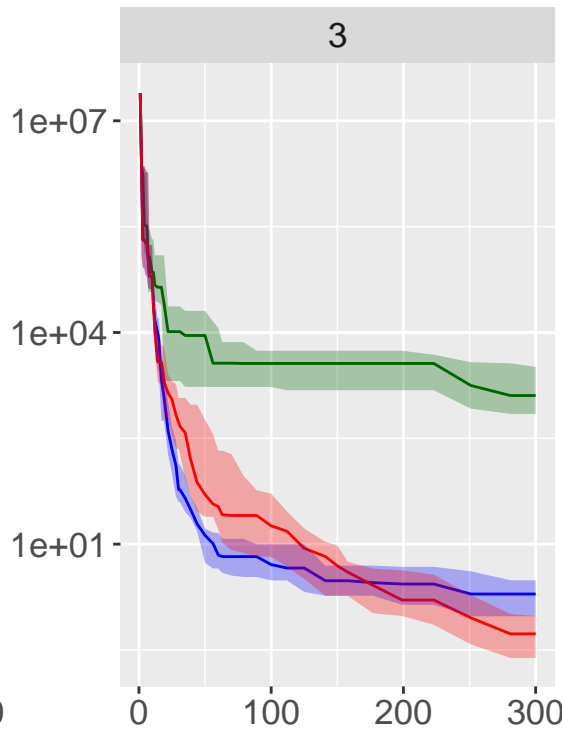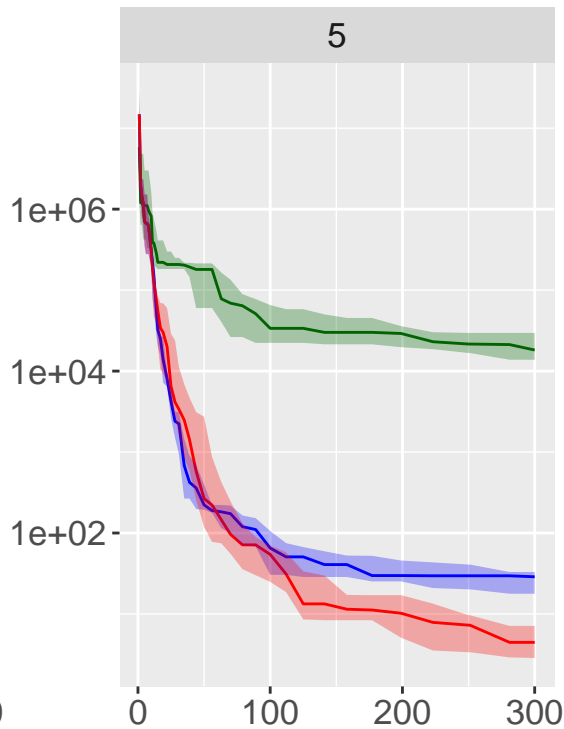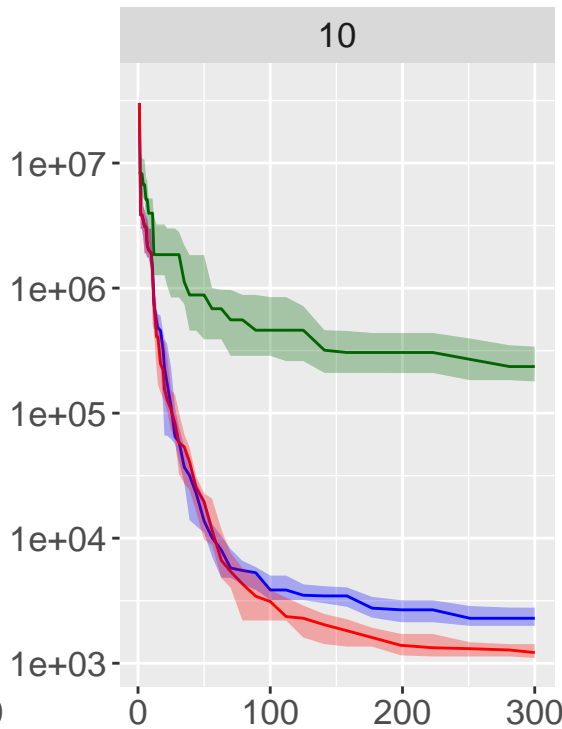

algName

- RandomSearch\_EI
- SBO\_EI
- SBO\_PV

iteration

# Rastrigin

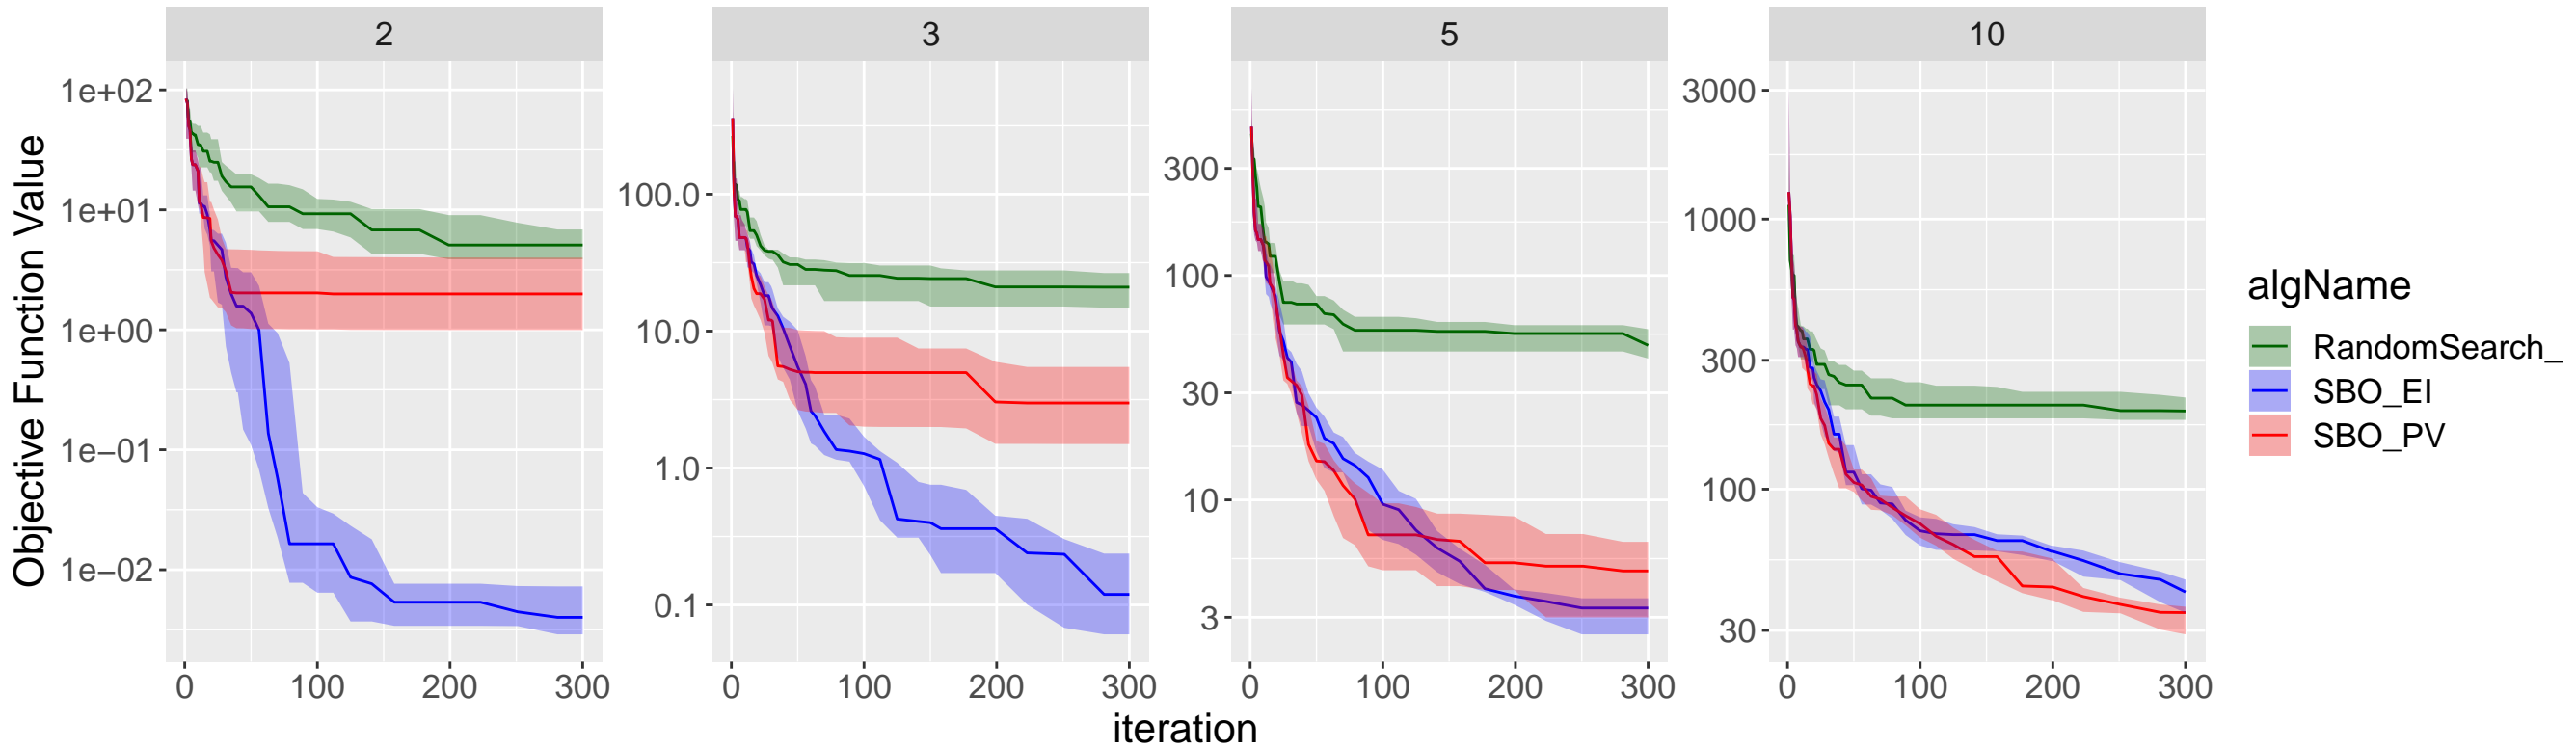

# Büche–Rastrigin

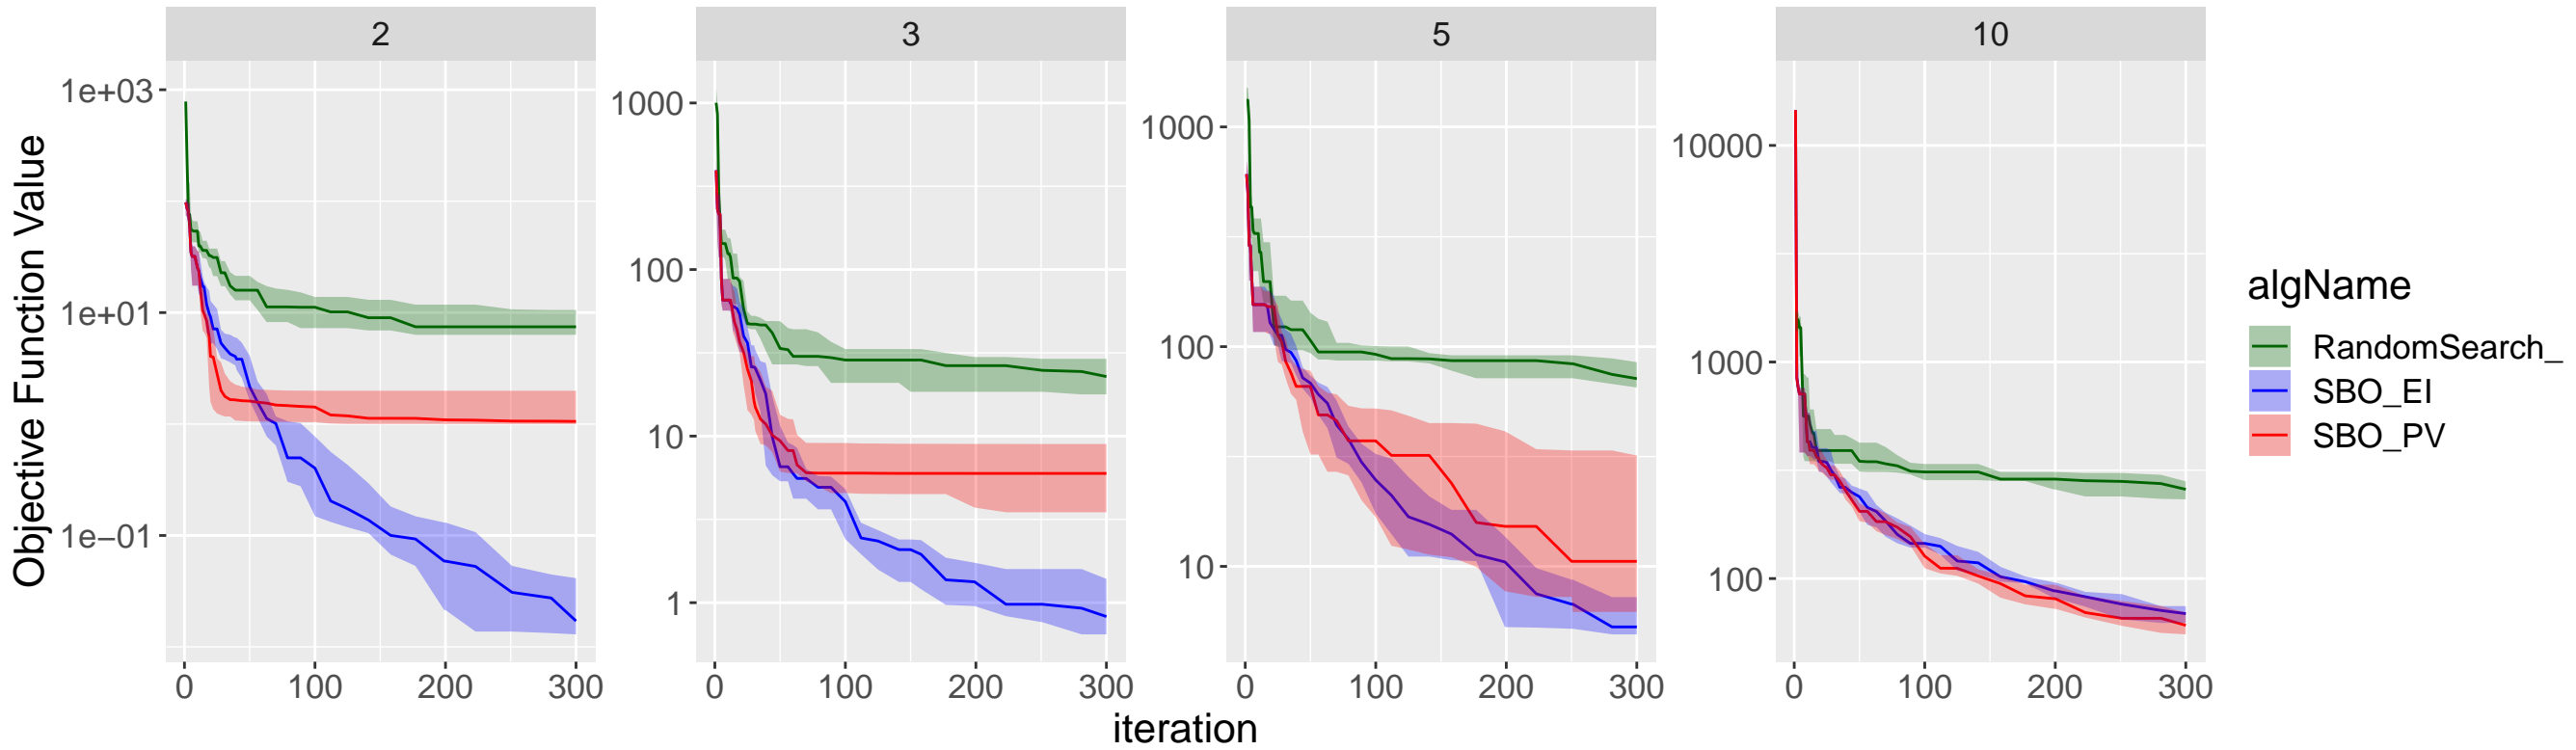

# Linear Slope

Objective Function Value

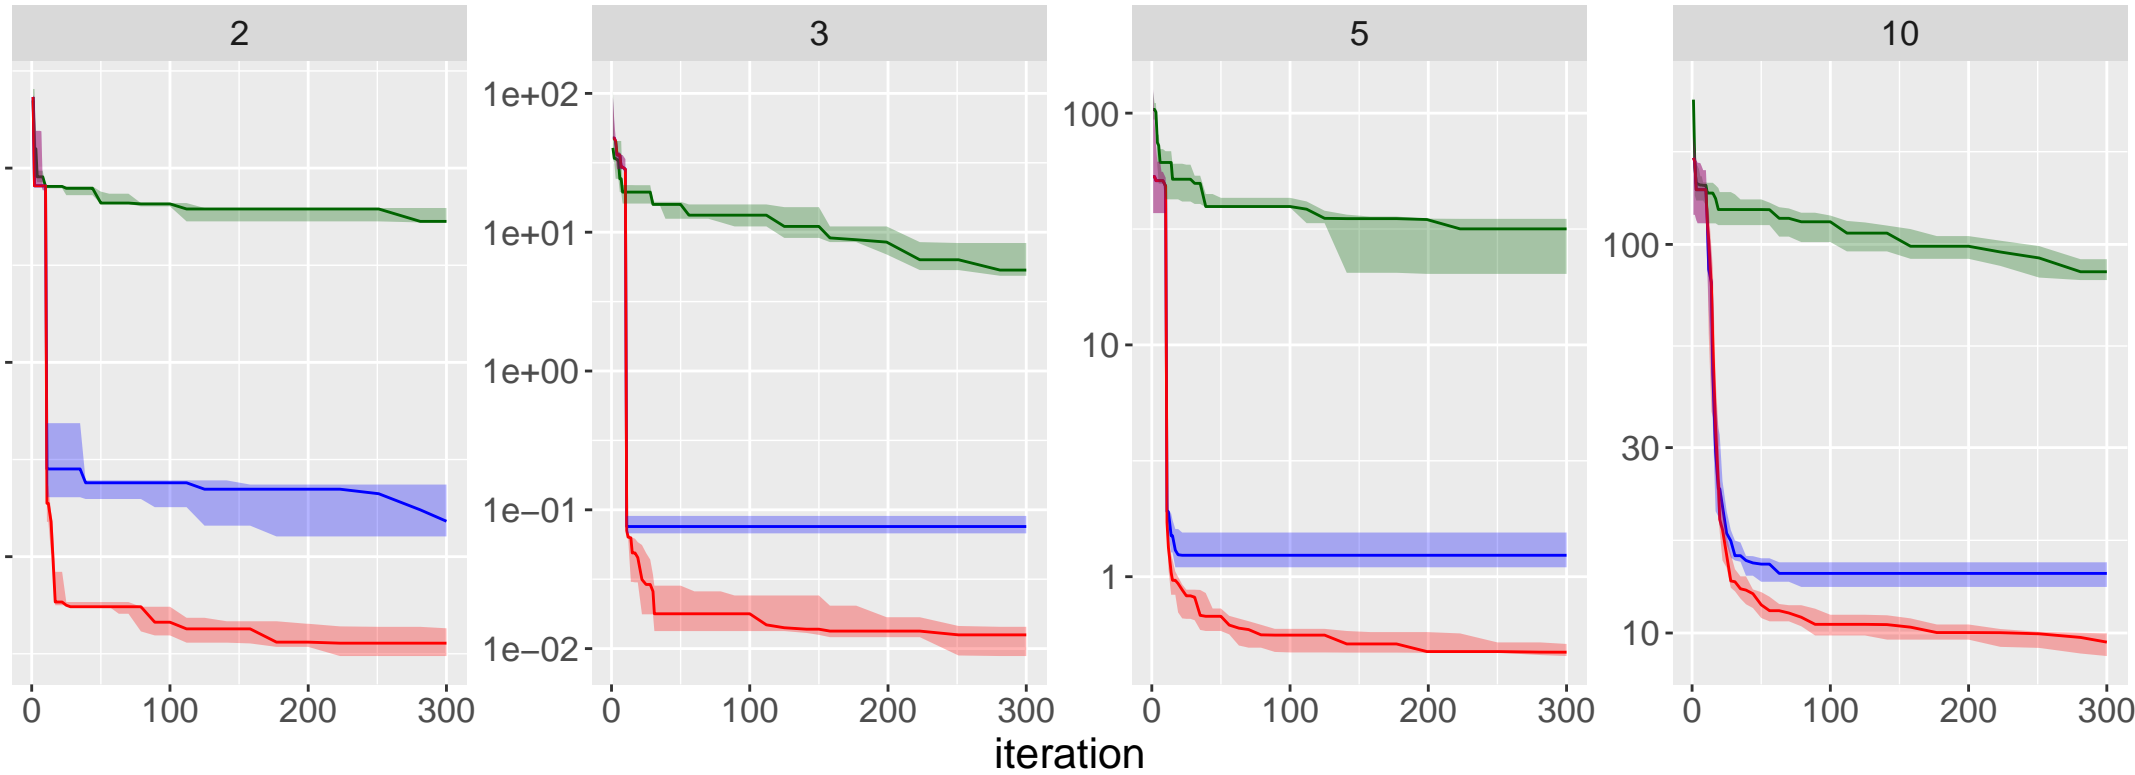

Attractive Sector

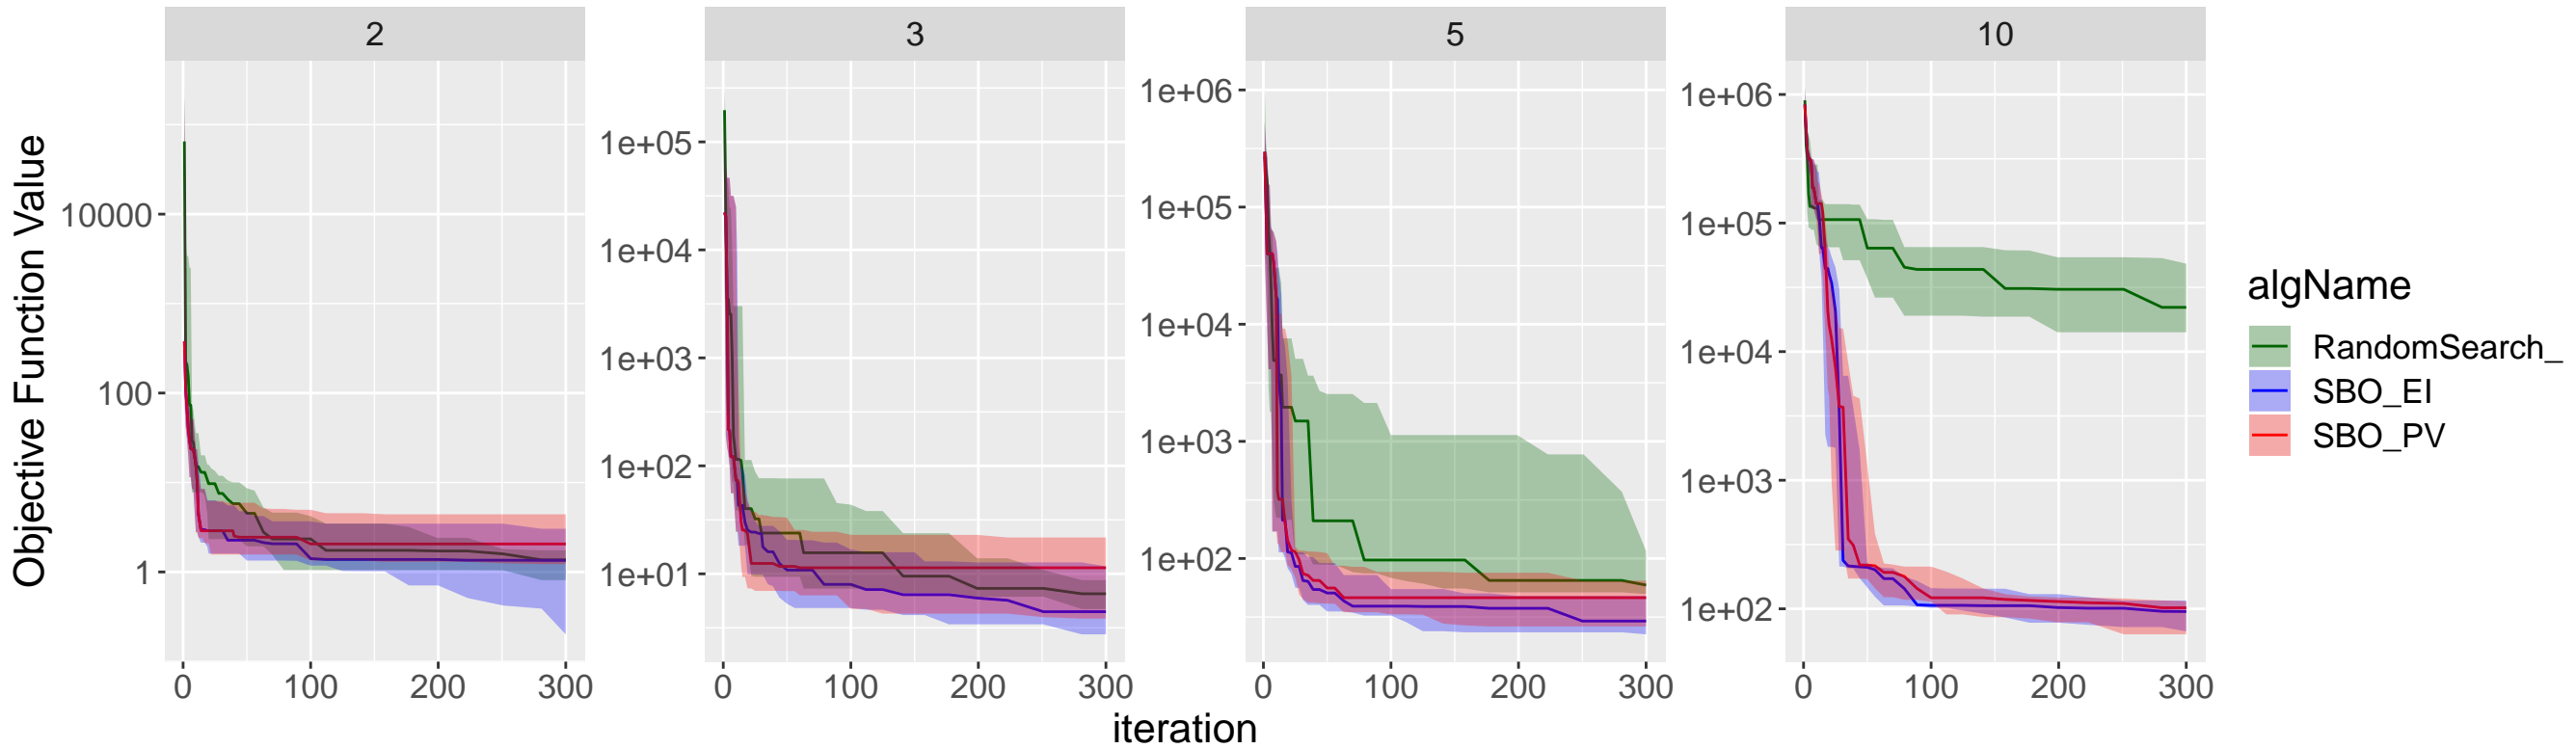

# Step Ellipsoidal

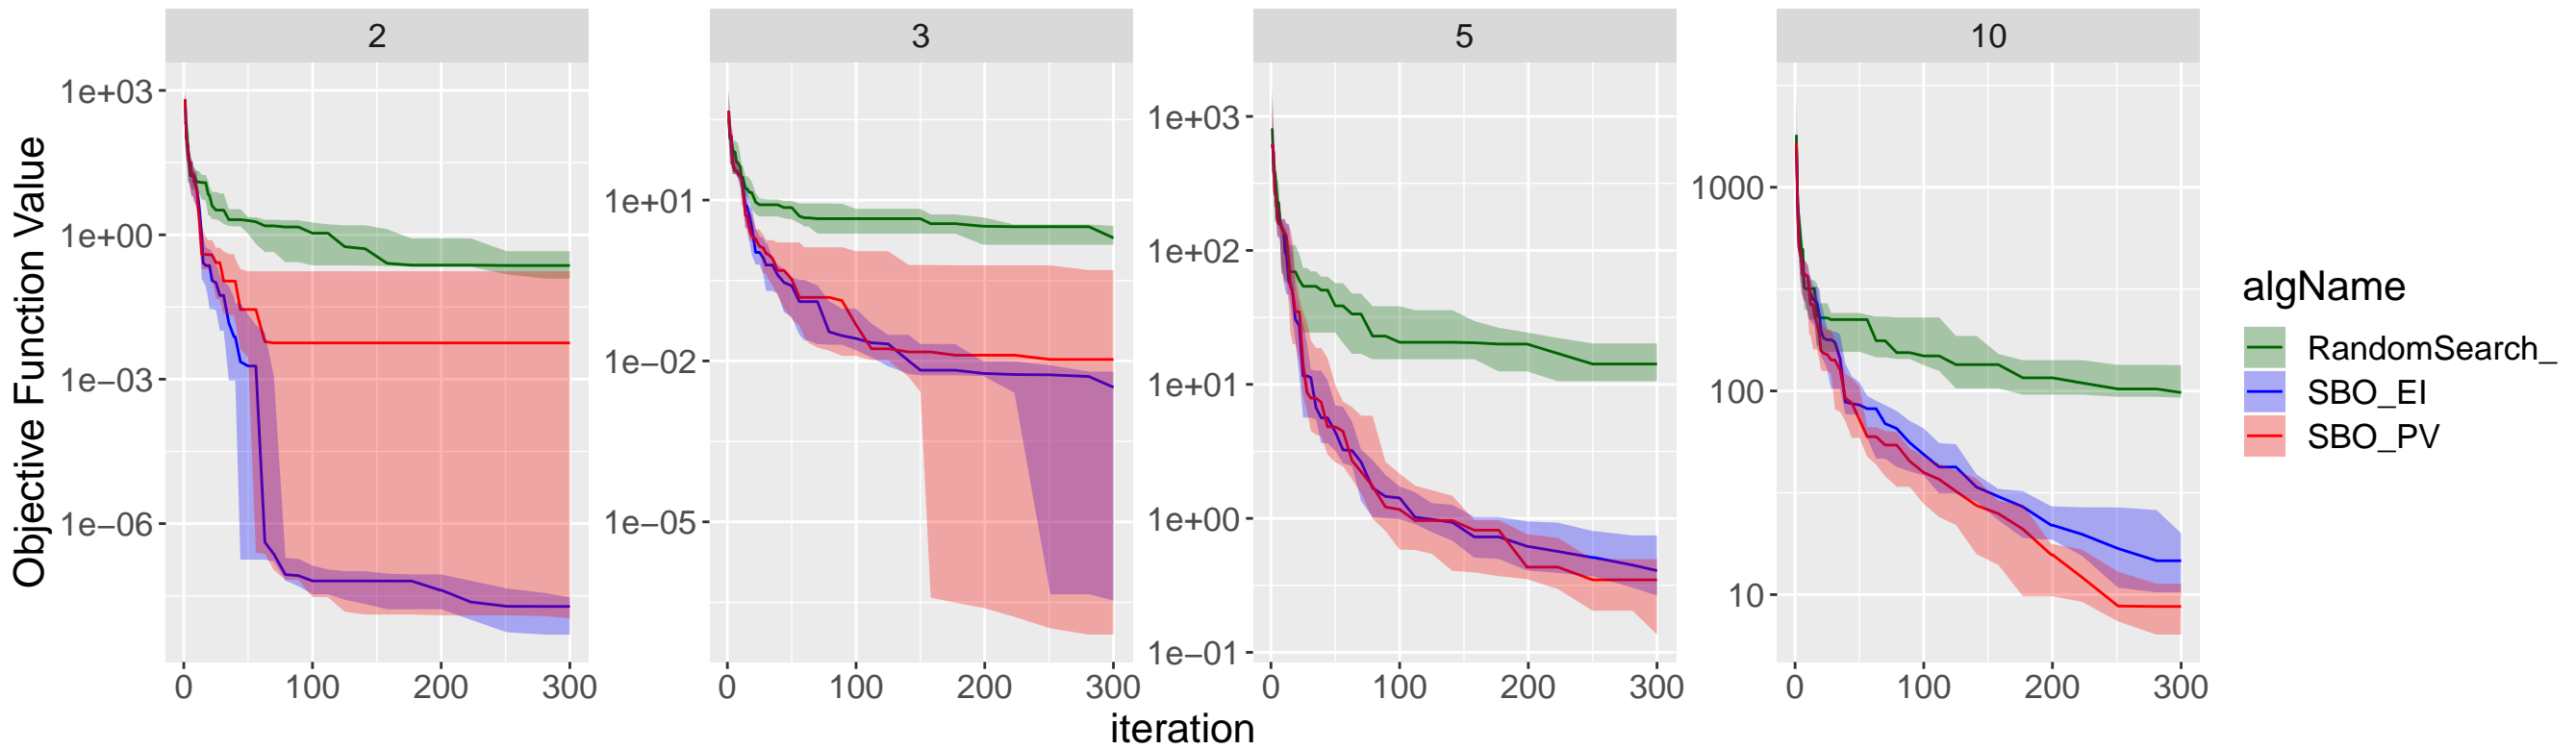

# Rosenbrock

Objective Function Value

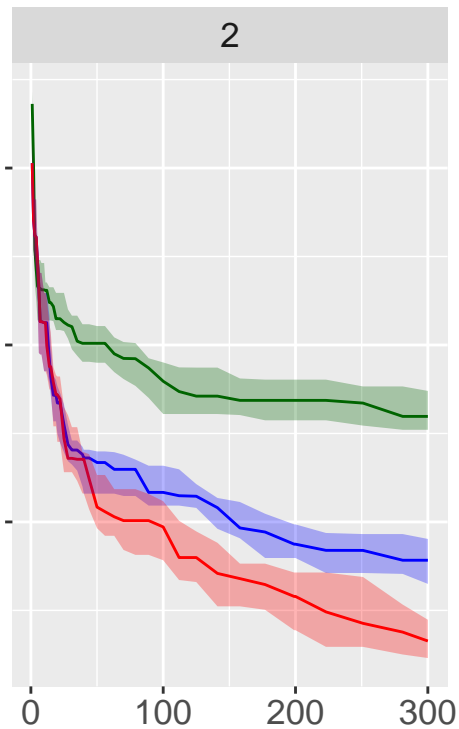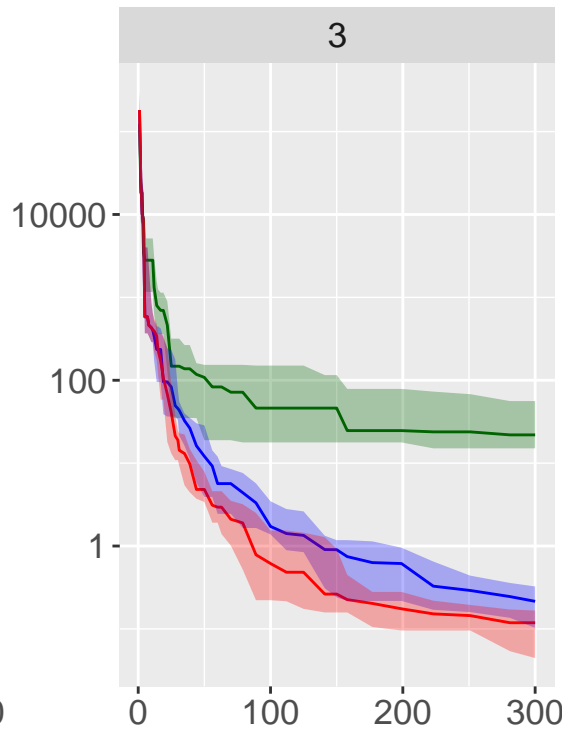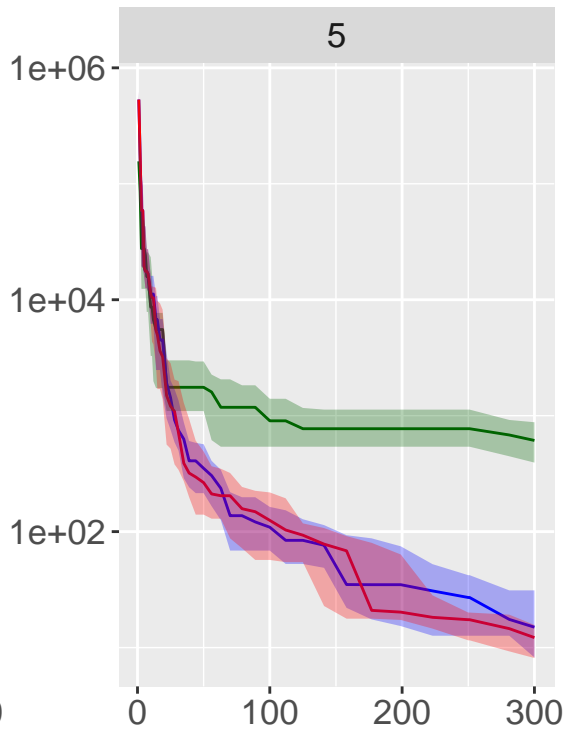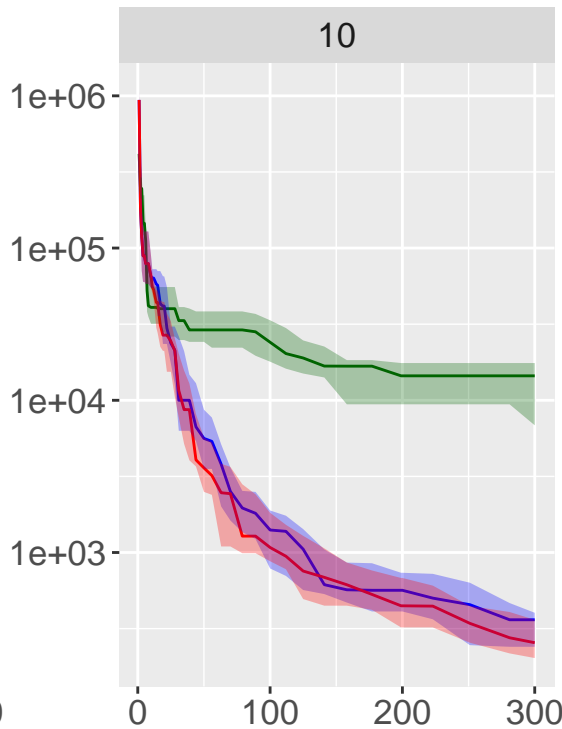

iteration

algName

- RandomSearch\_
- SBO\_EI
- SBO\_PV



# Rosenbrock, rotated

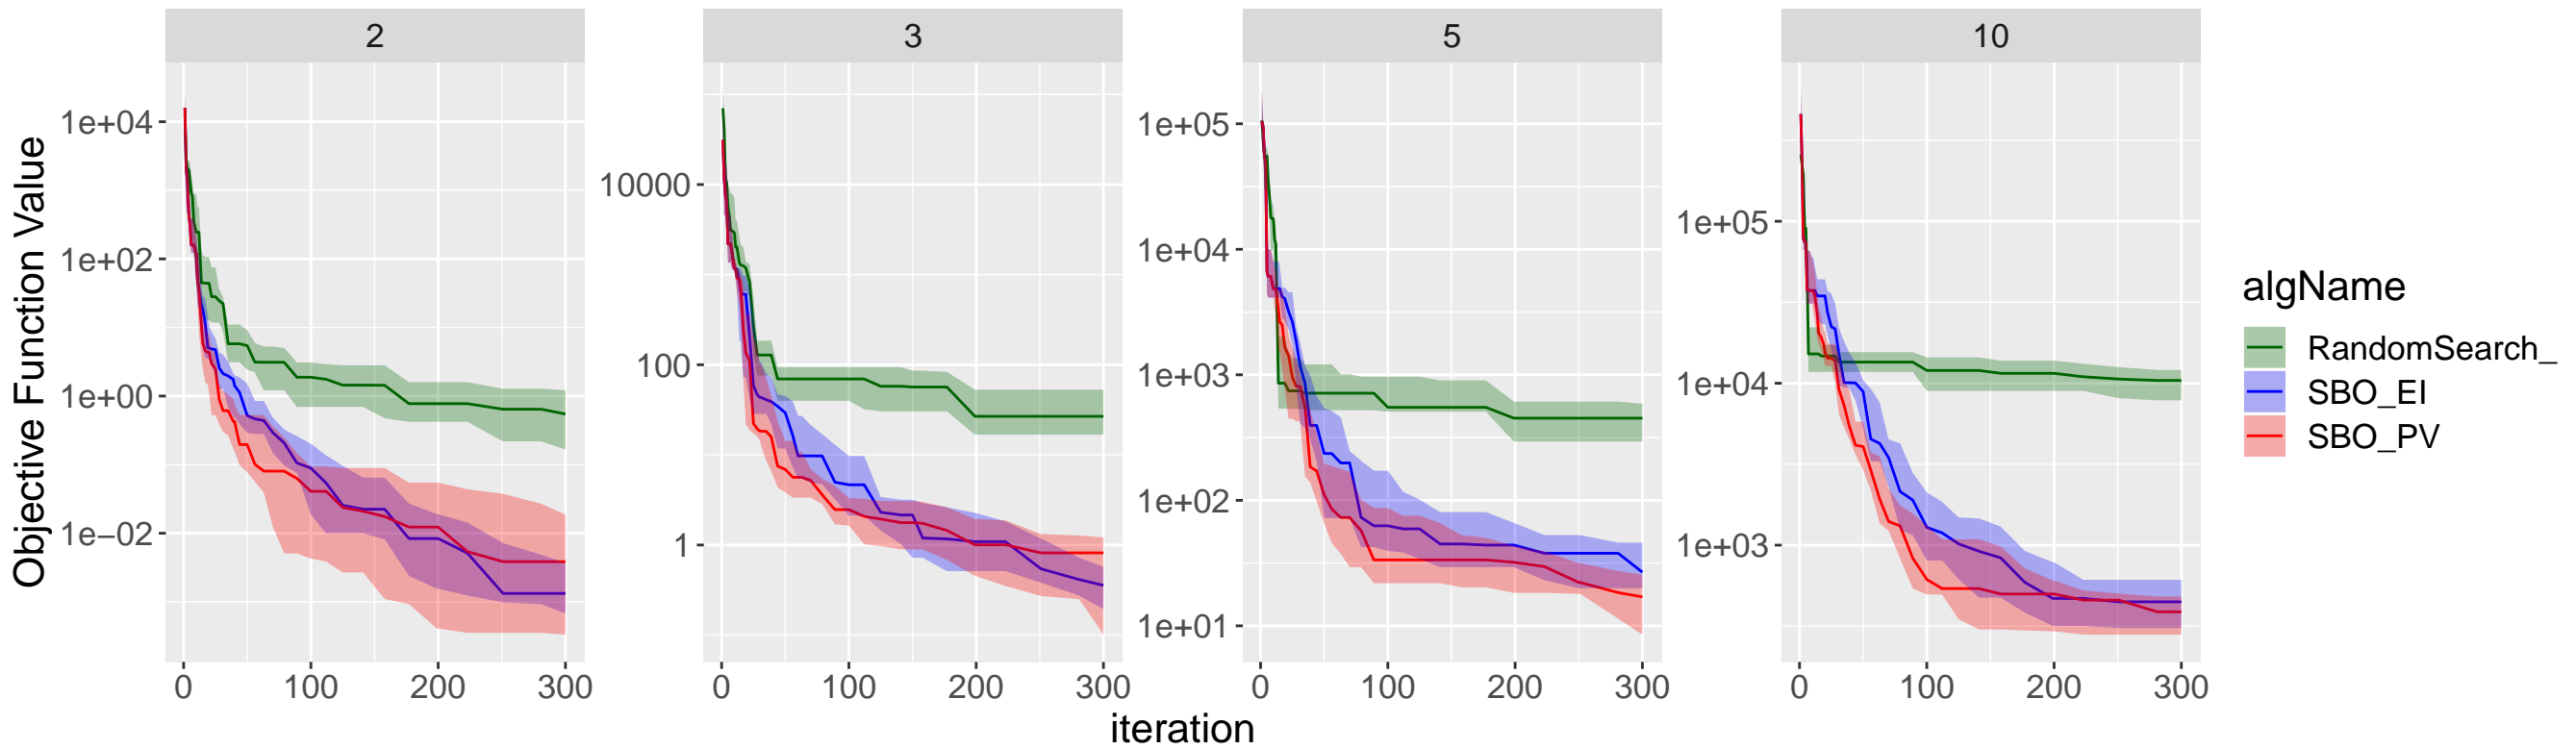

# Ellipsoidal

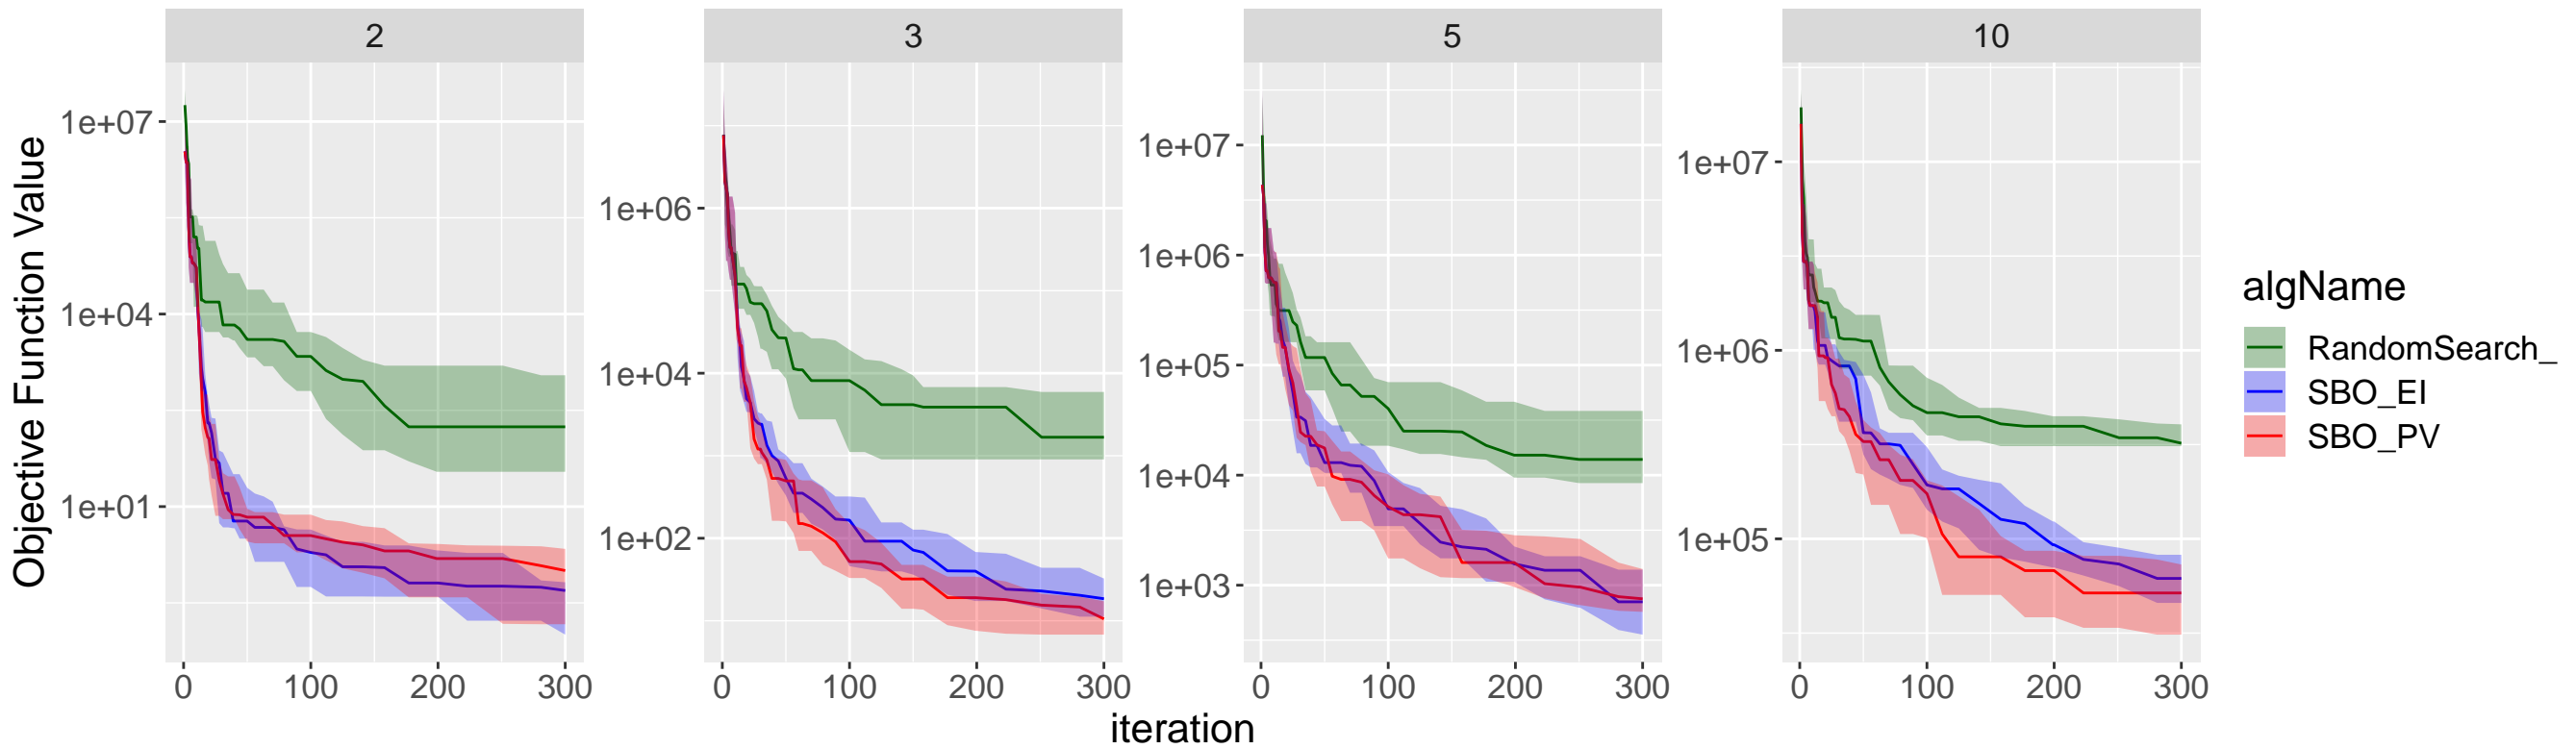

# Discus

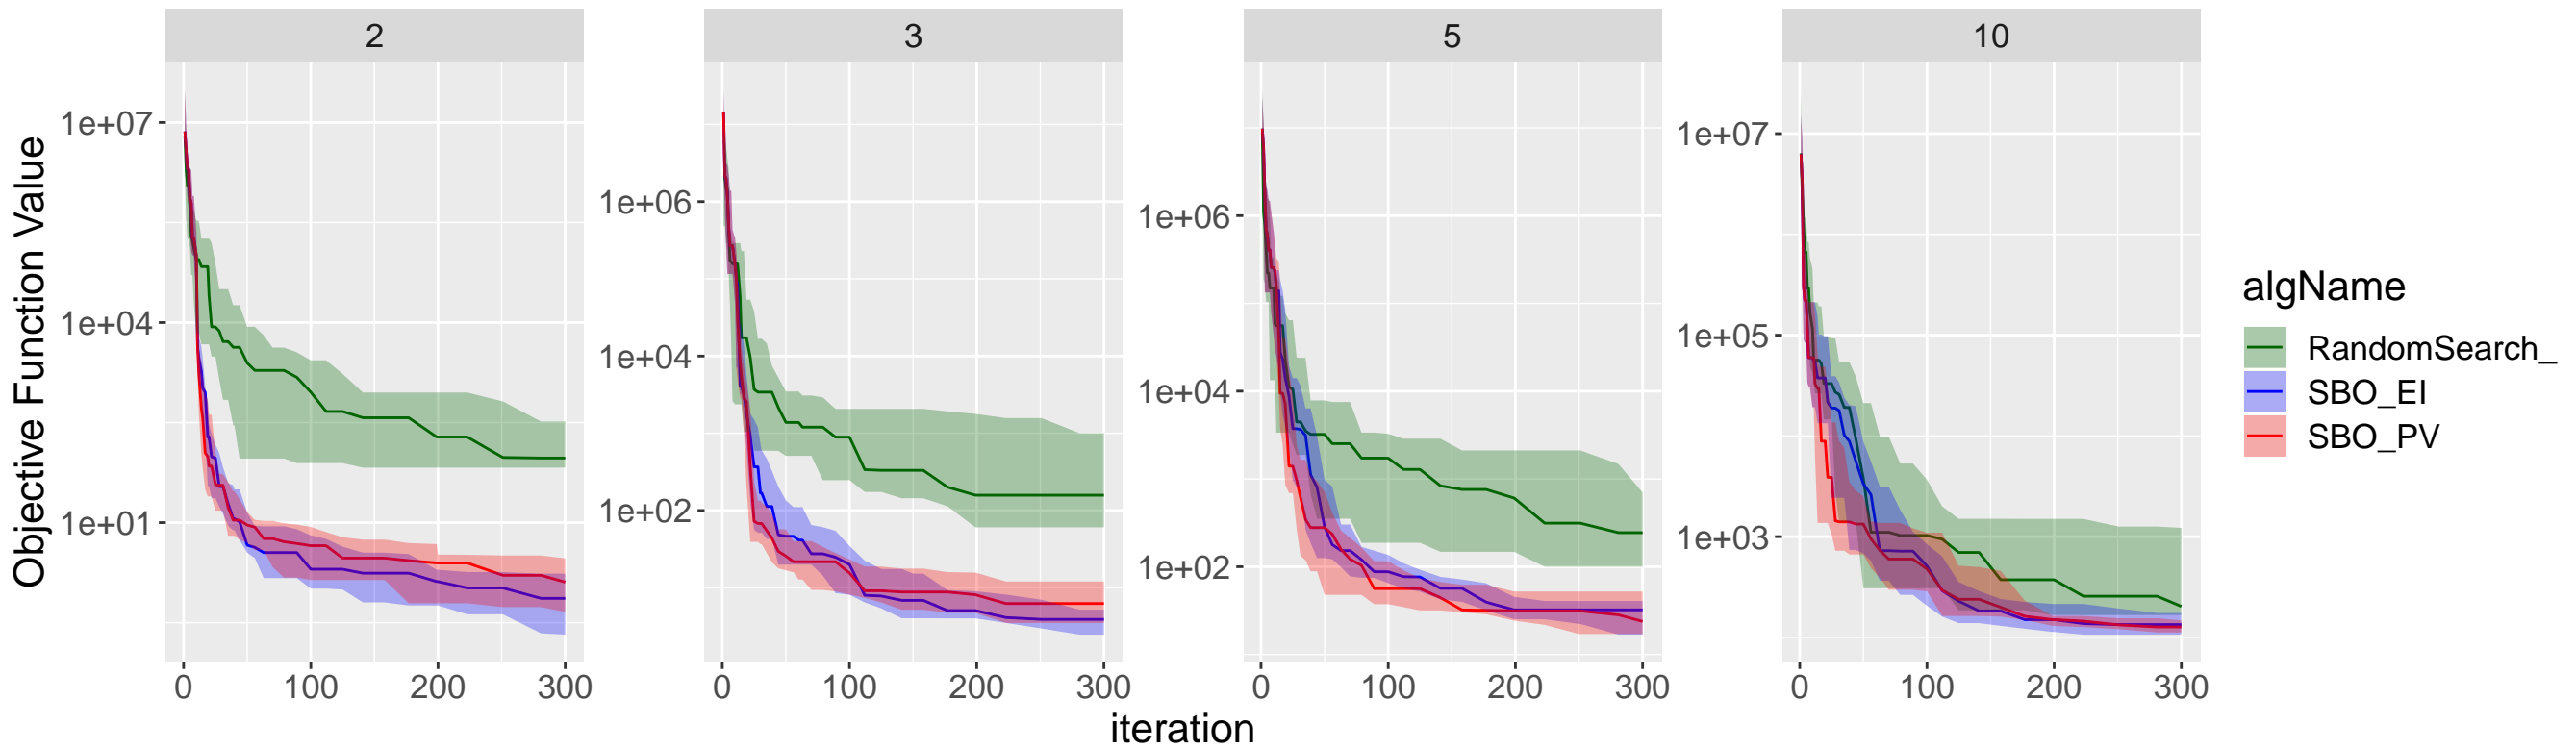

# Bent Cigar

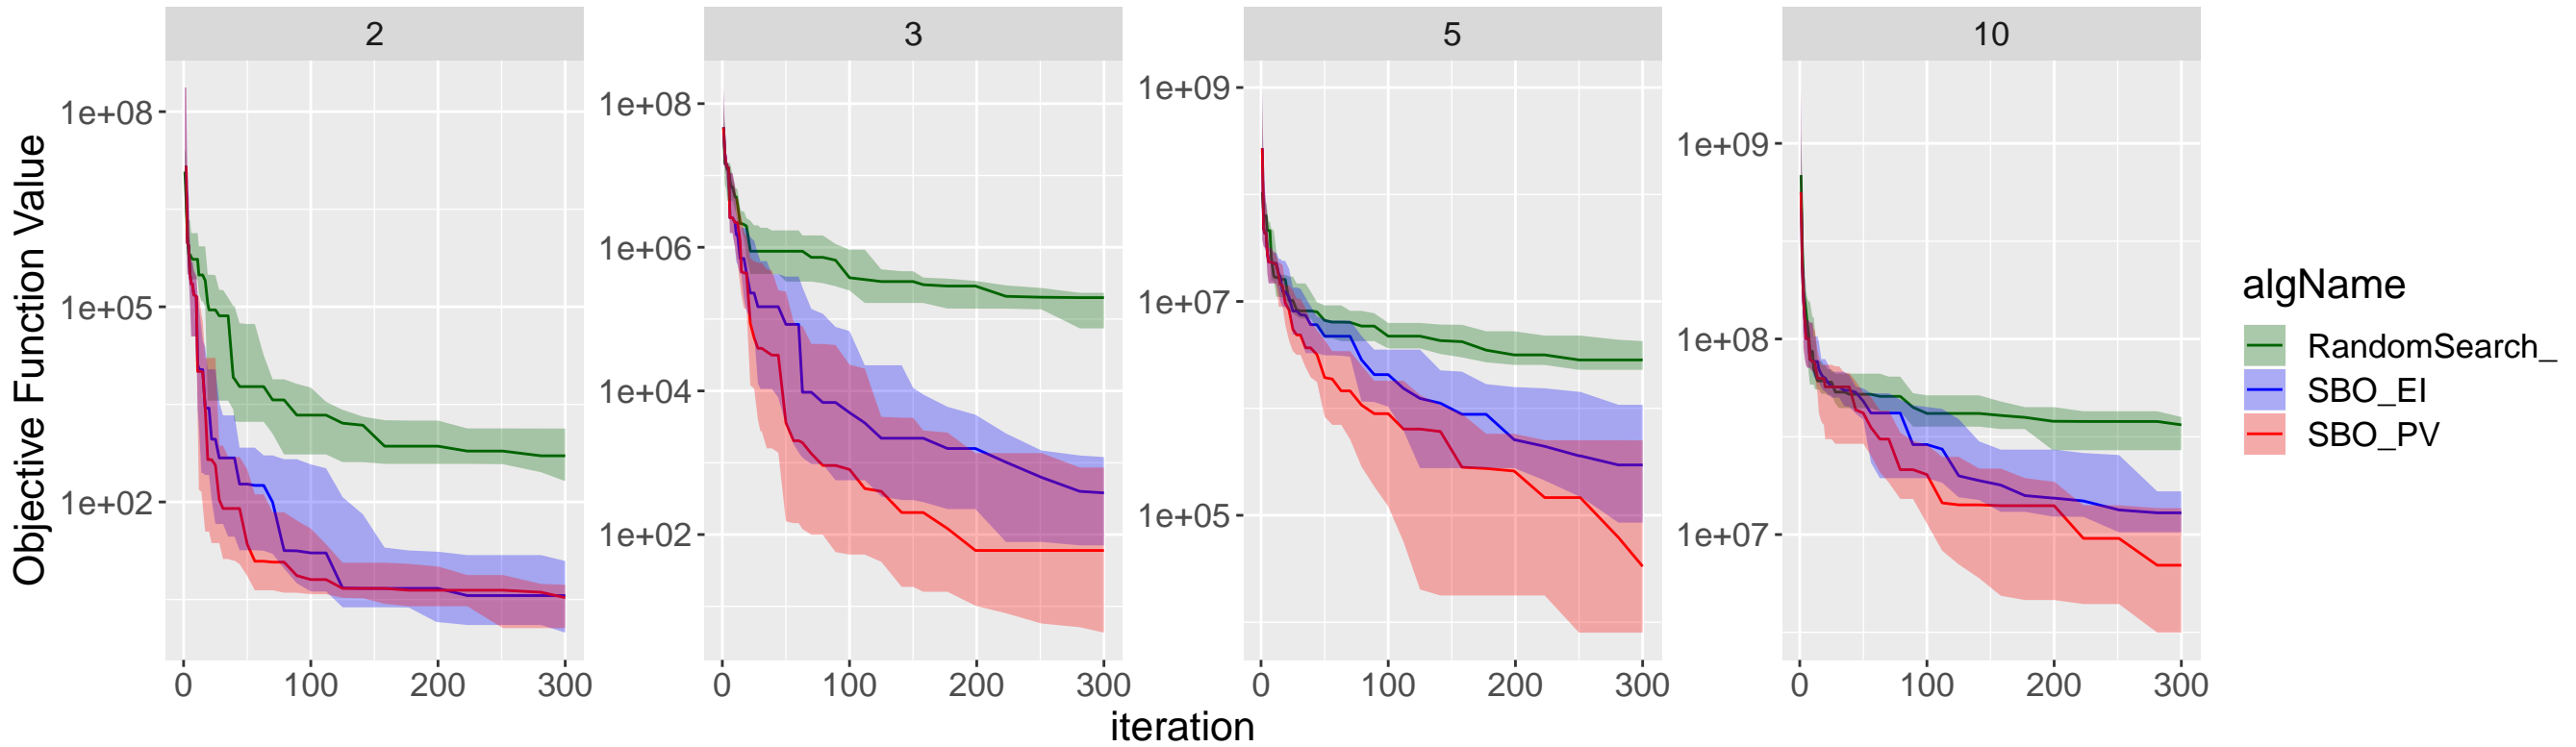

# Sharp Ridge

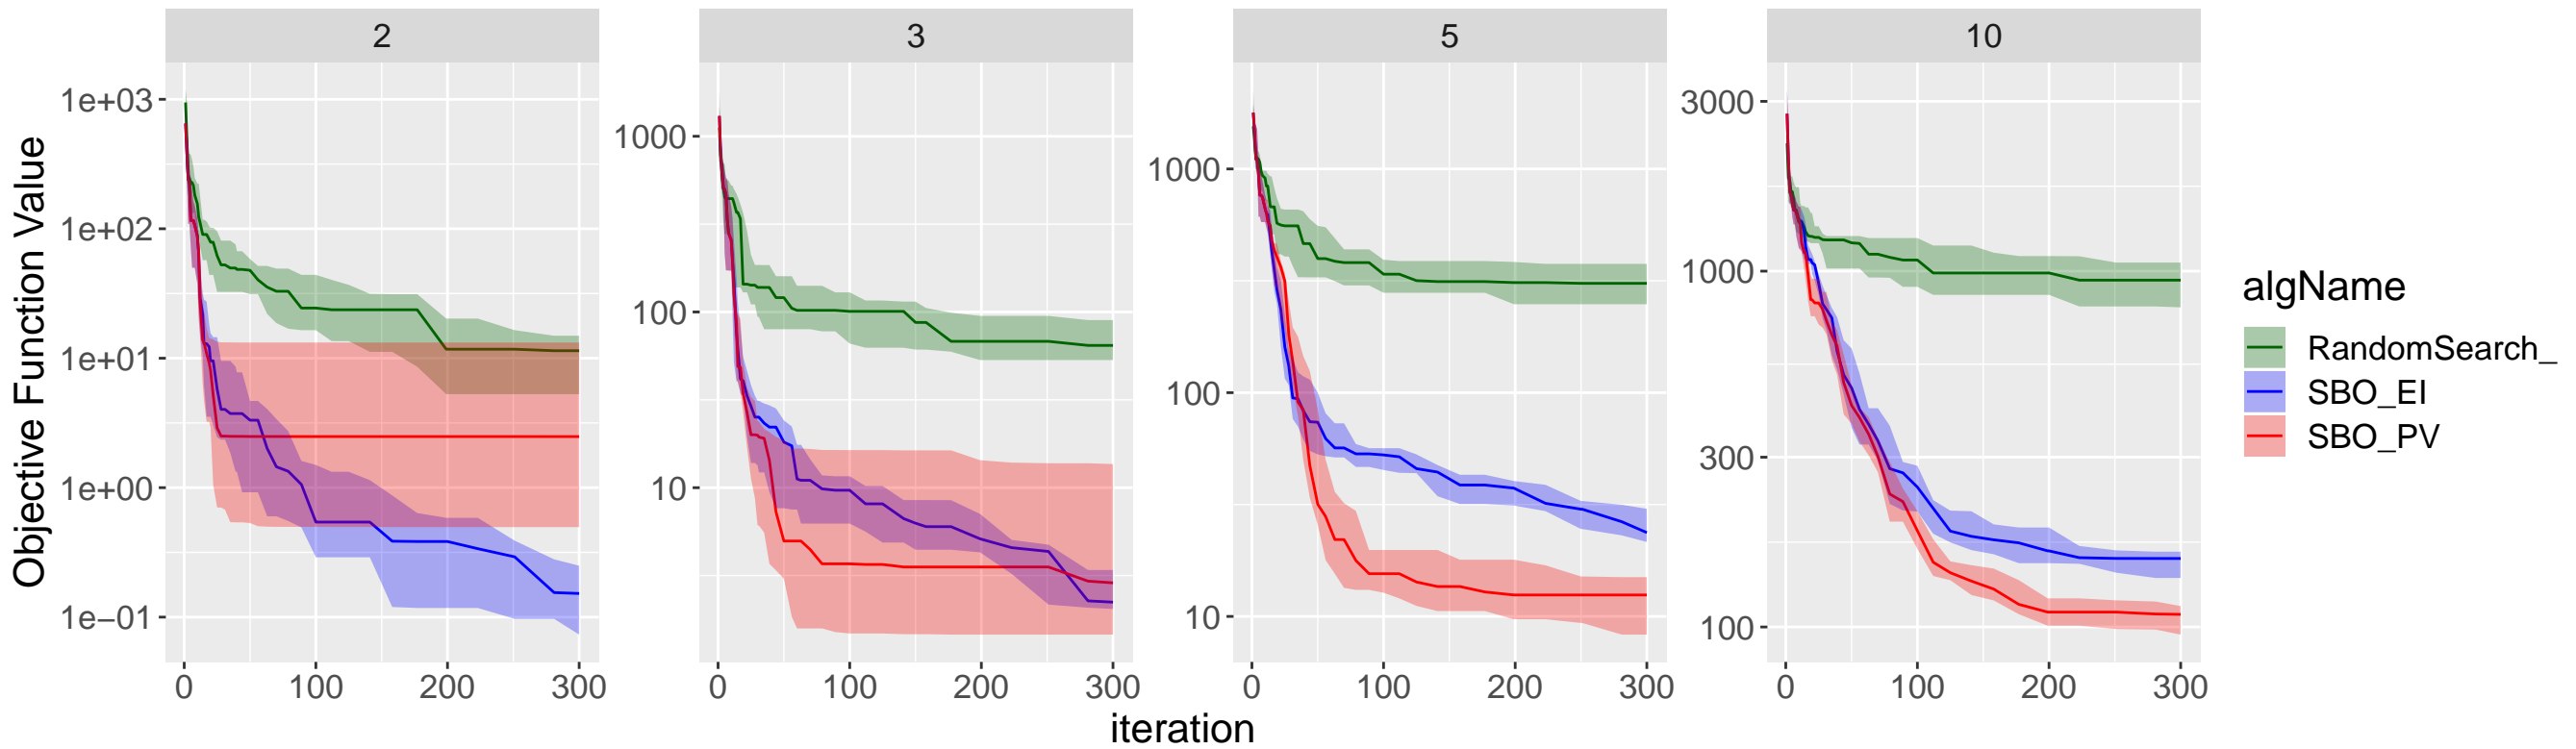

# Different Powers

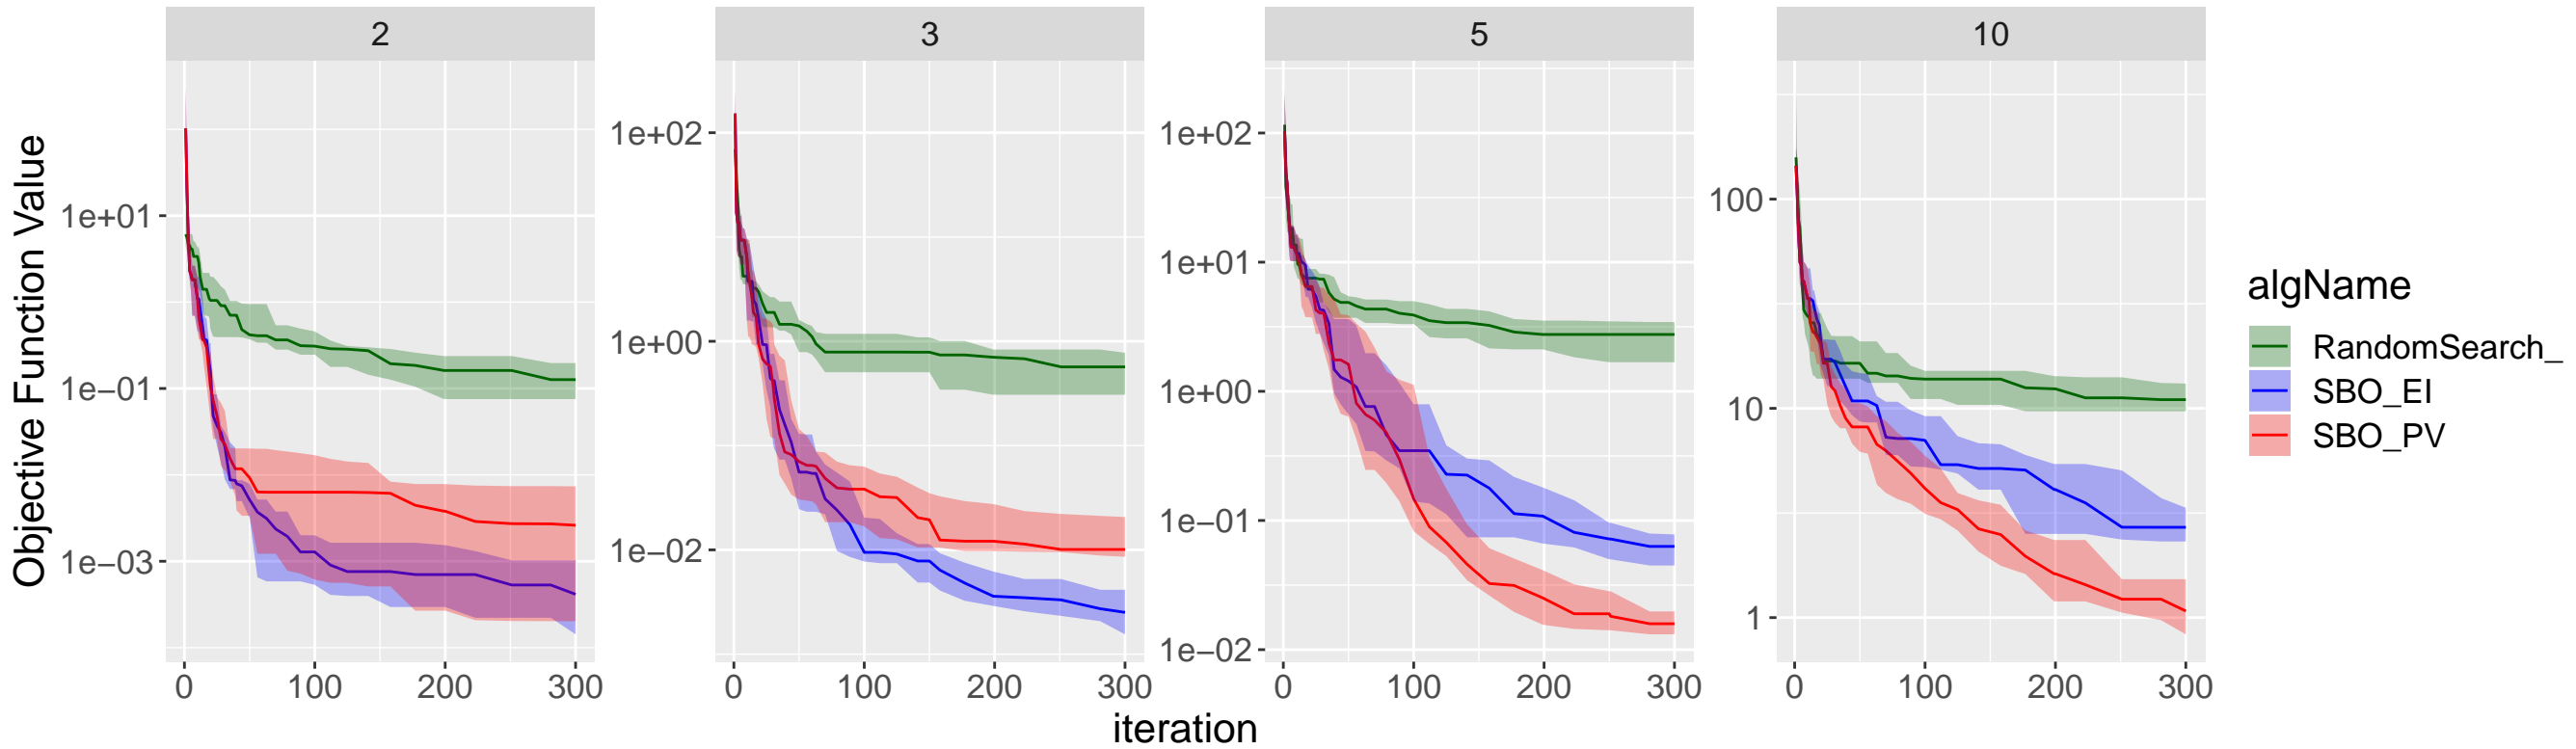

# Rastrigin

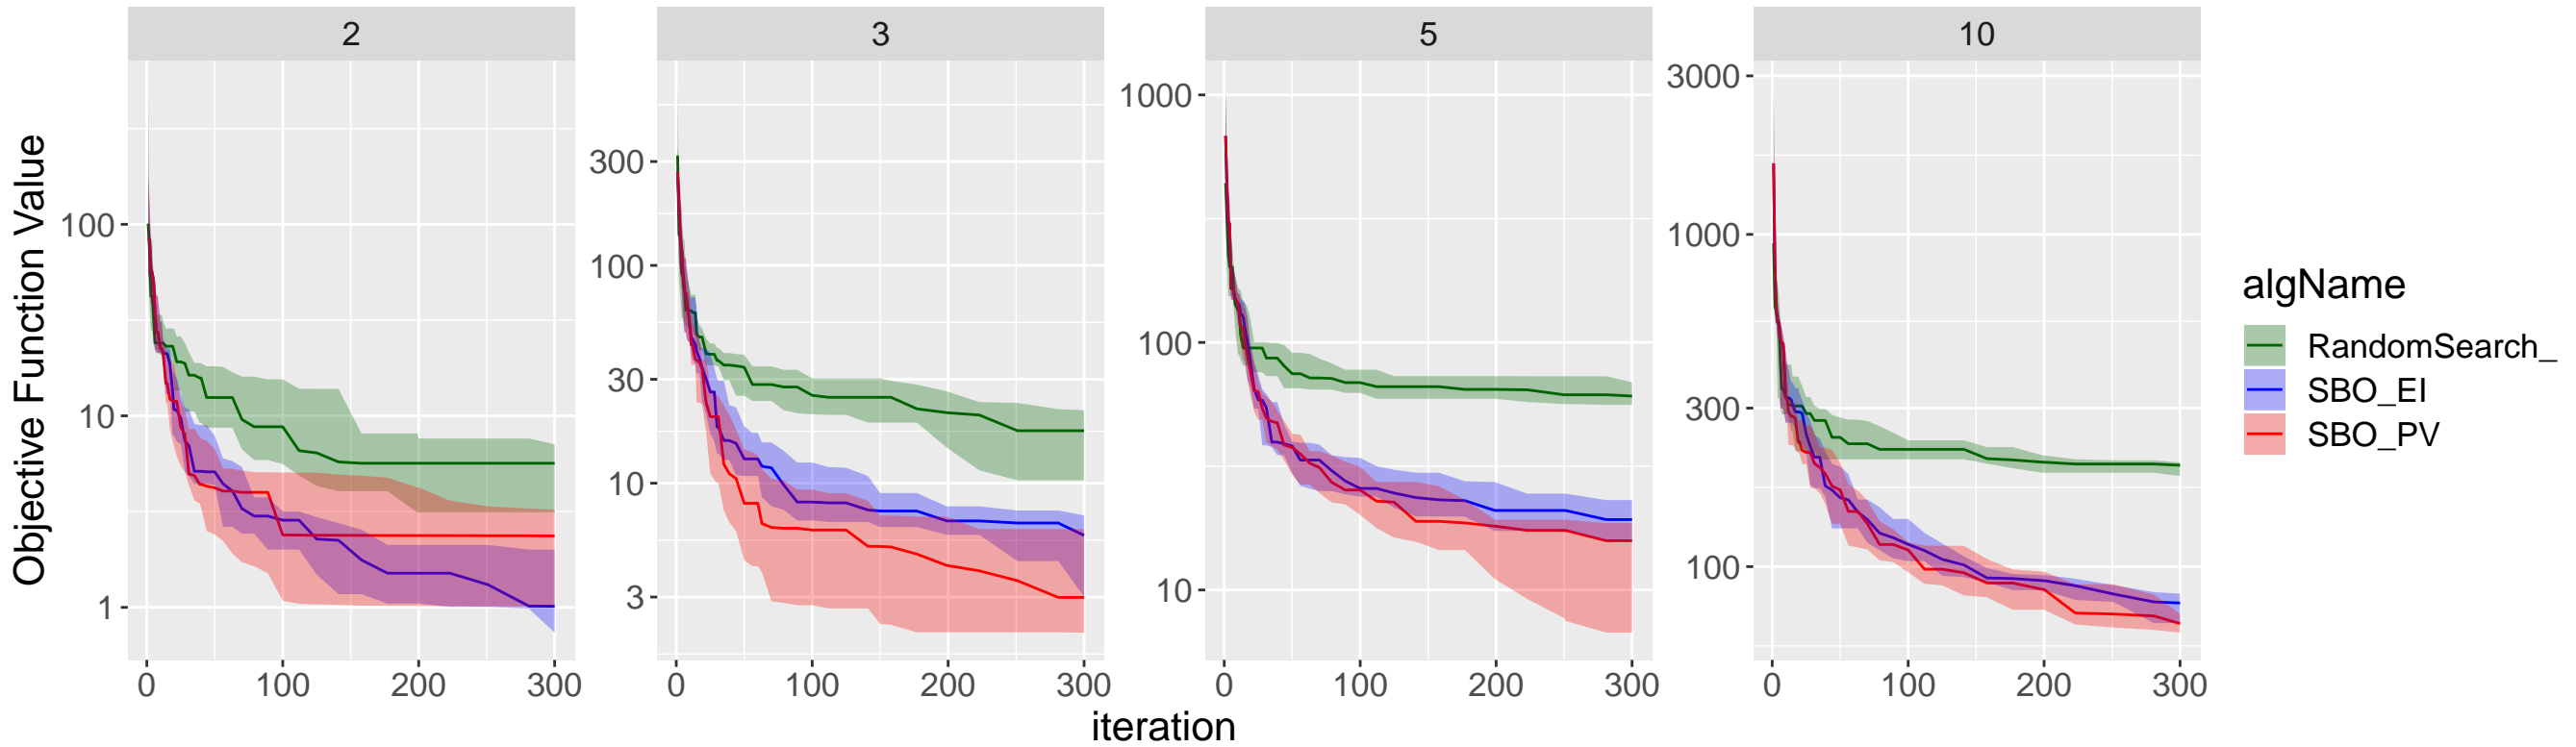

# Weierstrass

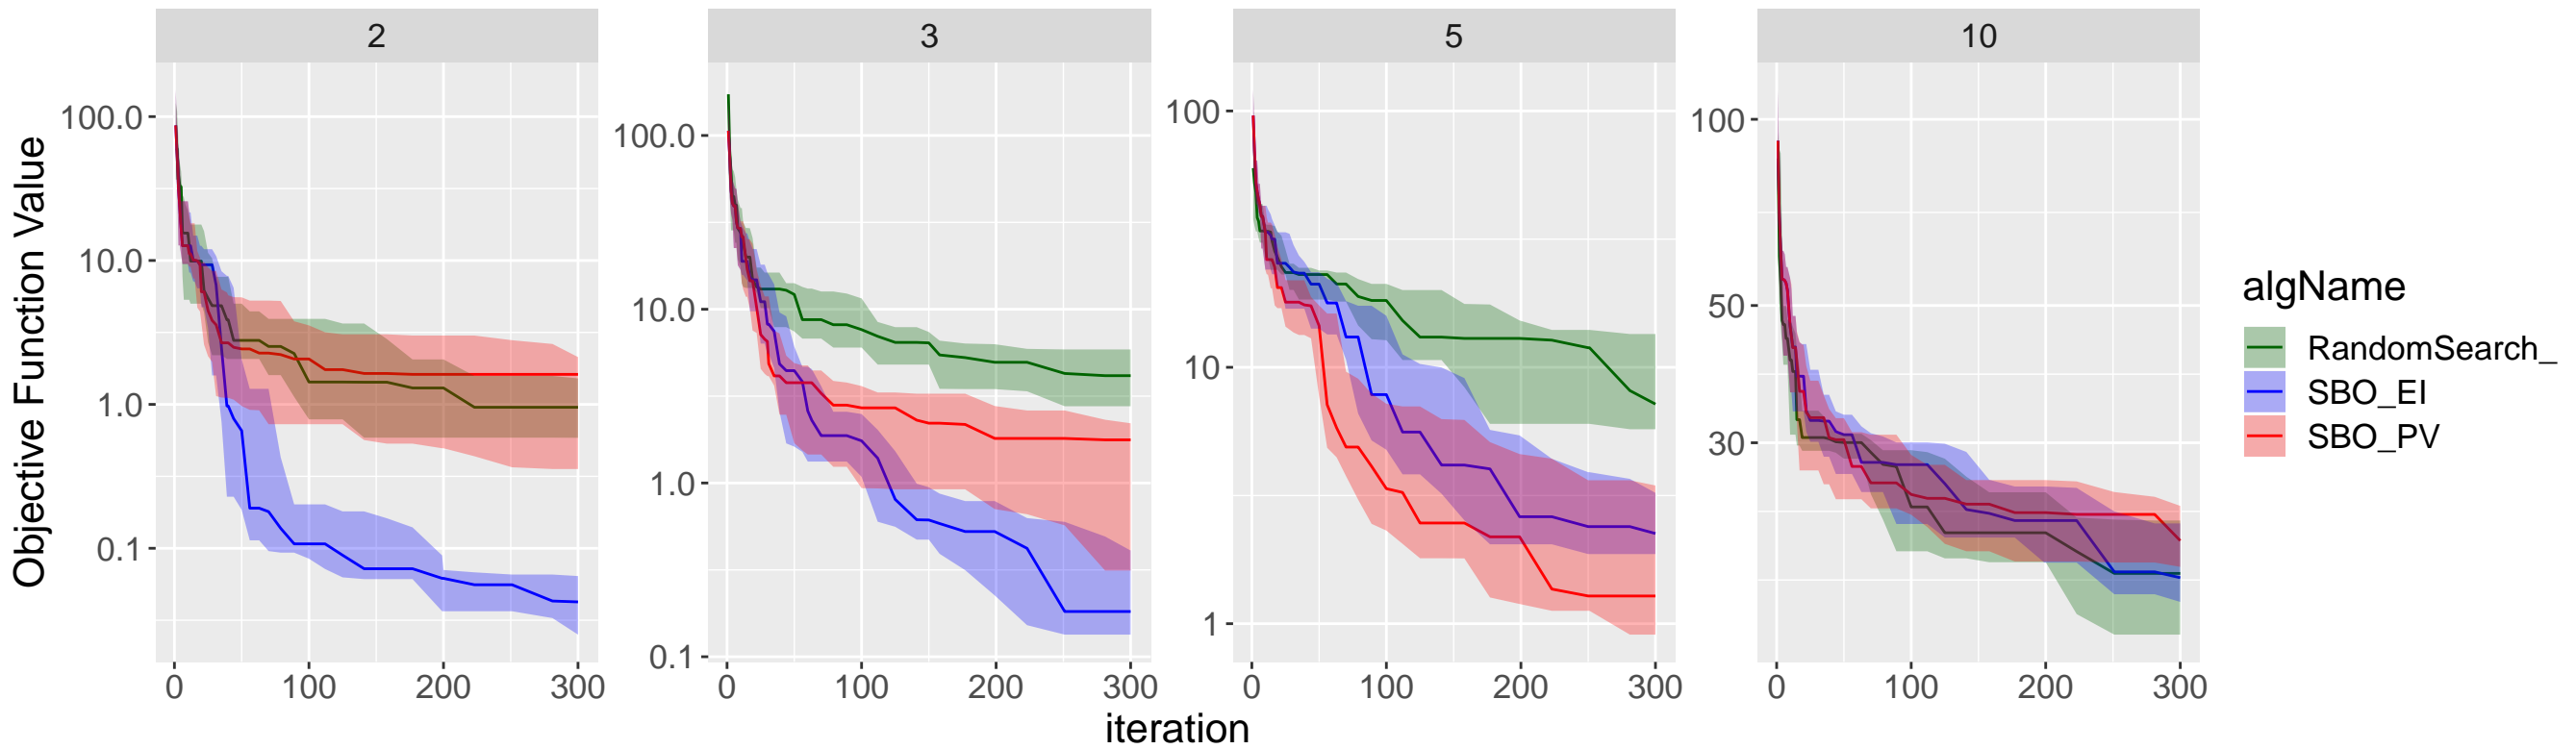



Schaffers F7

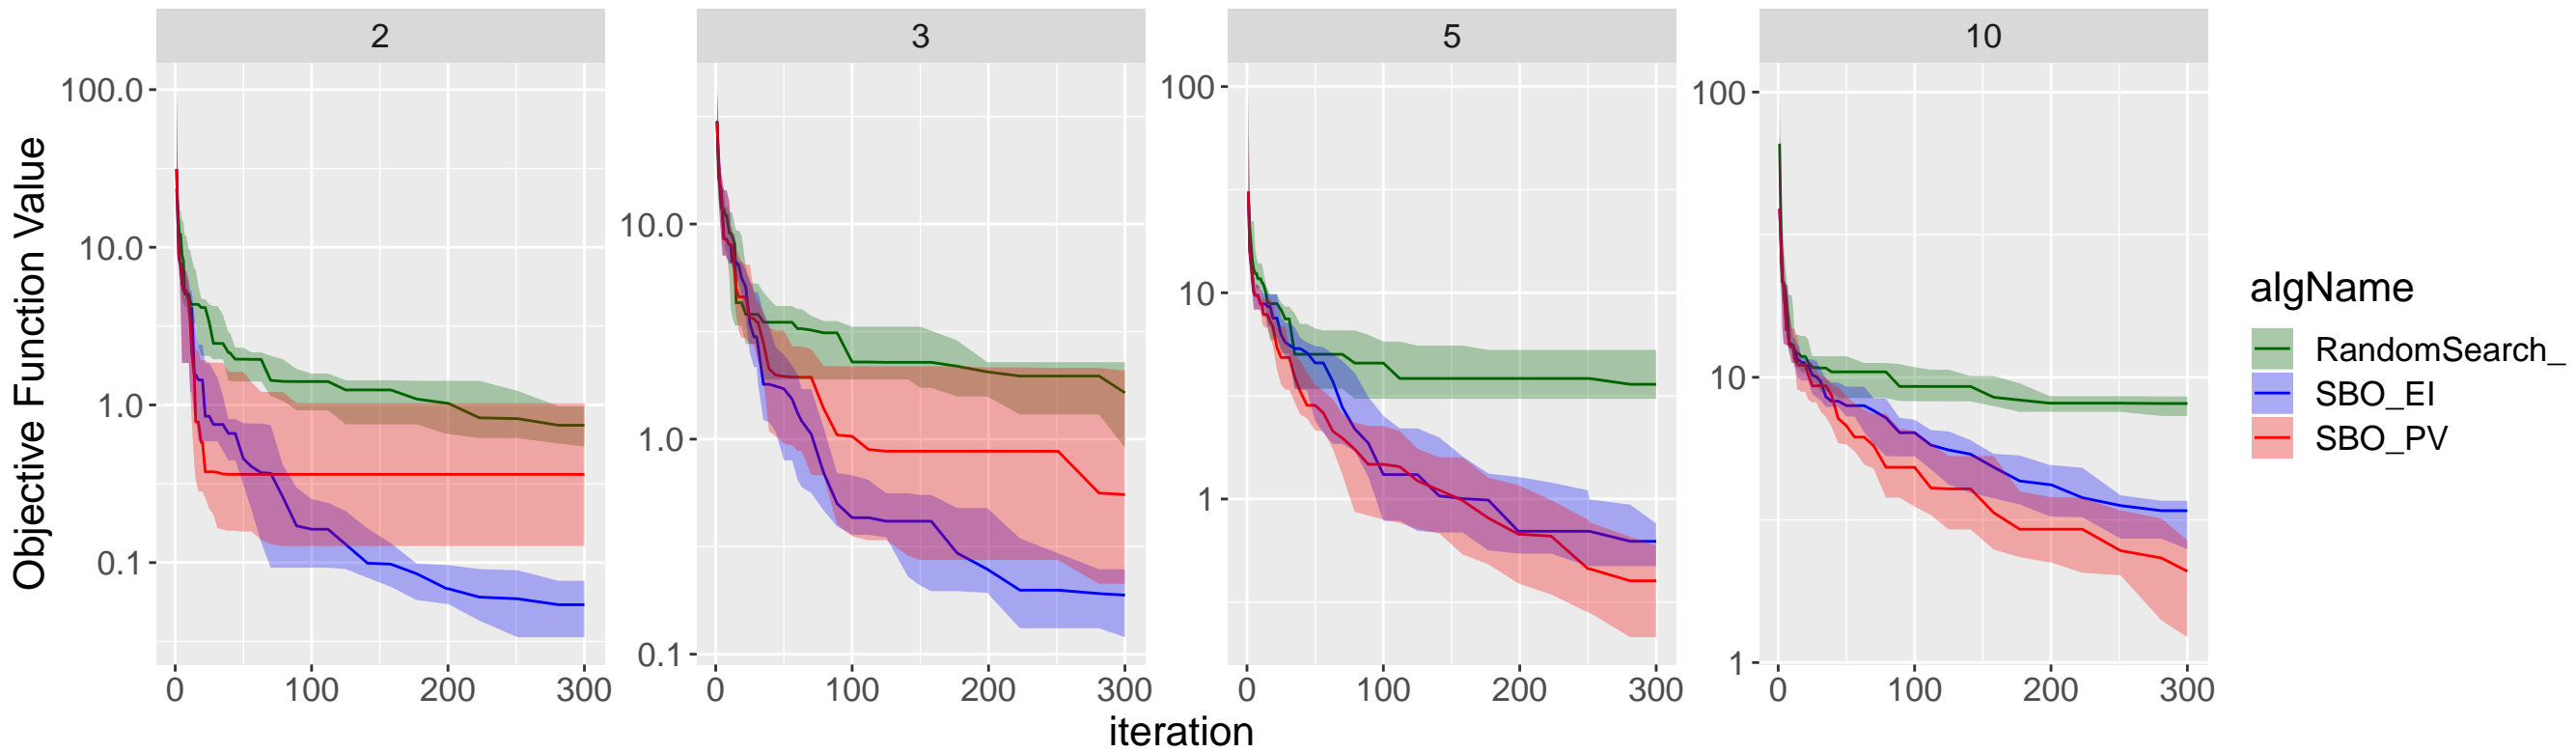

Schaffers F7

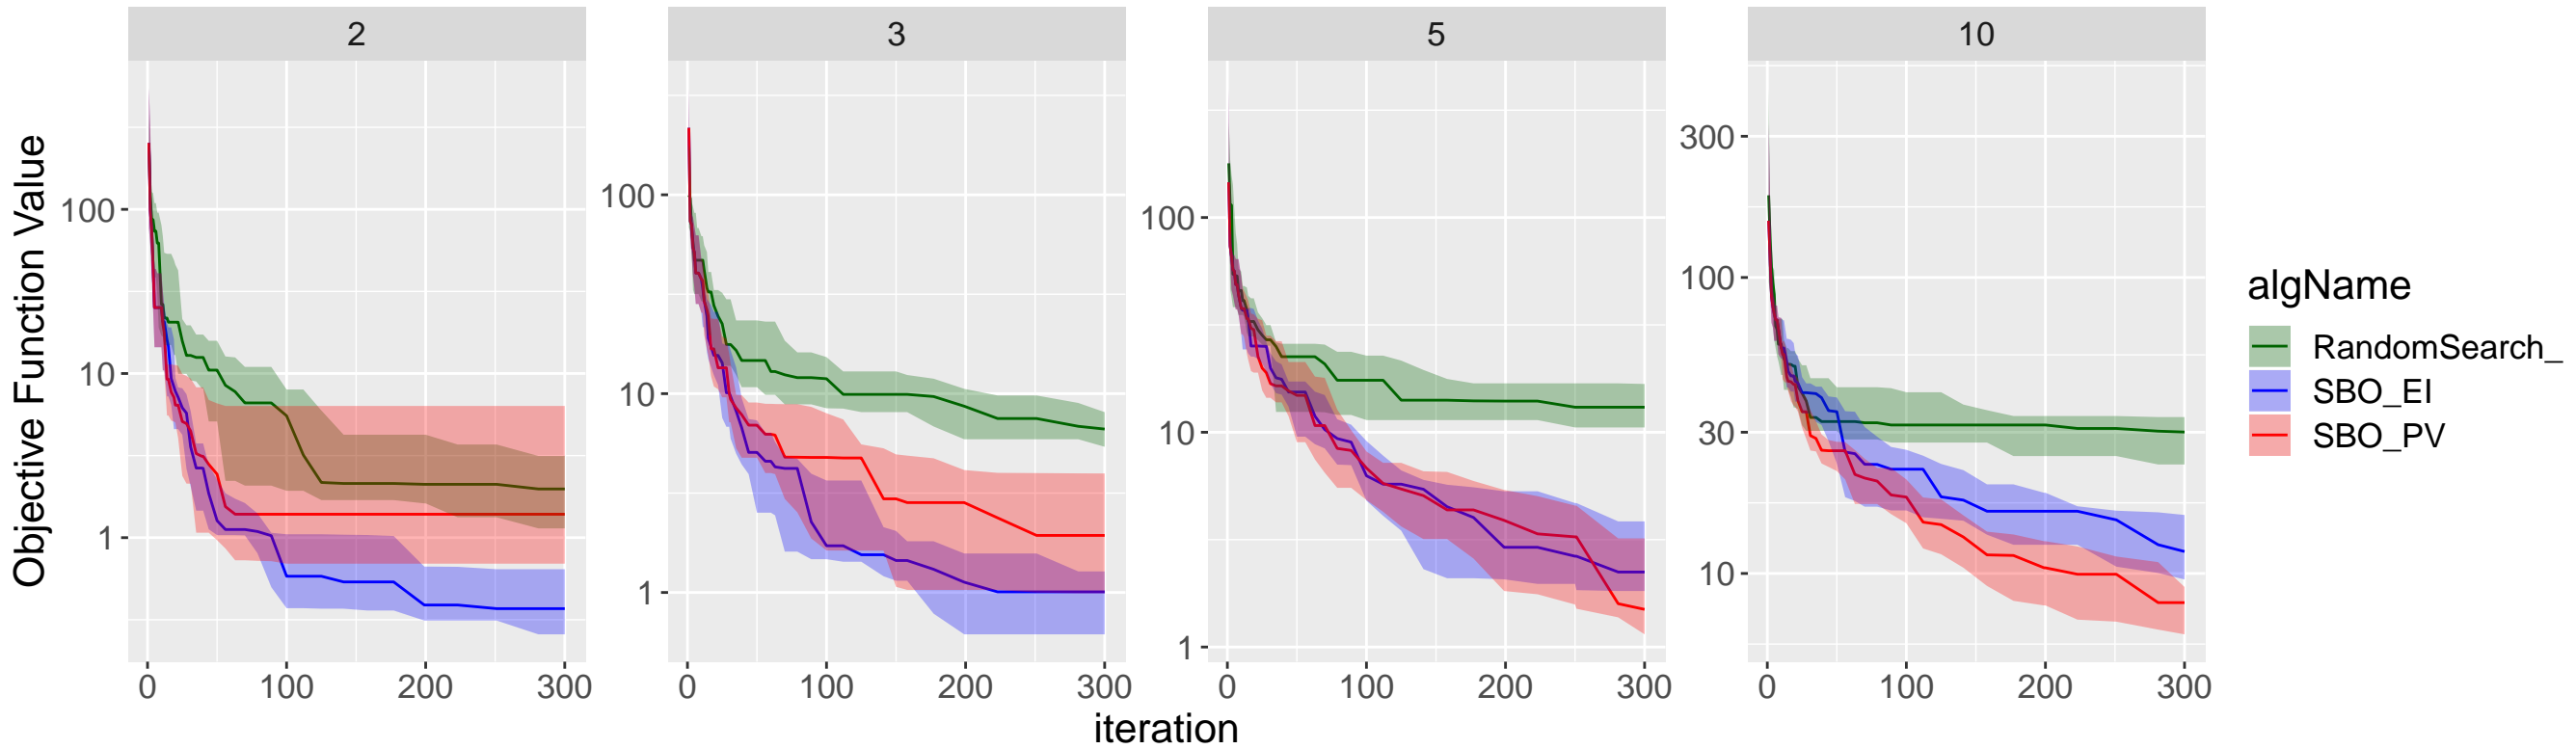

# Griwank–Rosenbrock

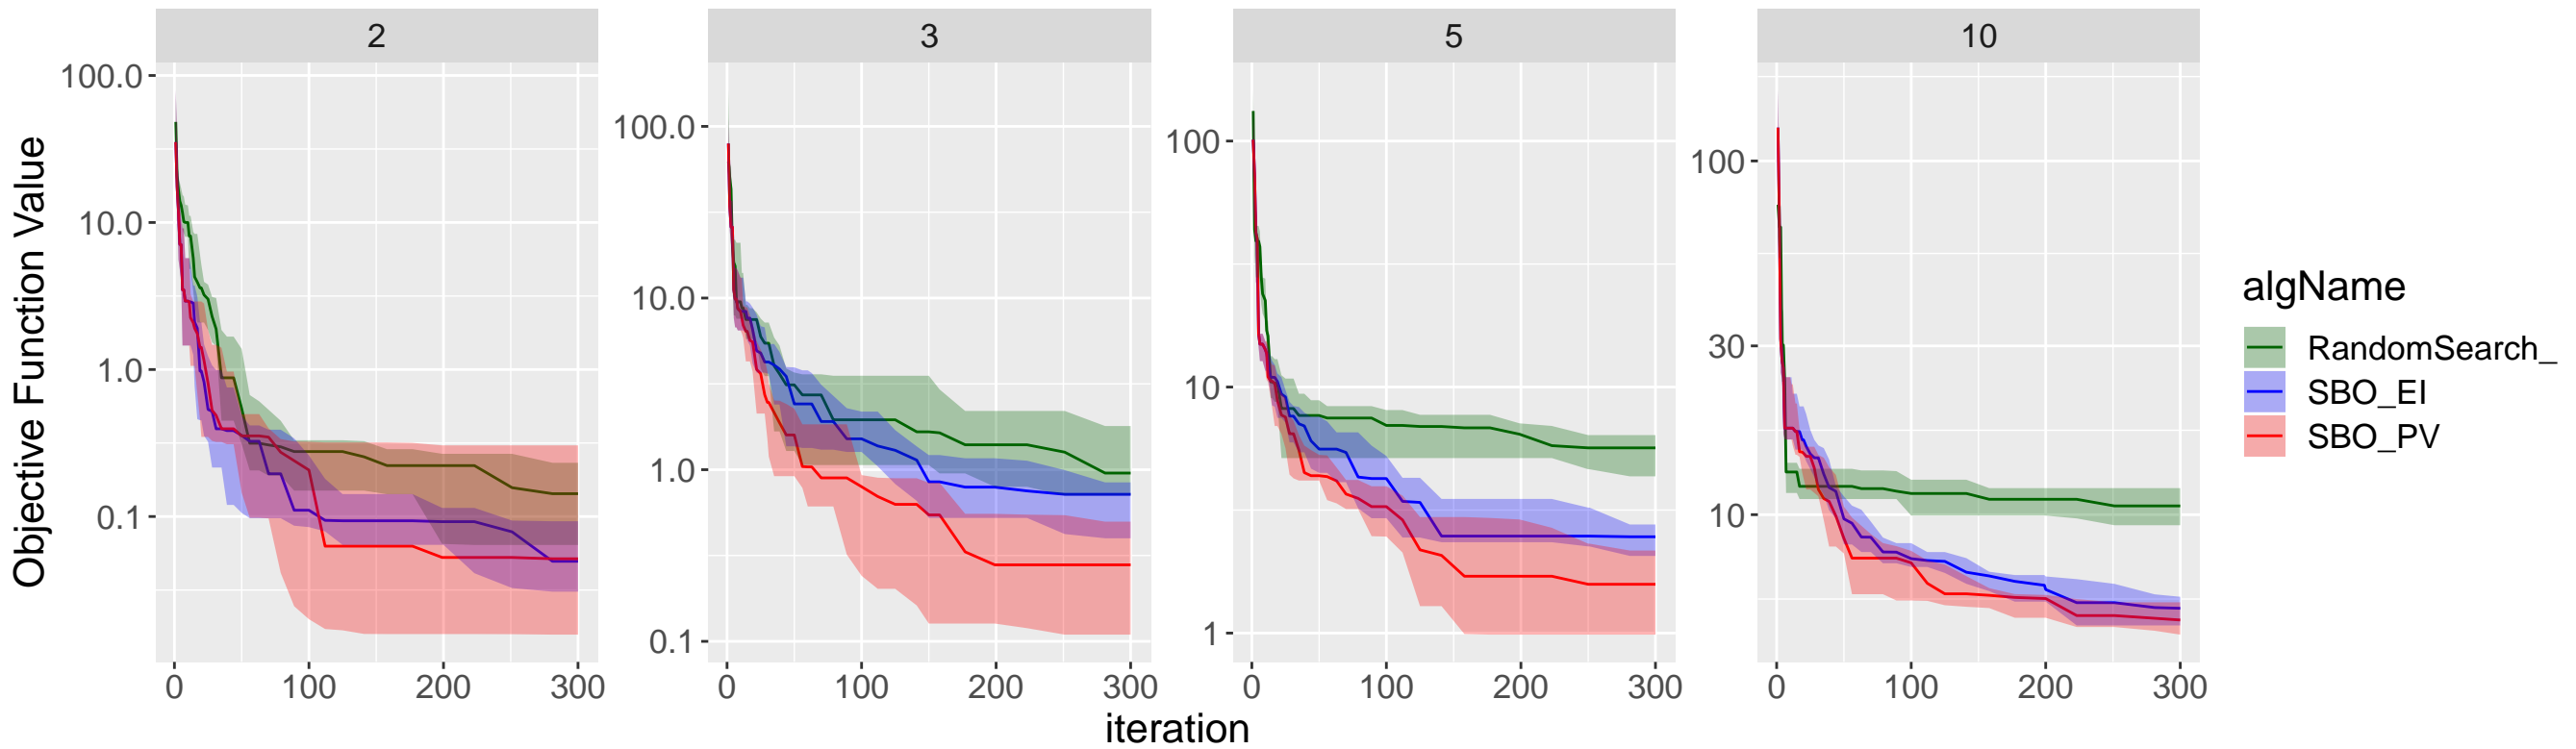

# Schwefel

Objective Function Value

2

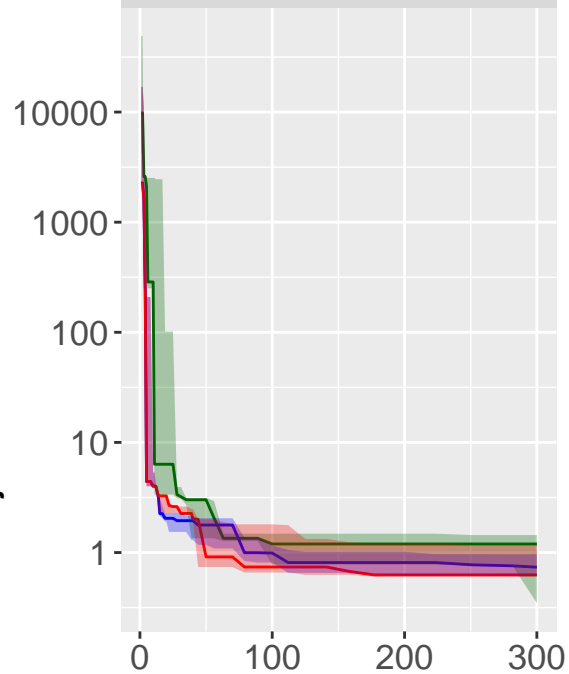

3

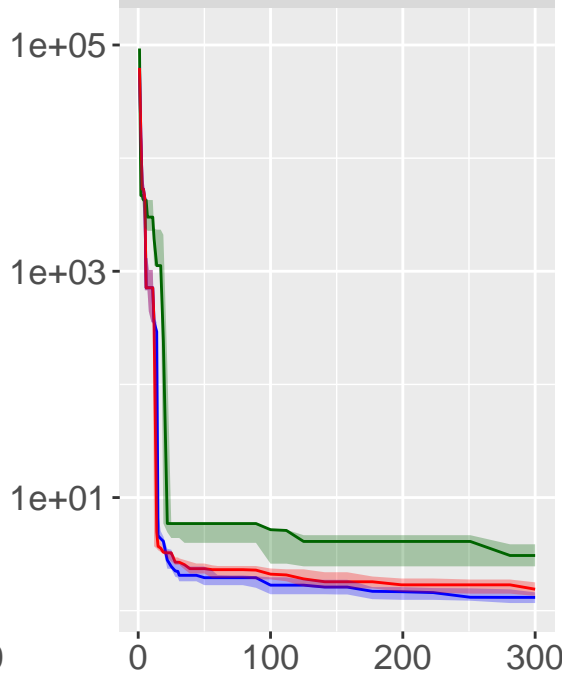

5

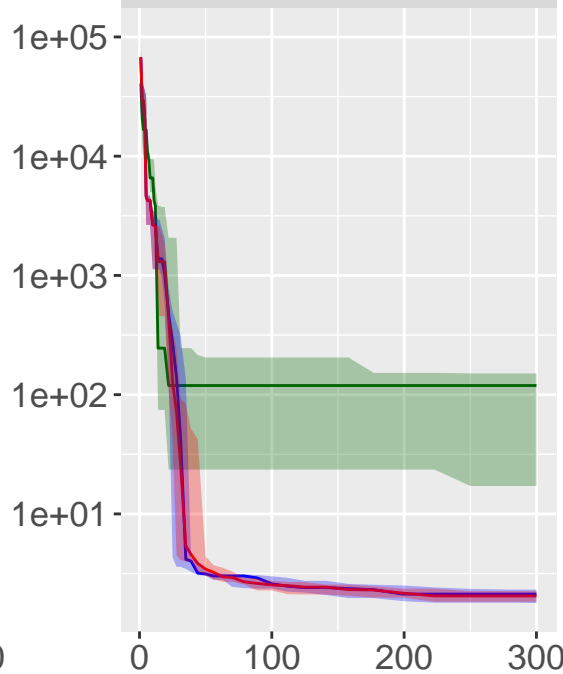

10

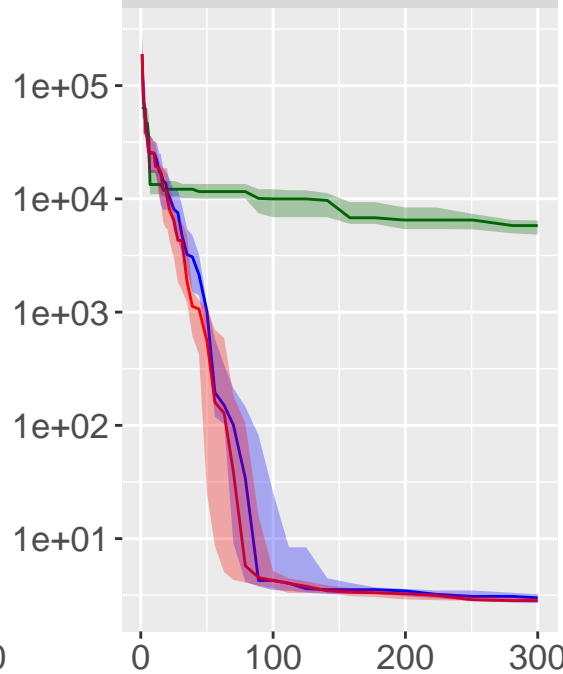

algName

- RandomSearch\_
- SBO\_EI
- SBO\_PV

# Gallagher Gaussian 101-me Peaks

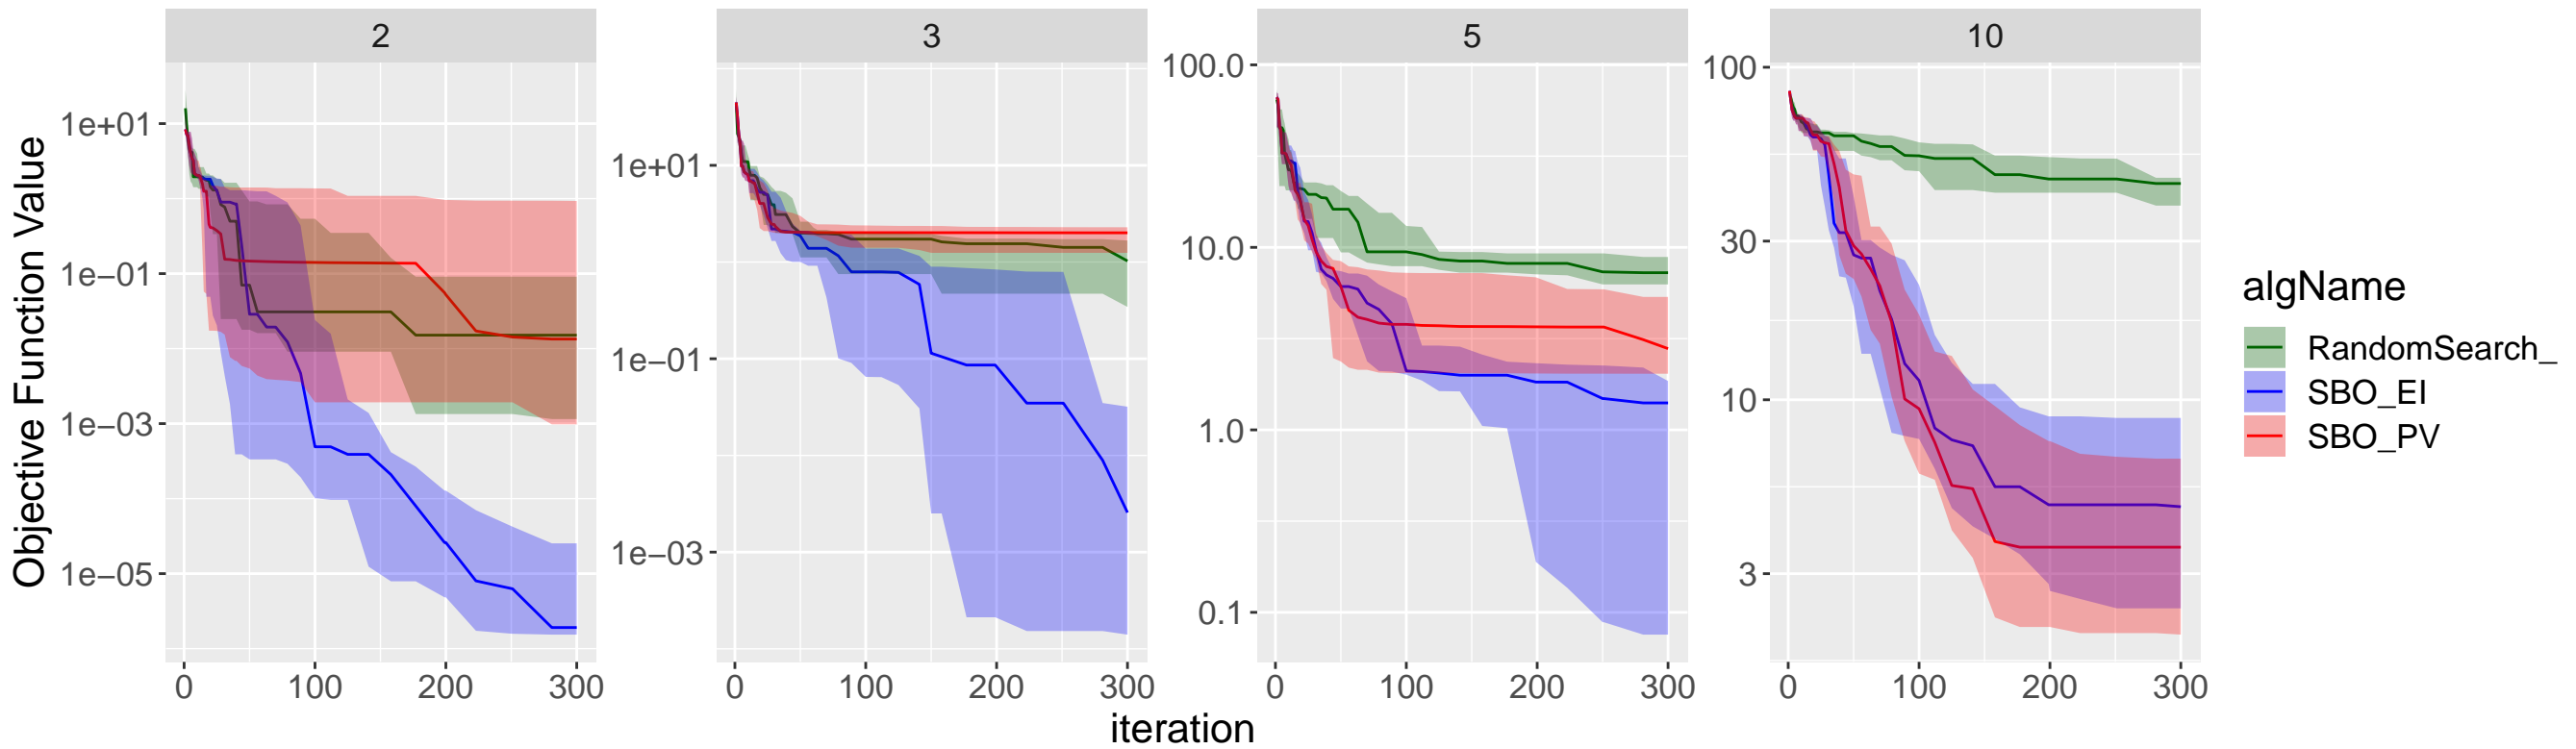

# Gallagher Gaussian 21-hi Peaks

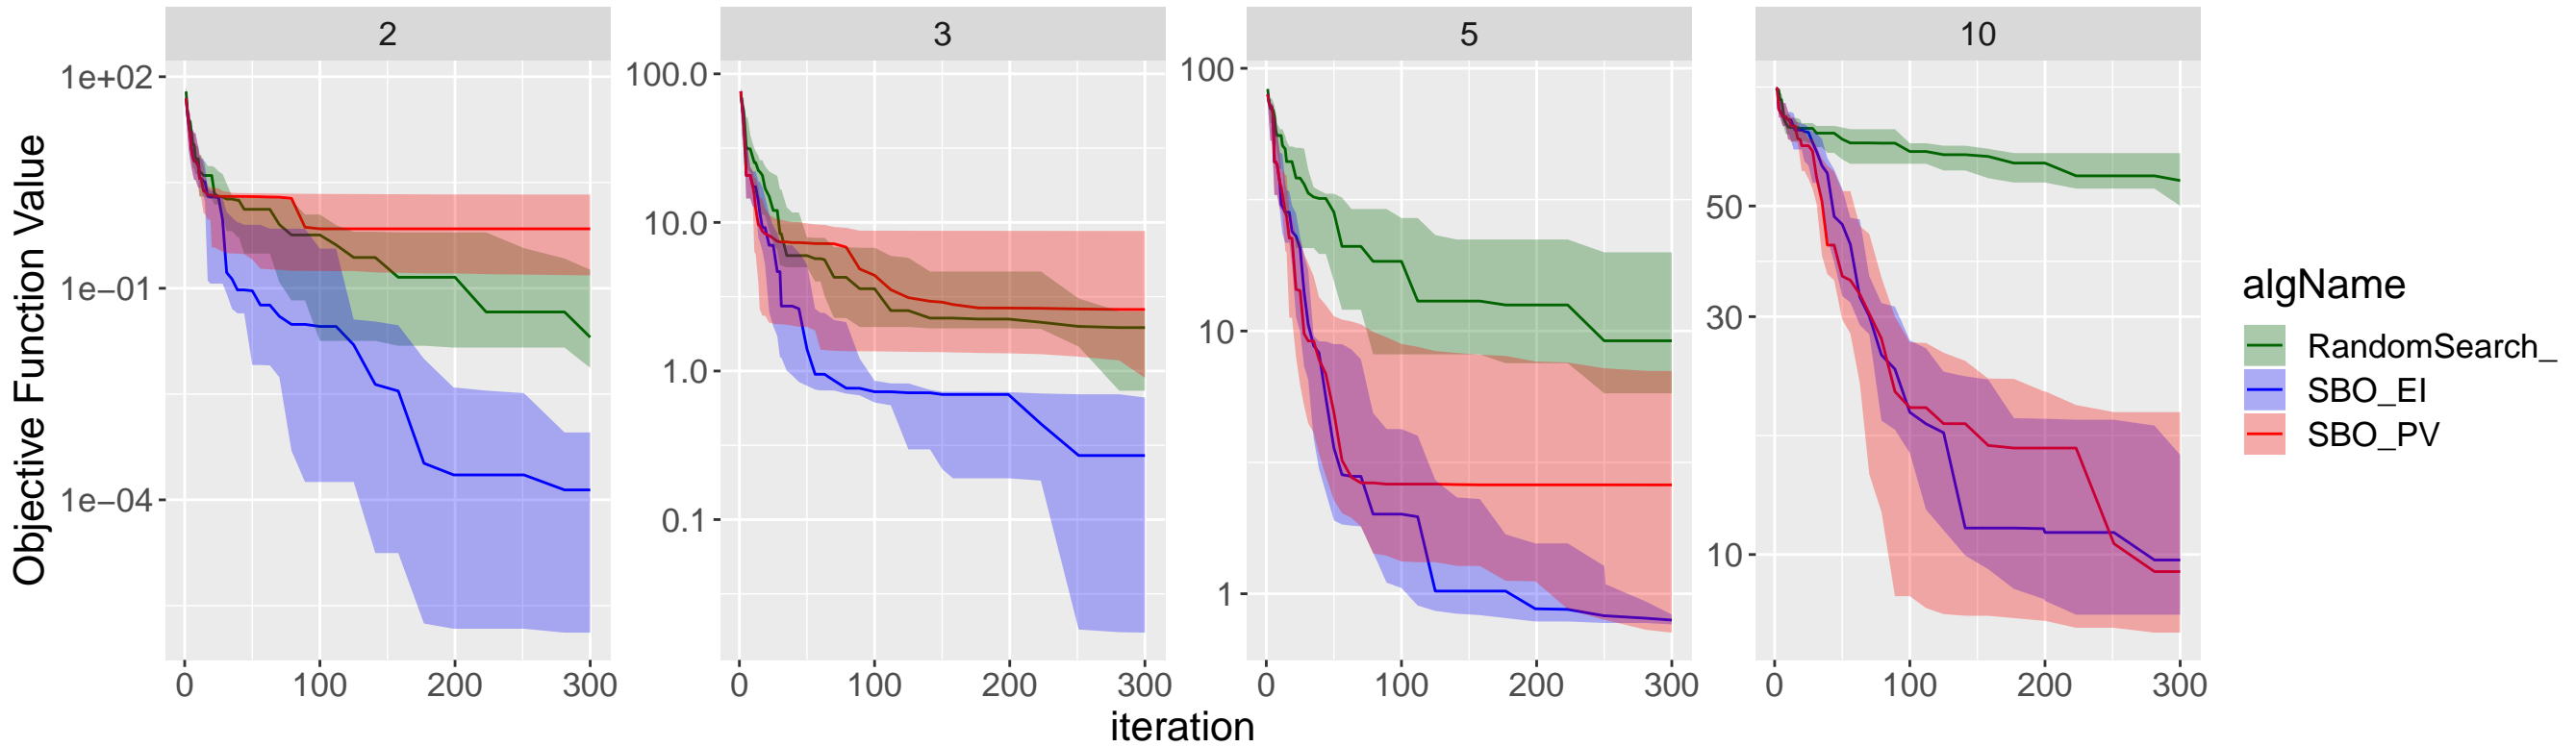

# Katsuura

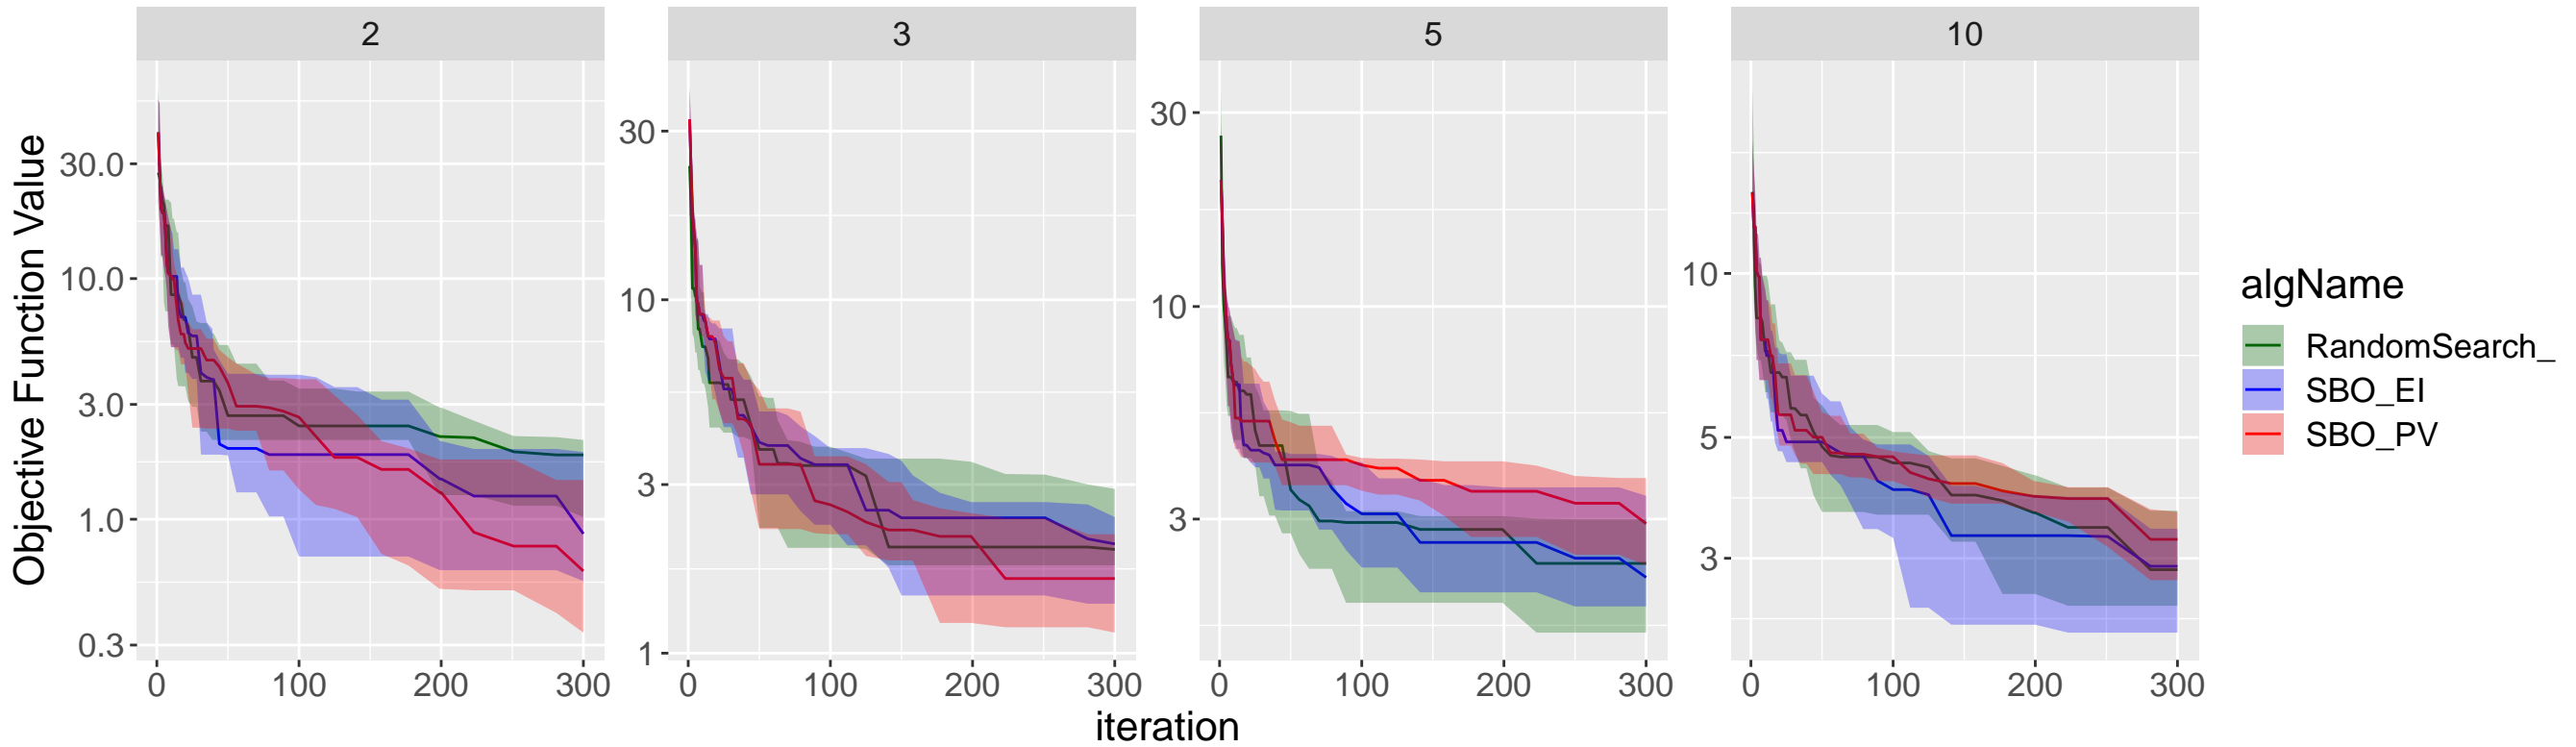

# Lunacek bi-Rastrigin

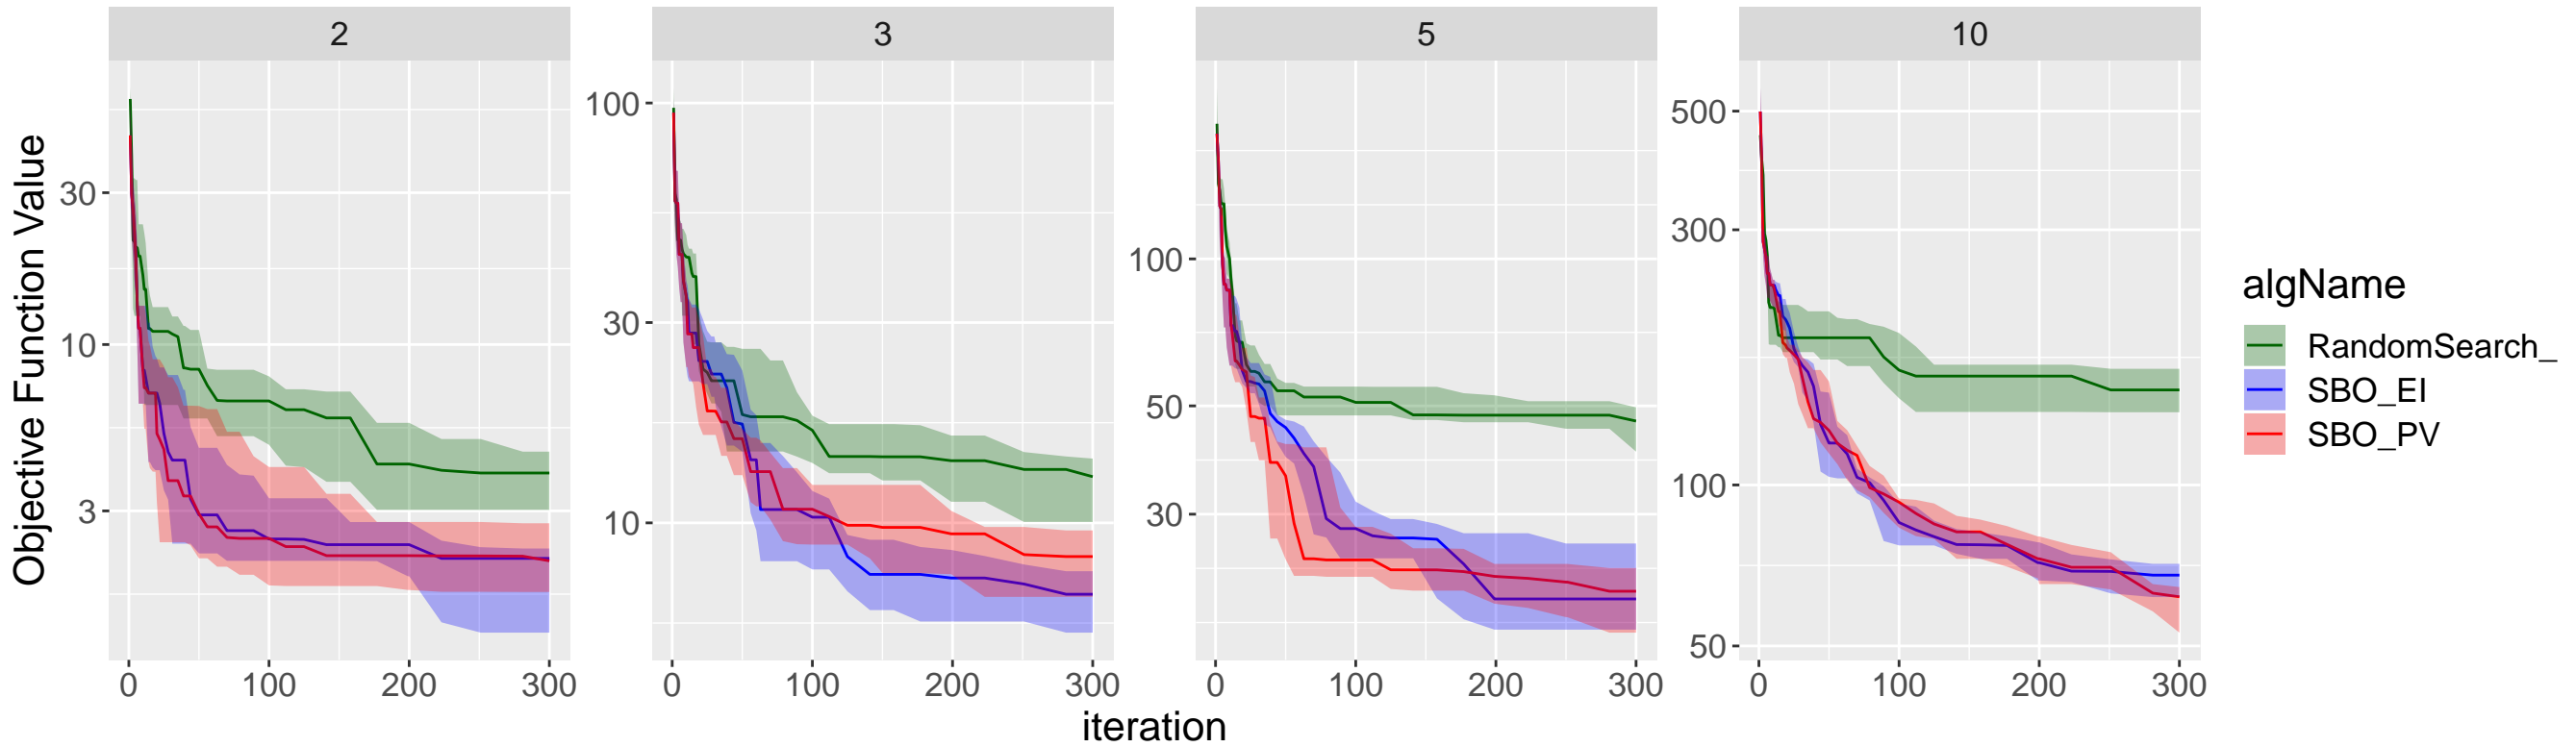

Supplement: Supplementary file 2 [file convergenceSpotOnBBOB.pdf]
