# Supplementary material for: Expected Improvement versus Predicted Value in Surrogate-Based Optimization
Source: arXiv:2001.02957 ancillary file (2020-02-17)

# Sphere

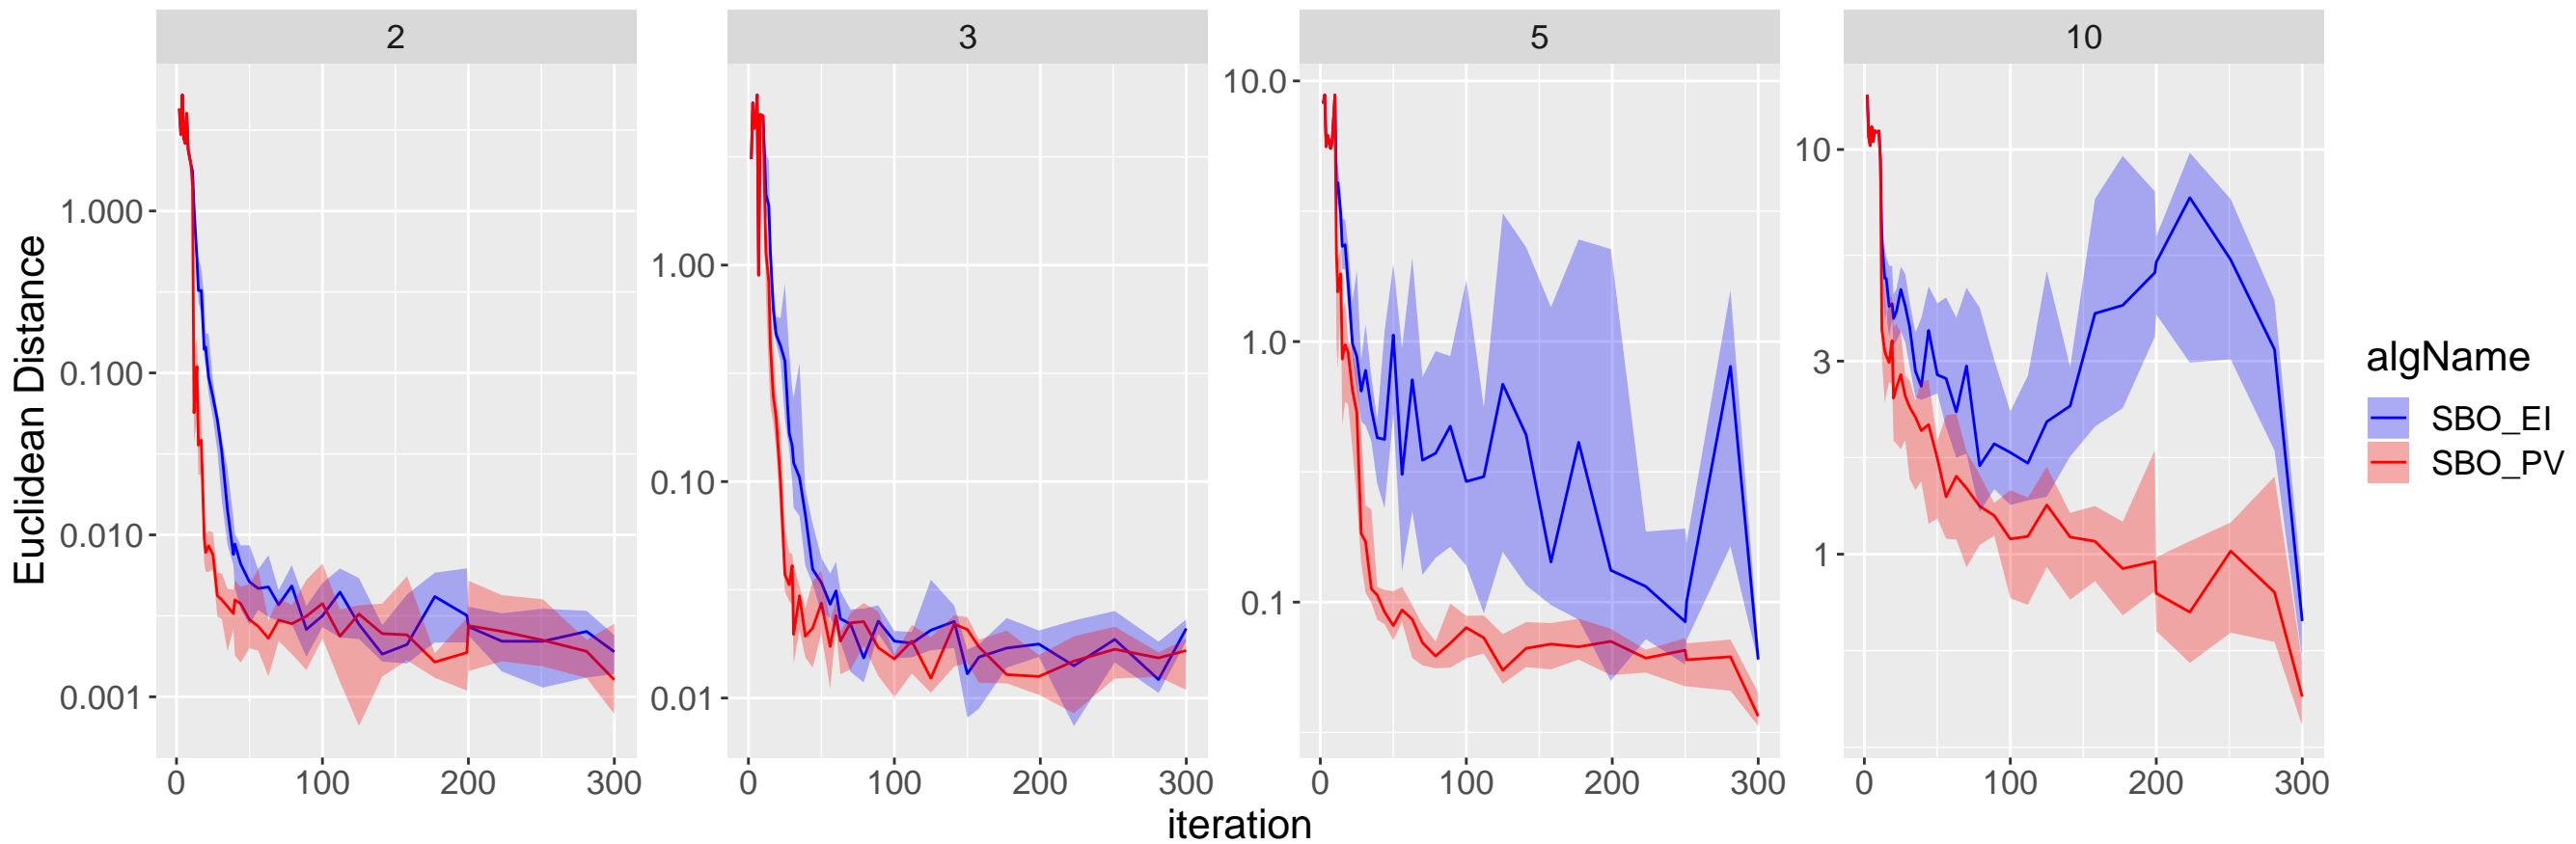

# Ellipsoidal

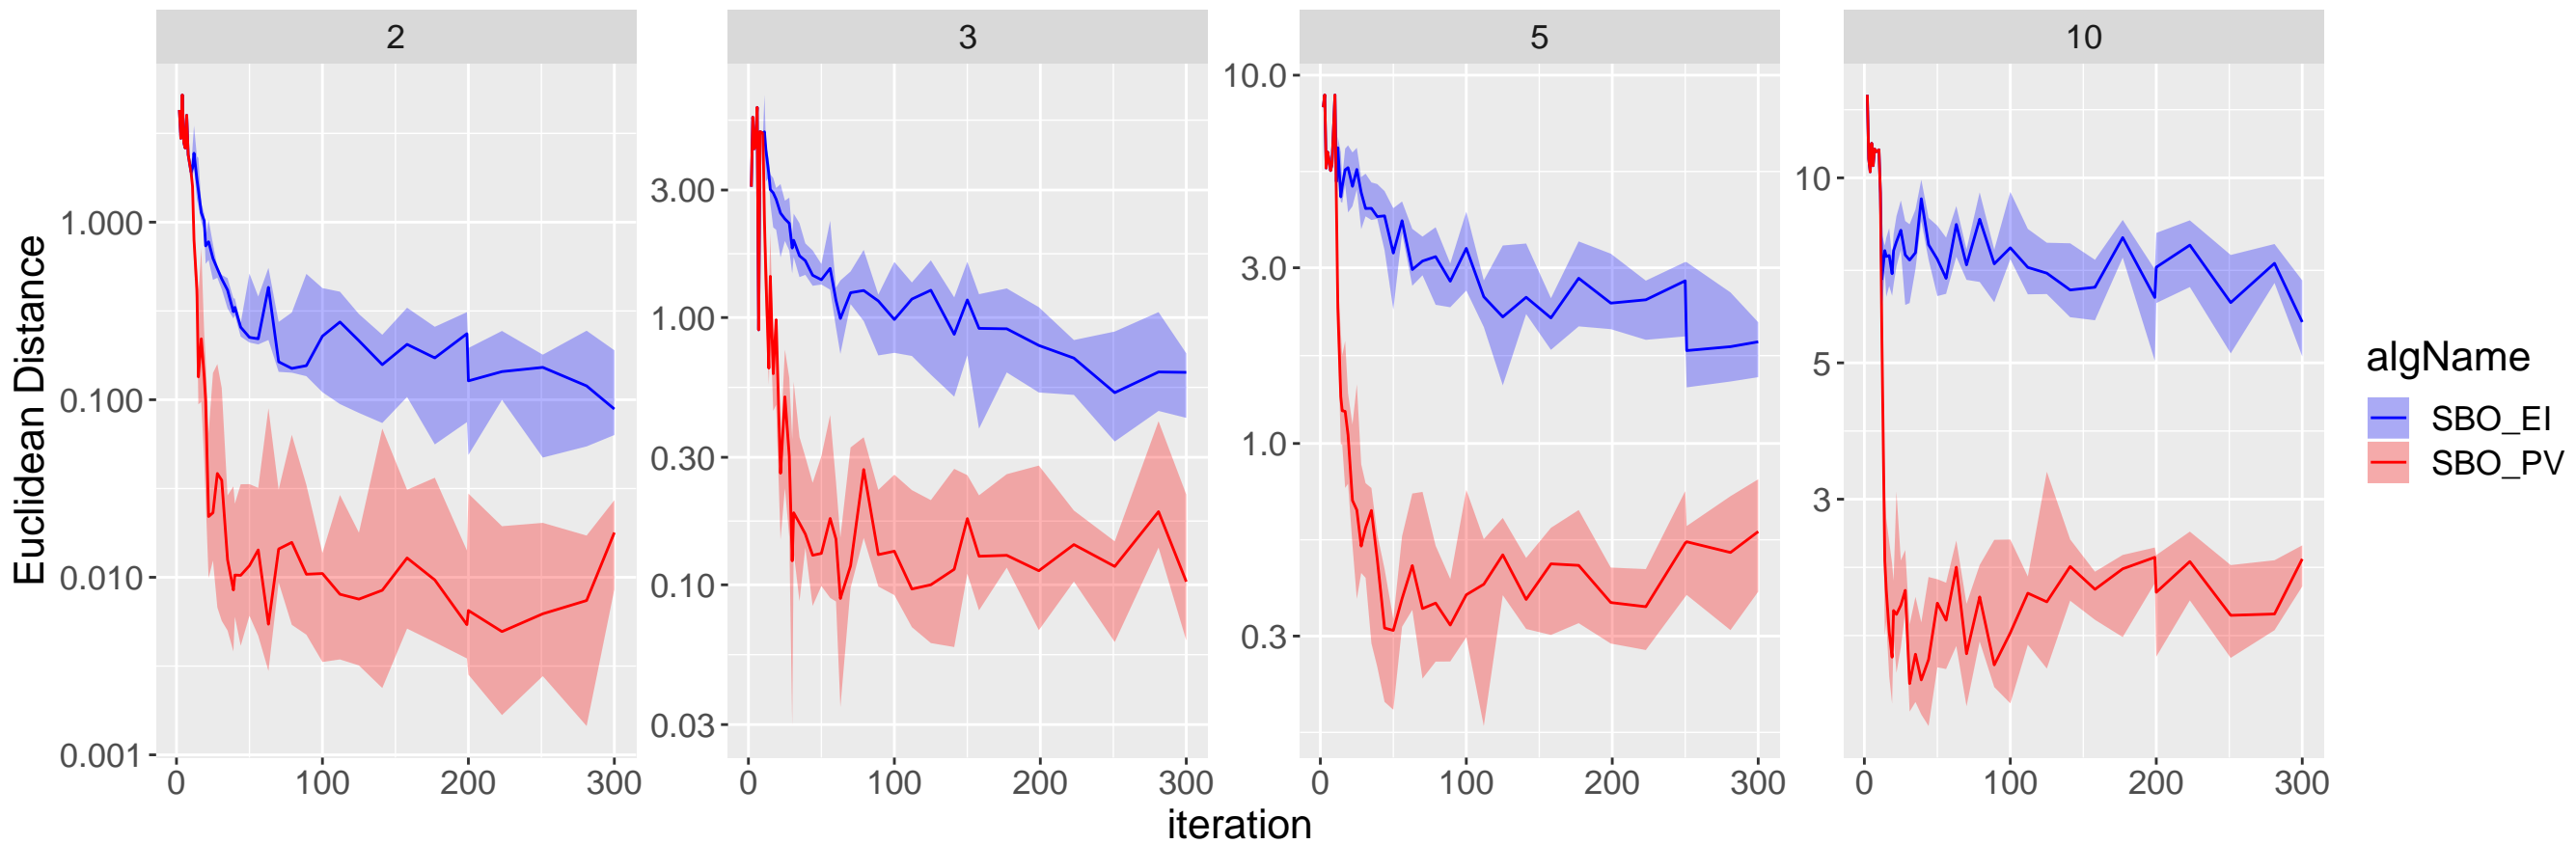

# Rastrigin

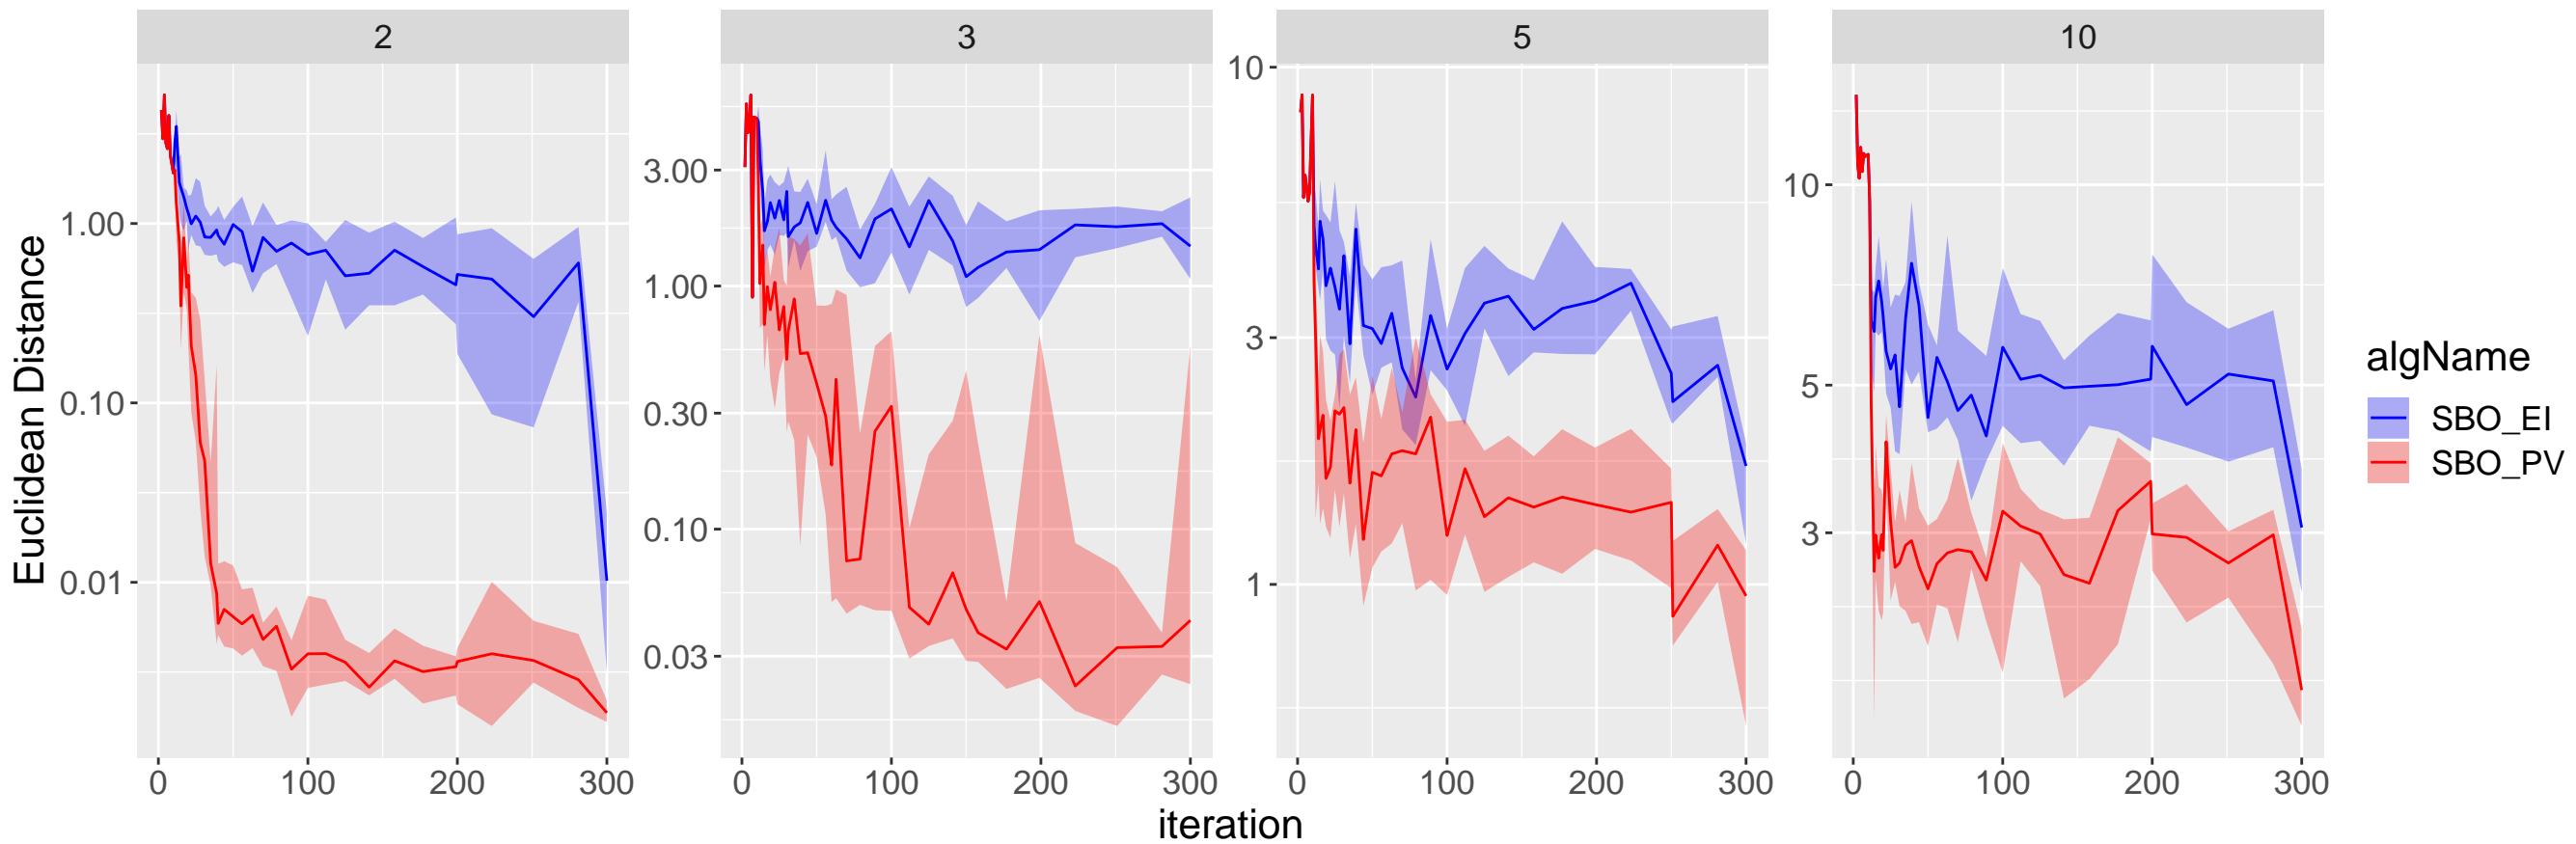

# Büche–Rastrigin

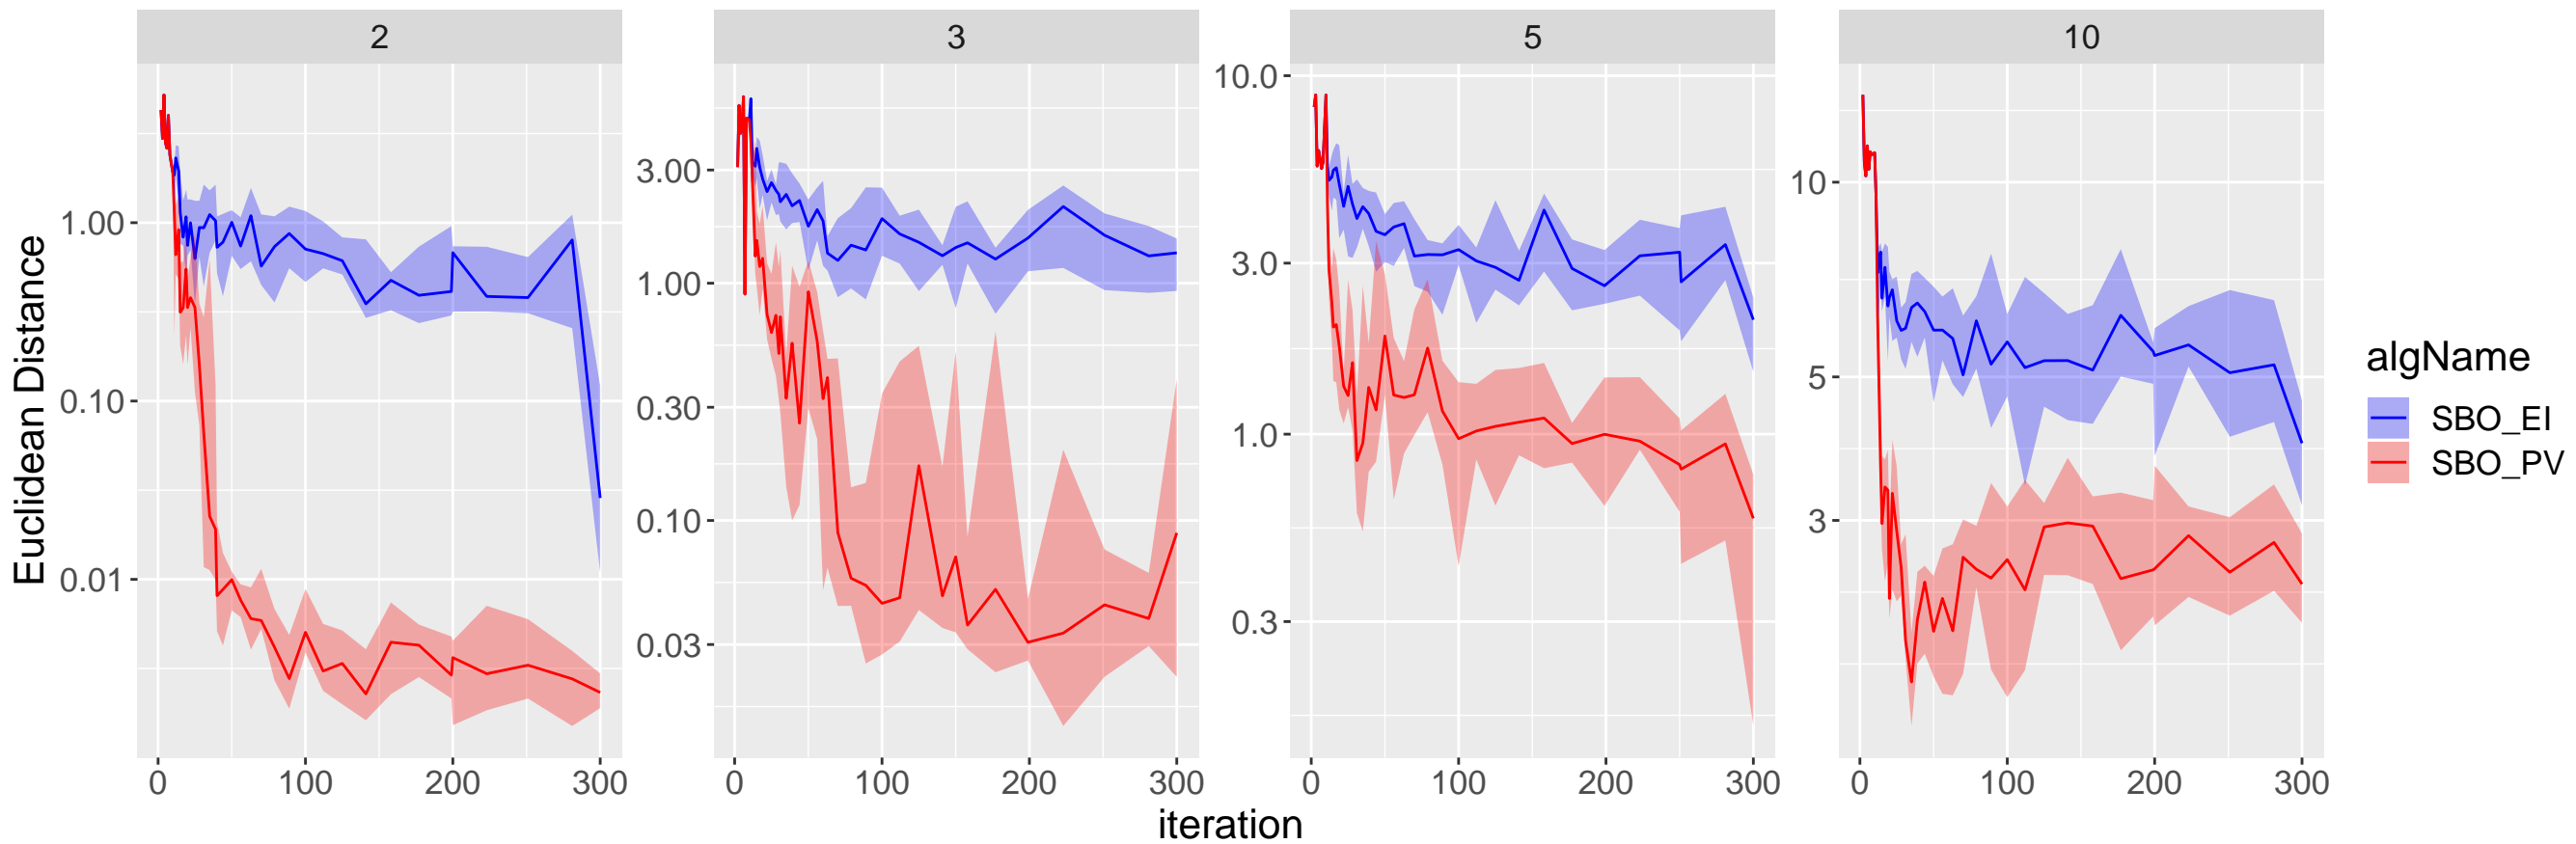

# Linear Slope

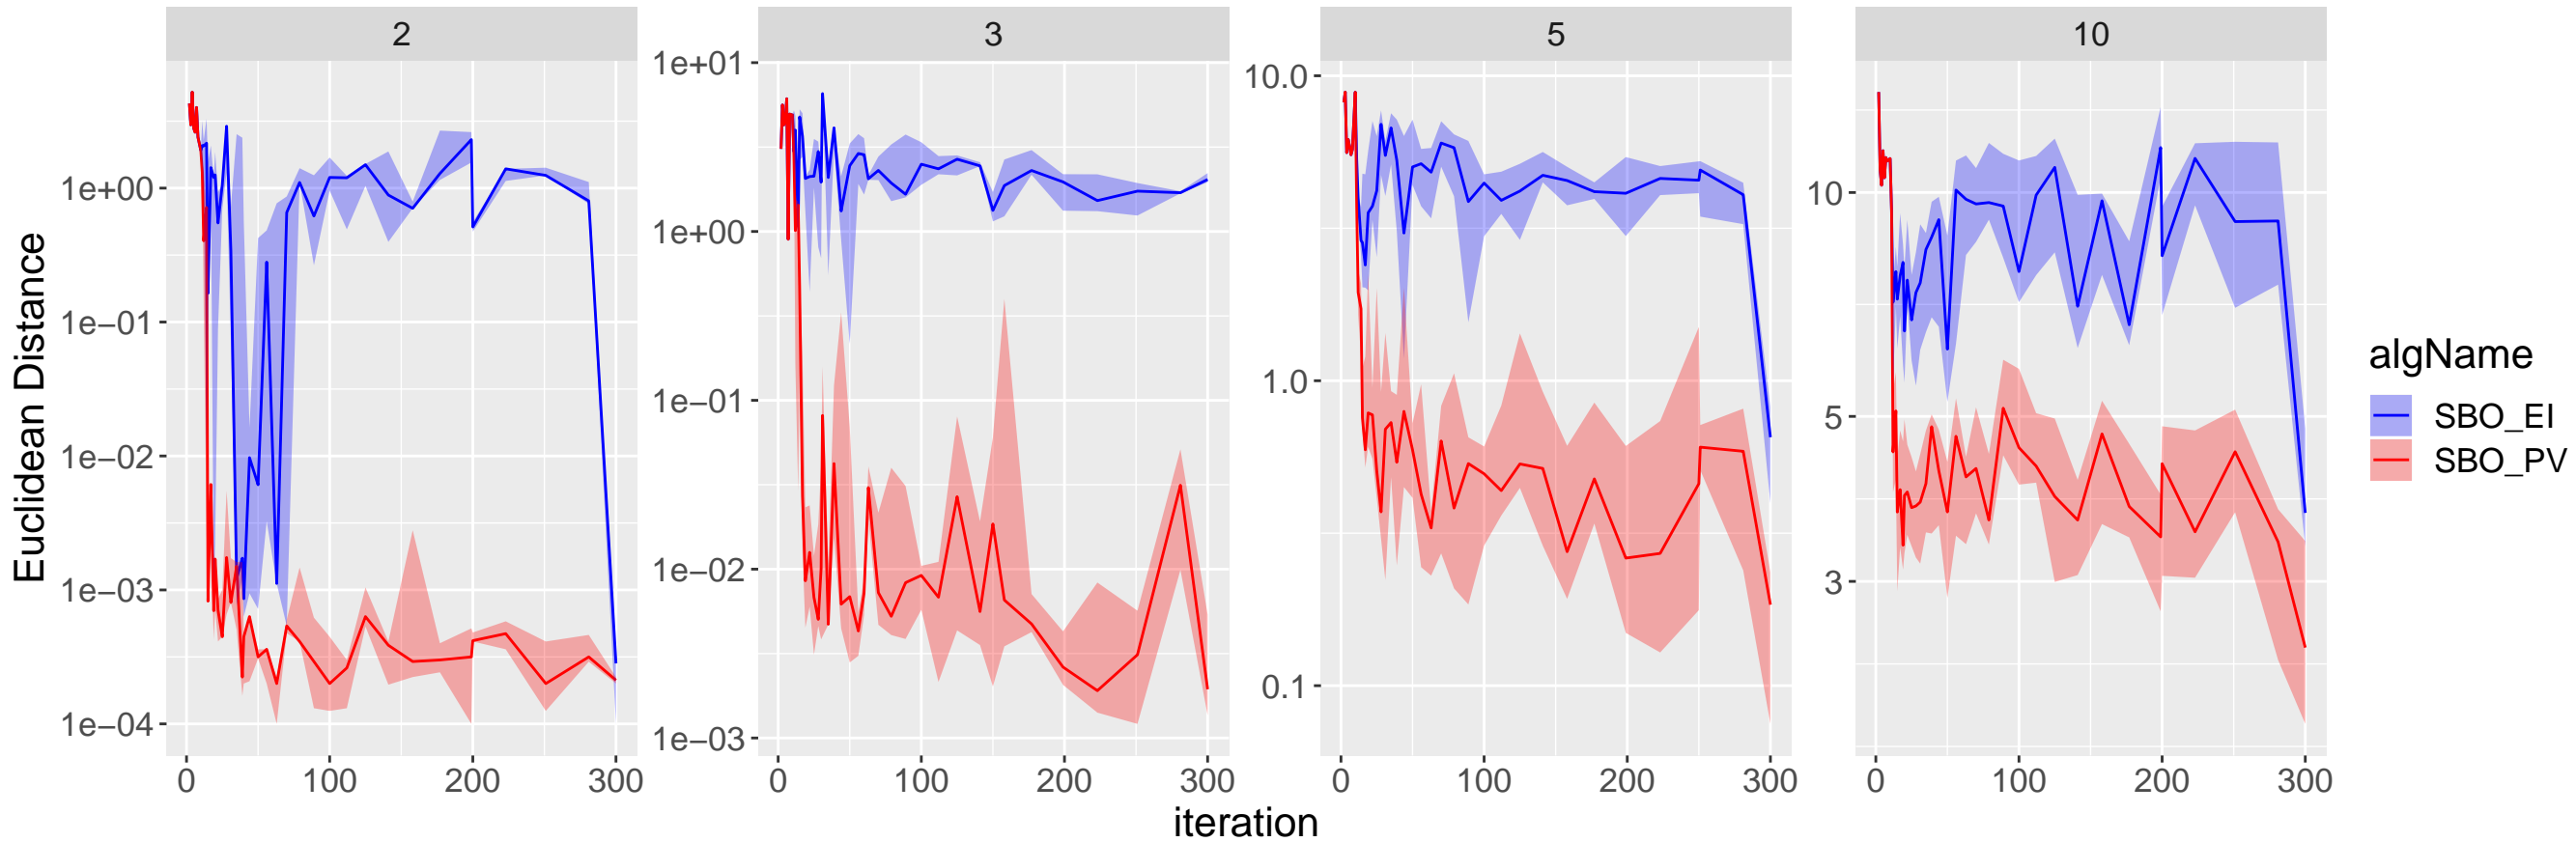

# Attractive Sector

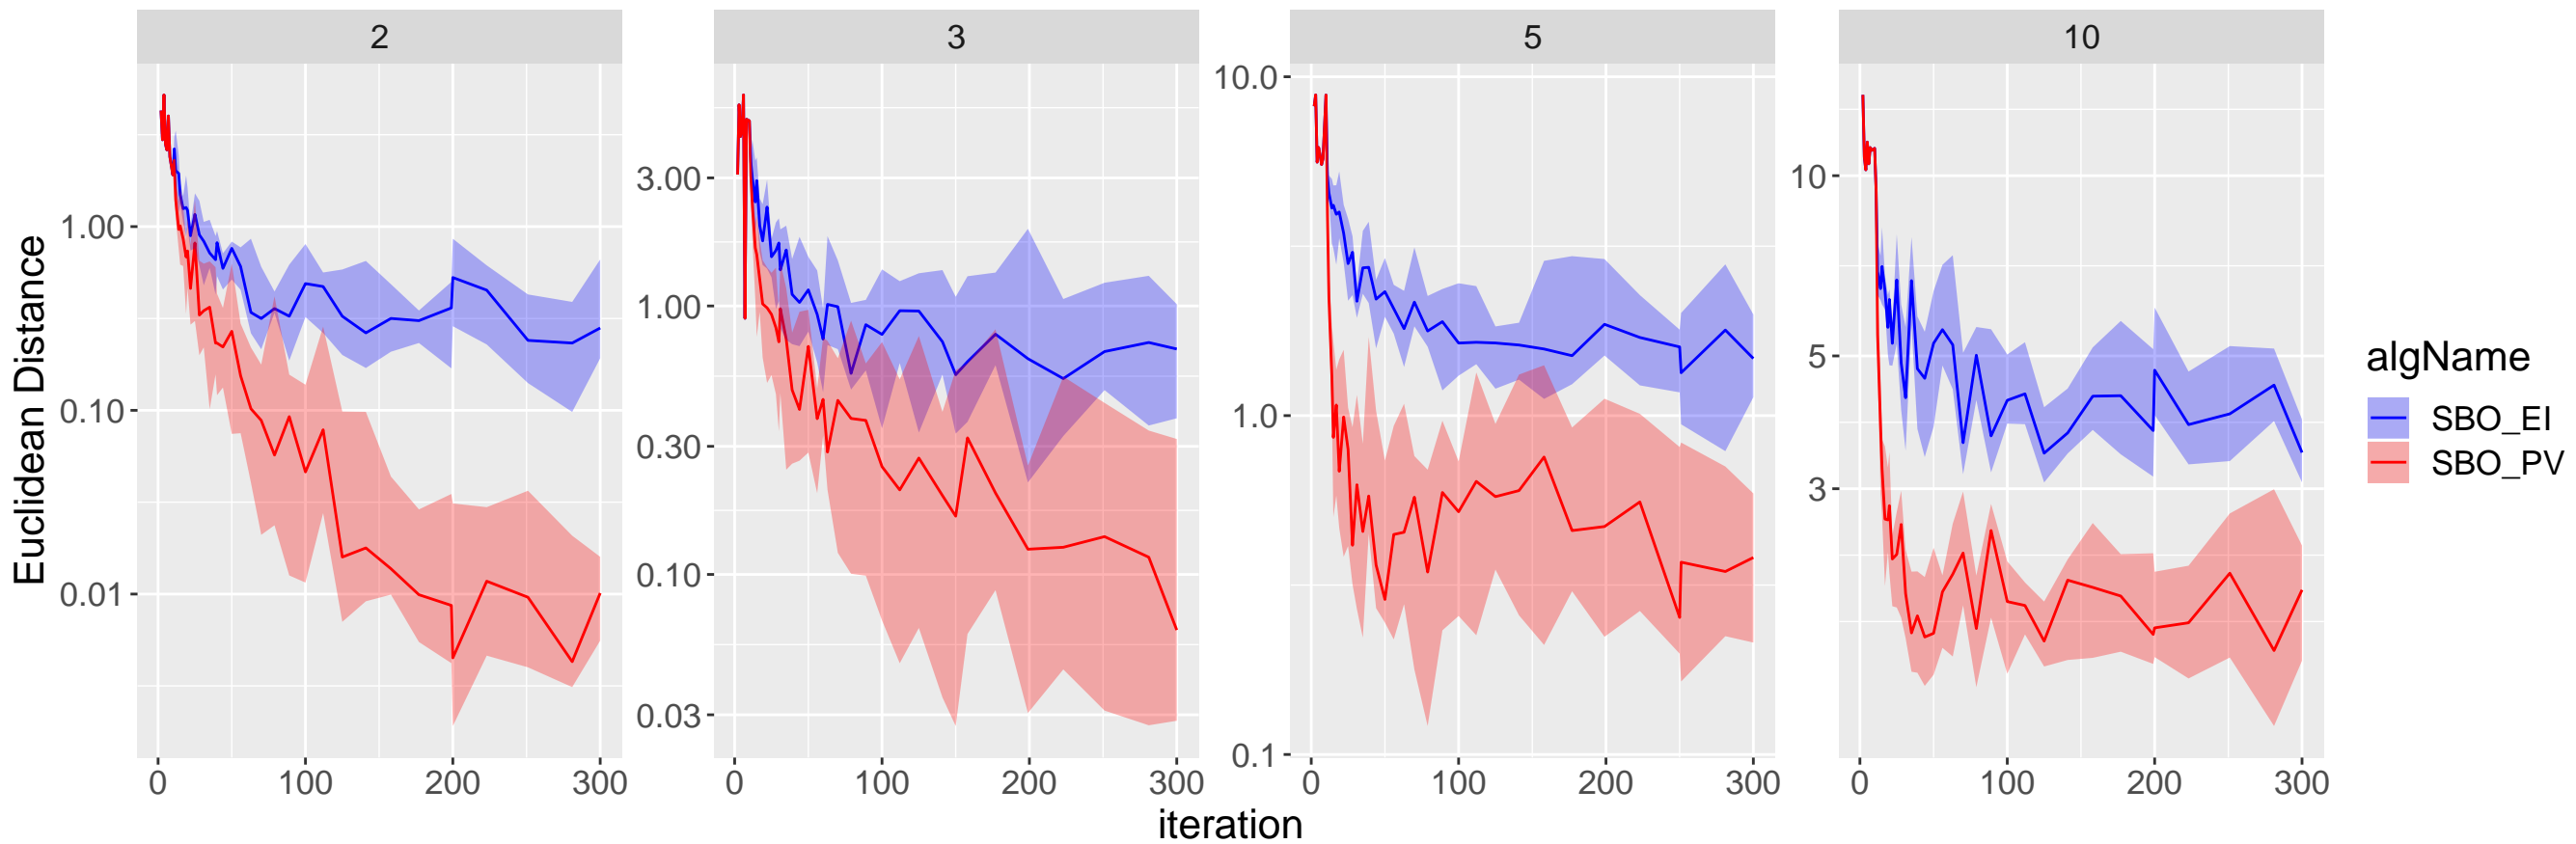

# Step Ellipsoidal

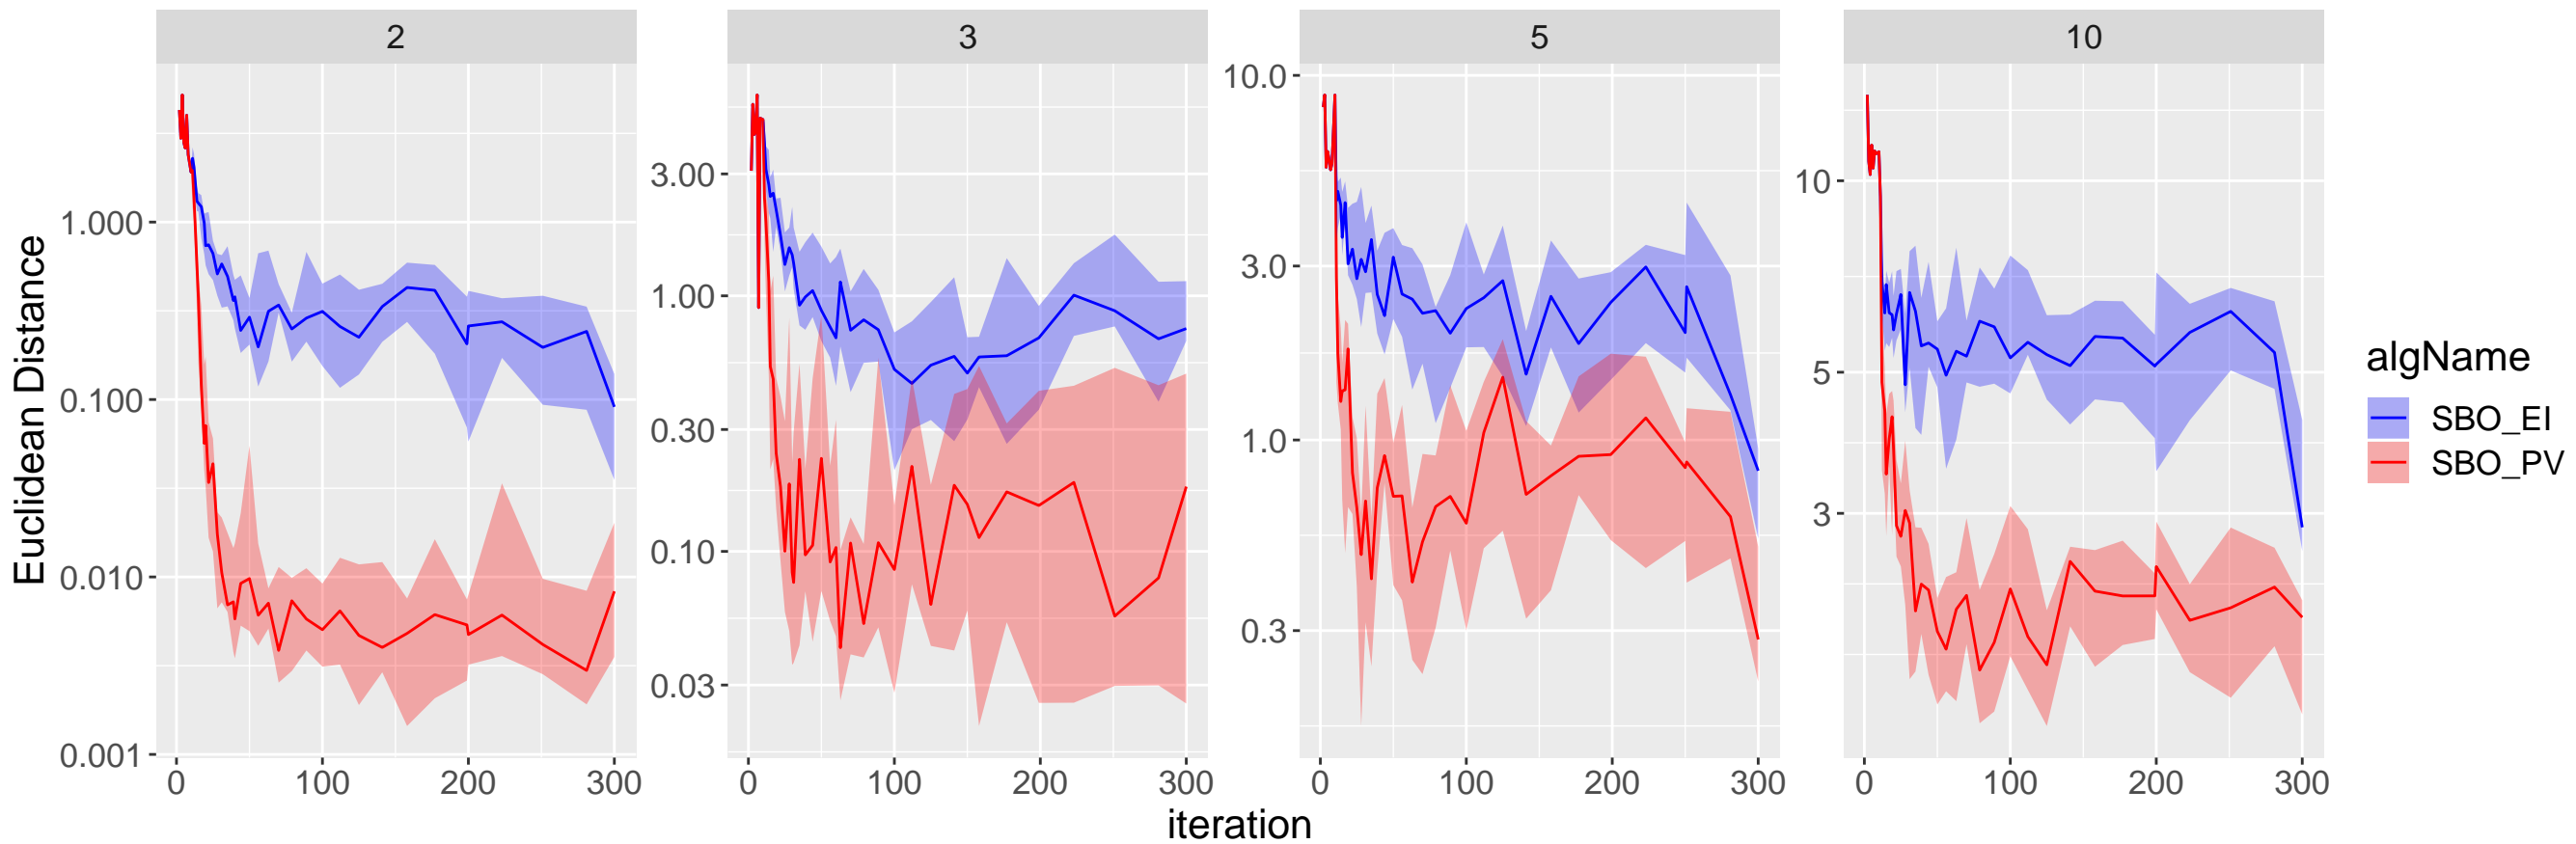

# Rosenbrock

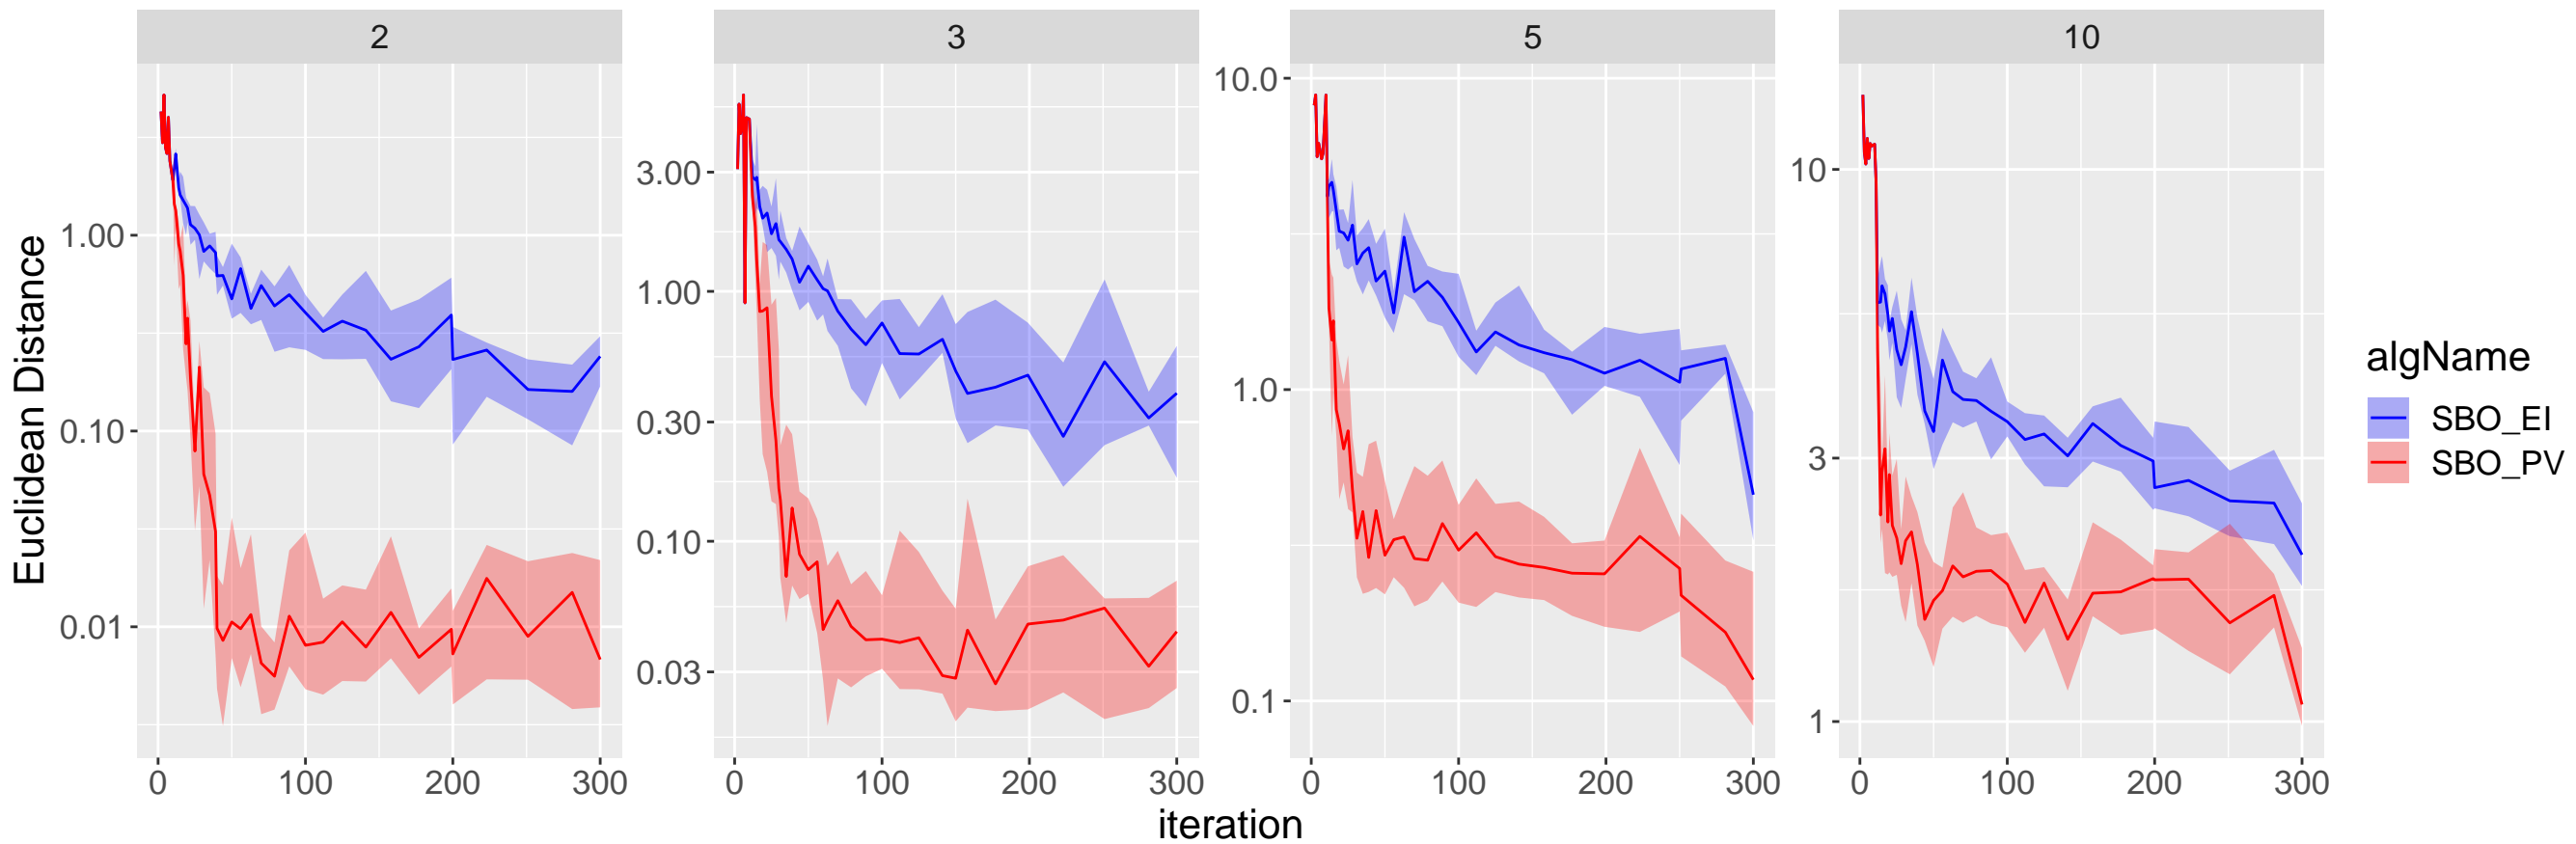



# Rosenbrock, rotated

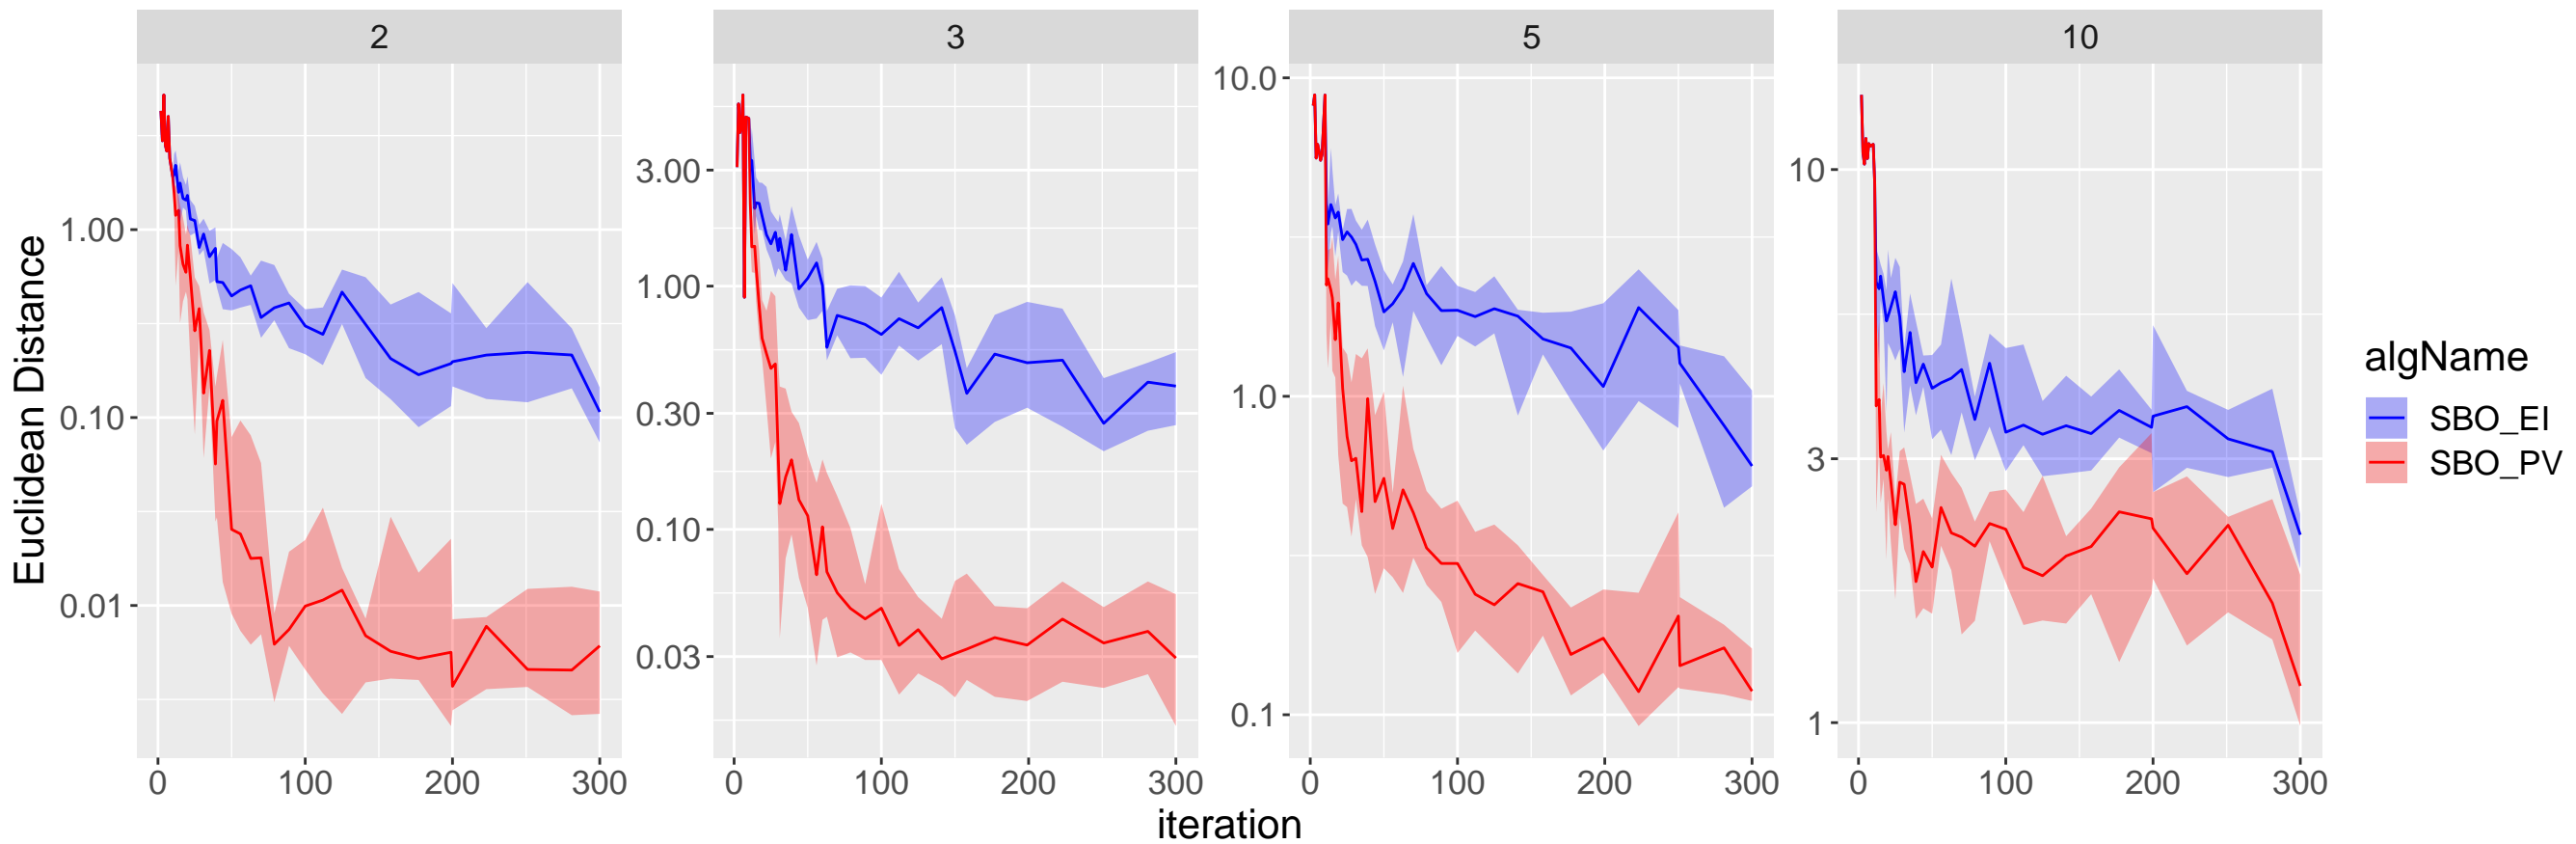

# Ellipsoidal

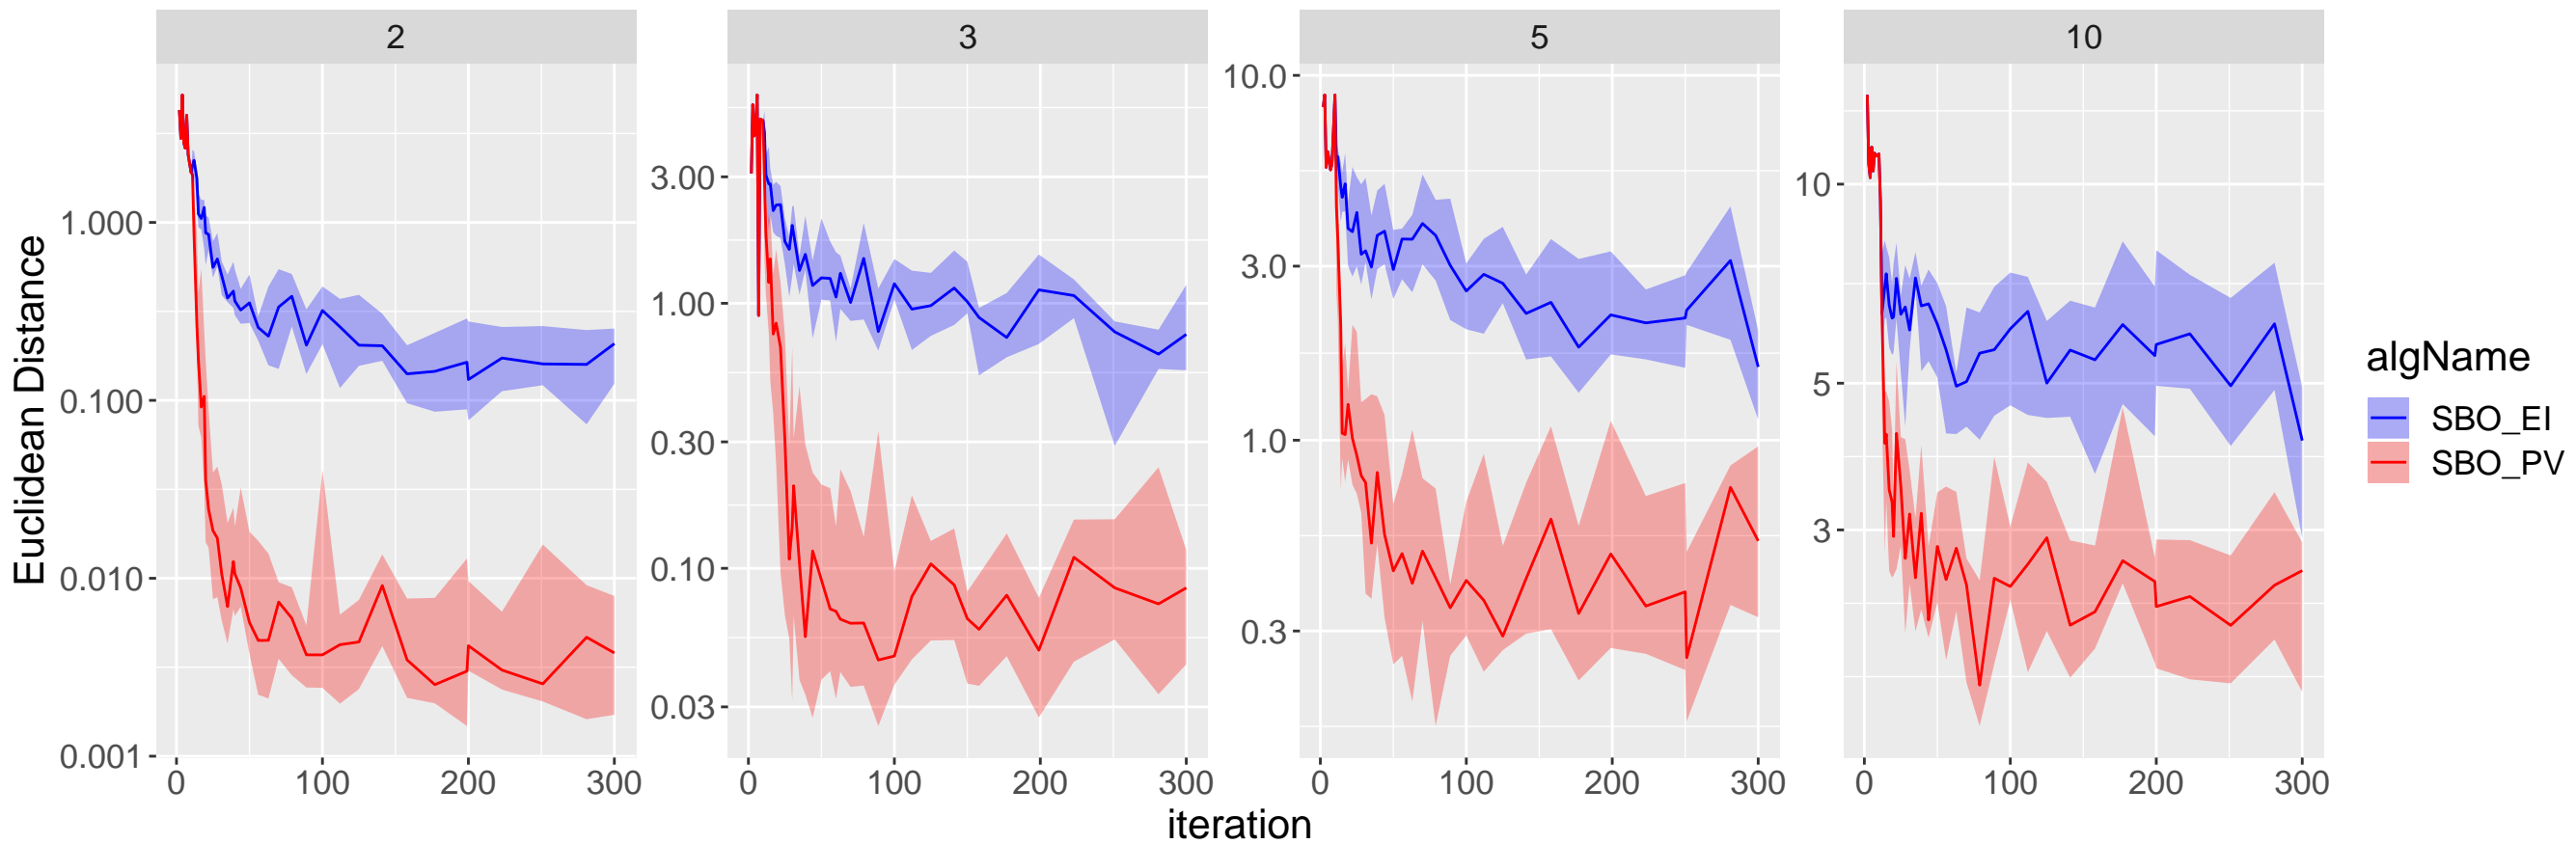

# Discus

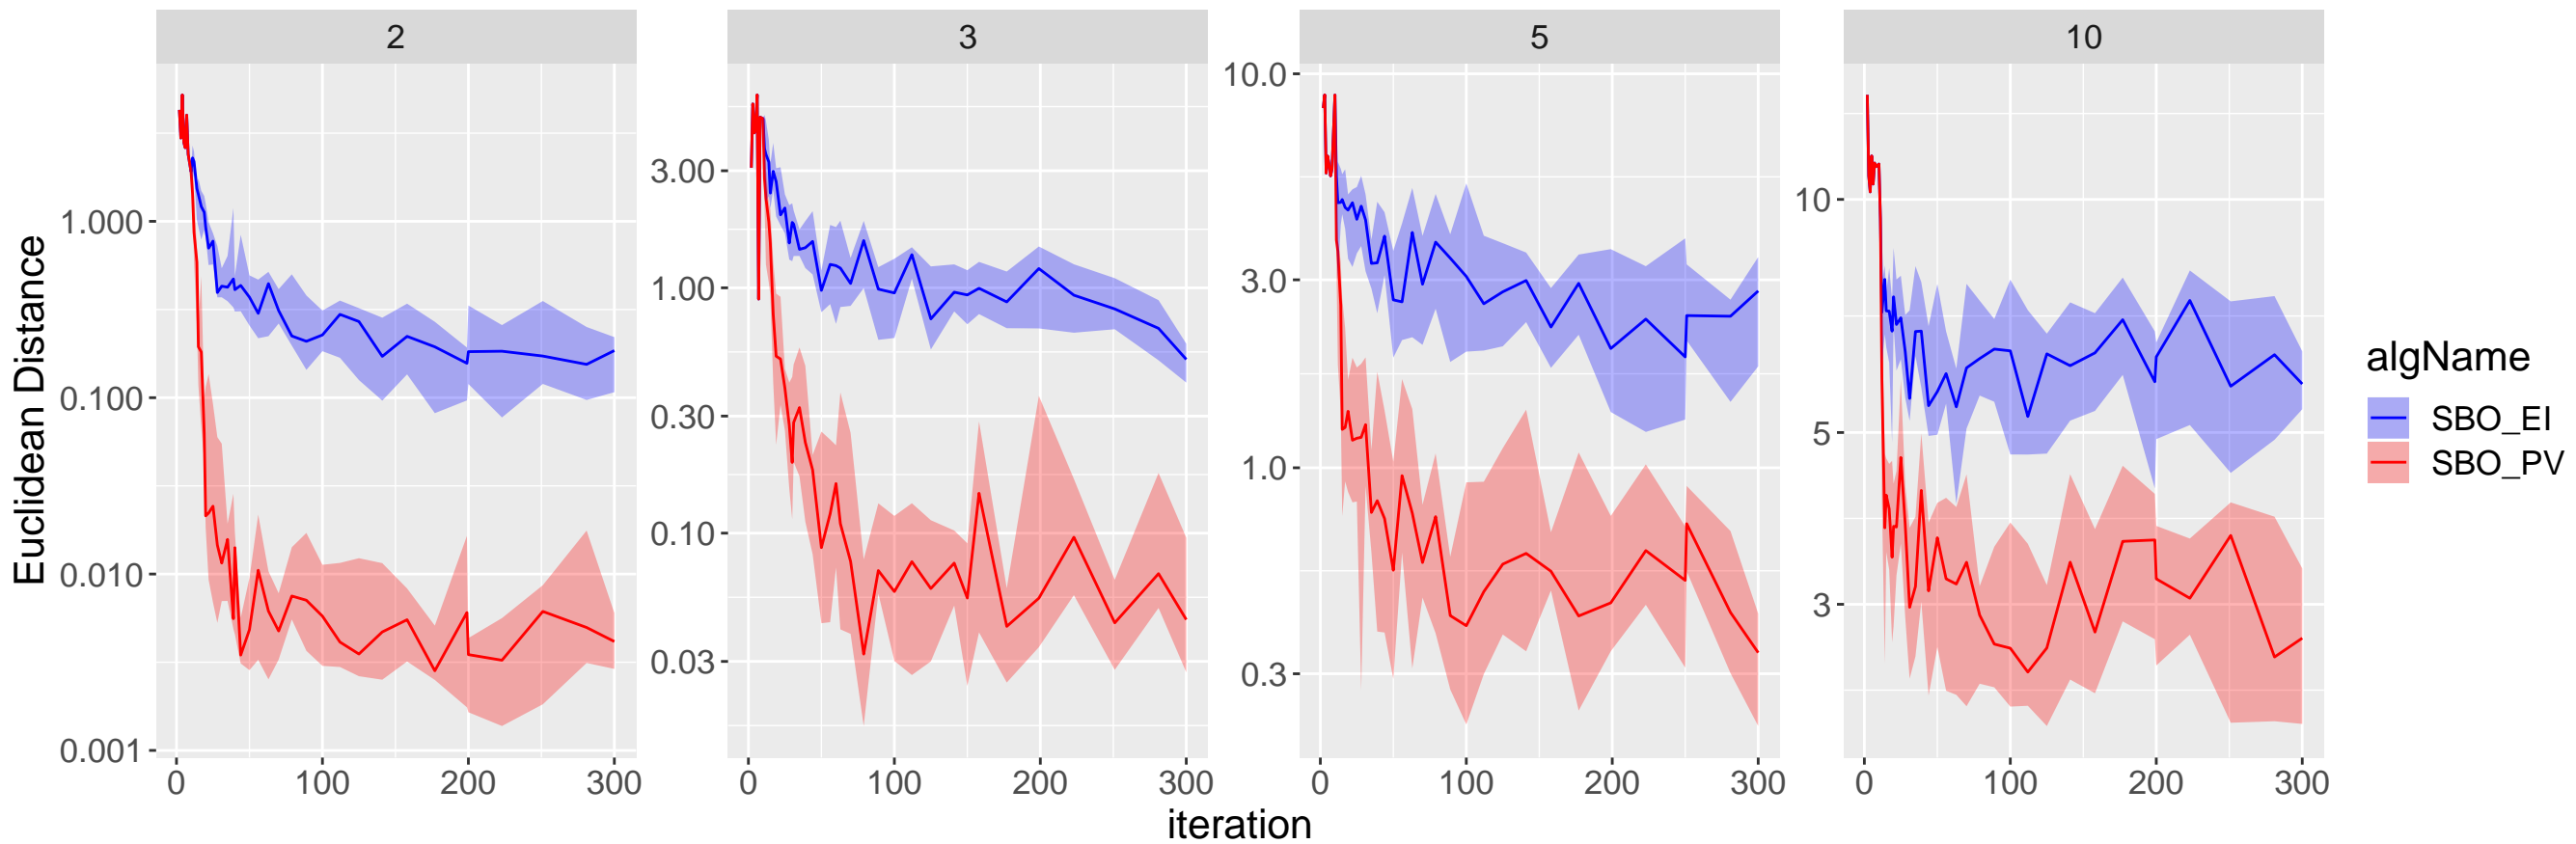

# Bent Cigar

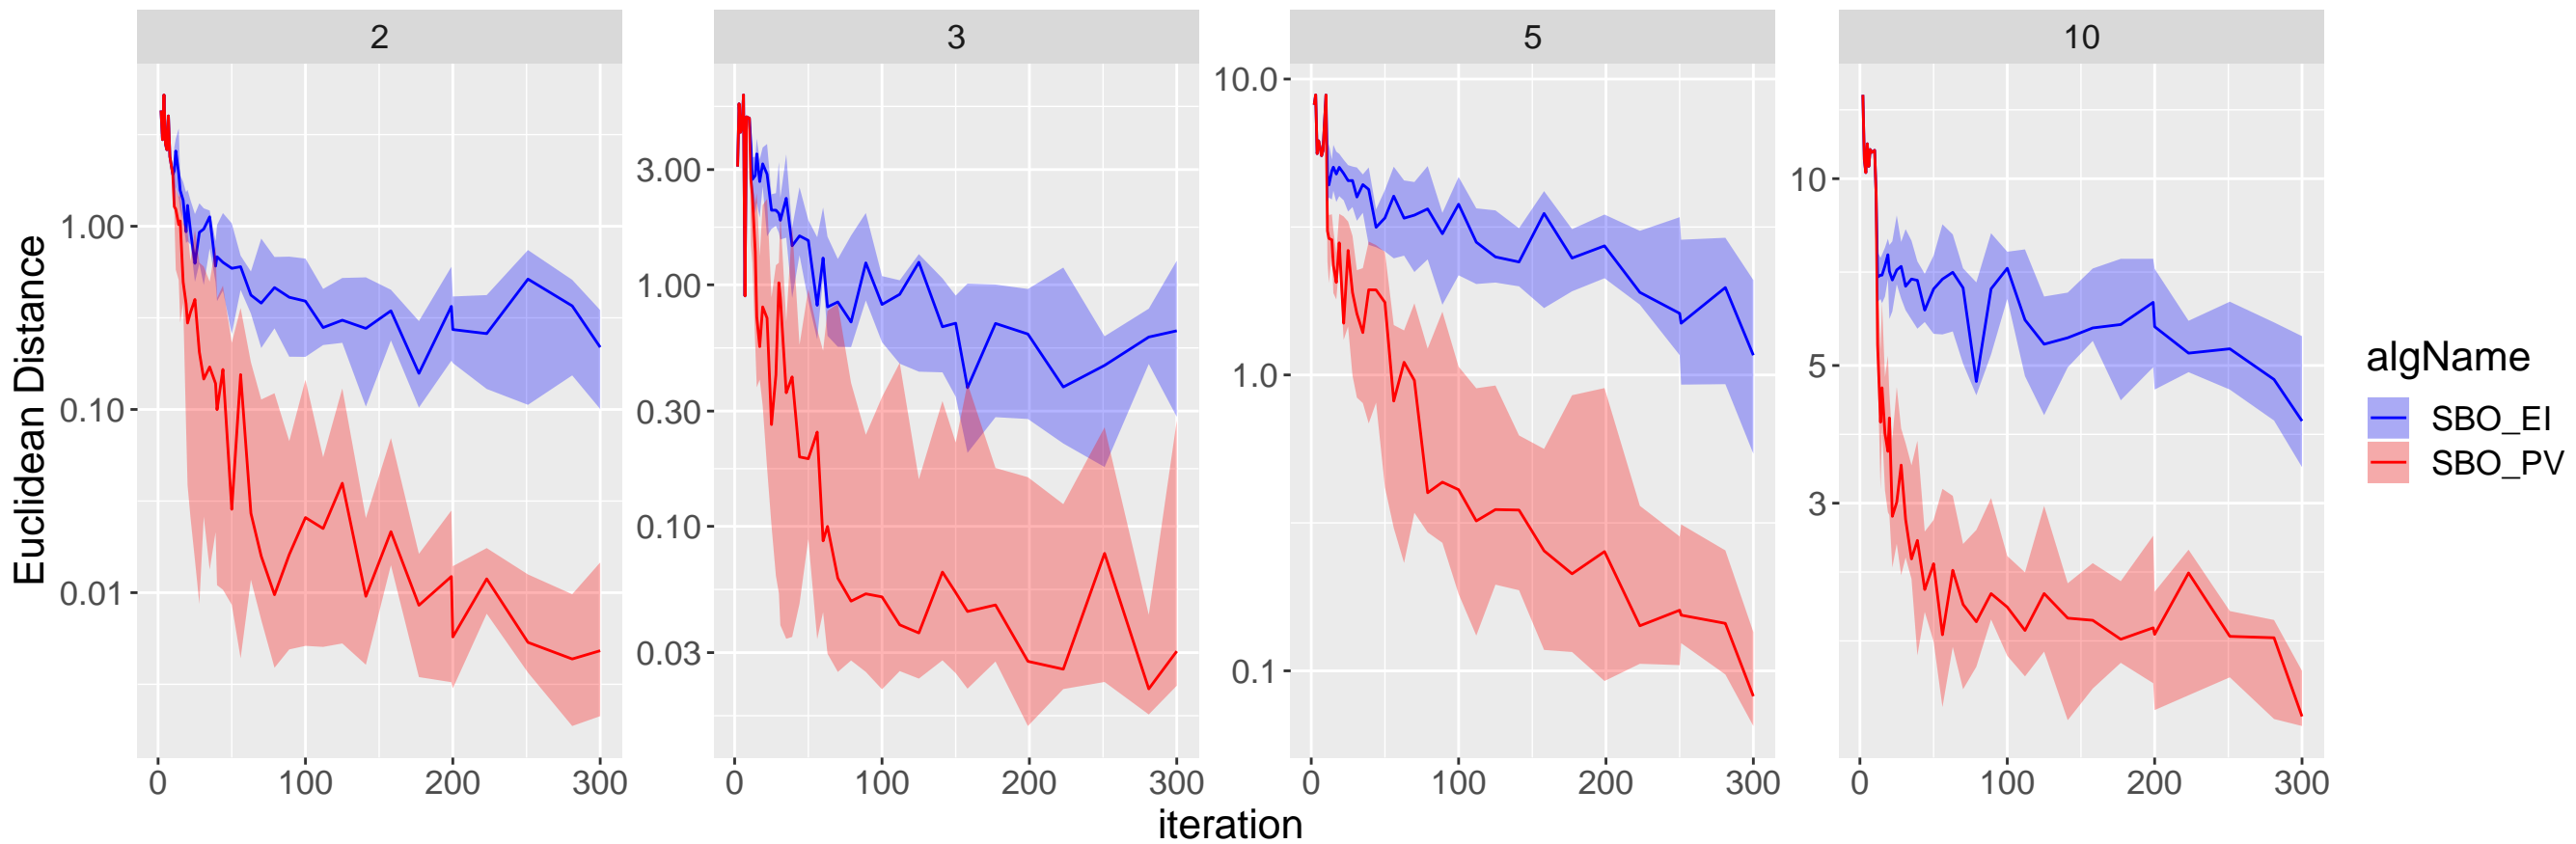

# Sharp Ridge

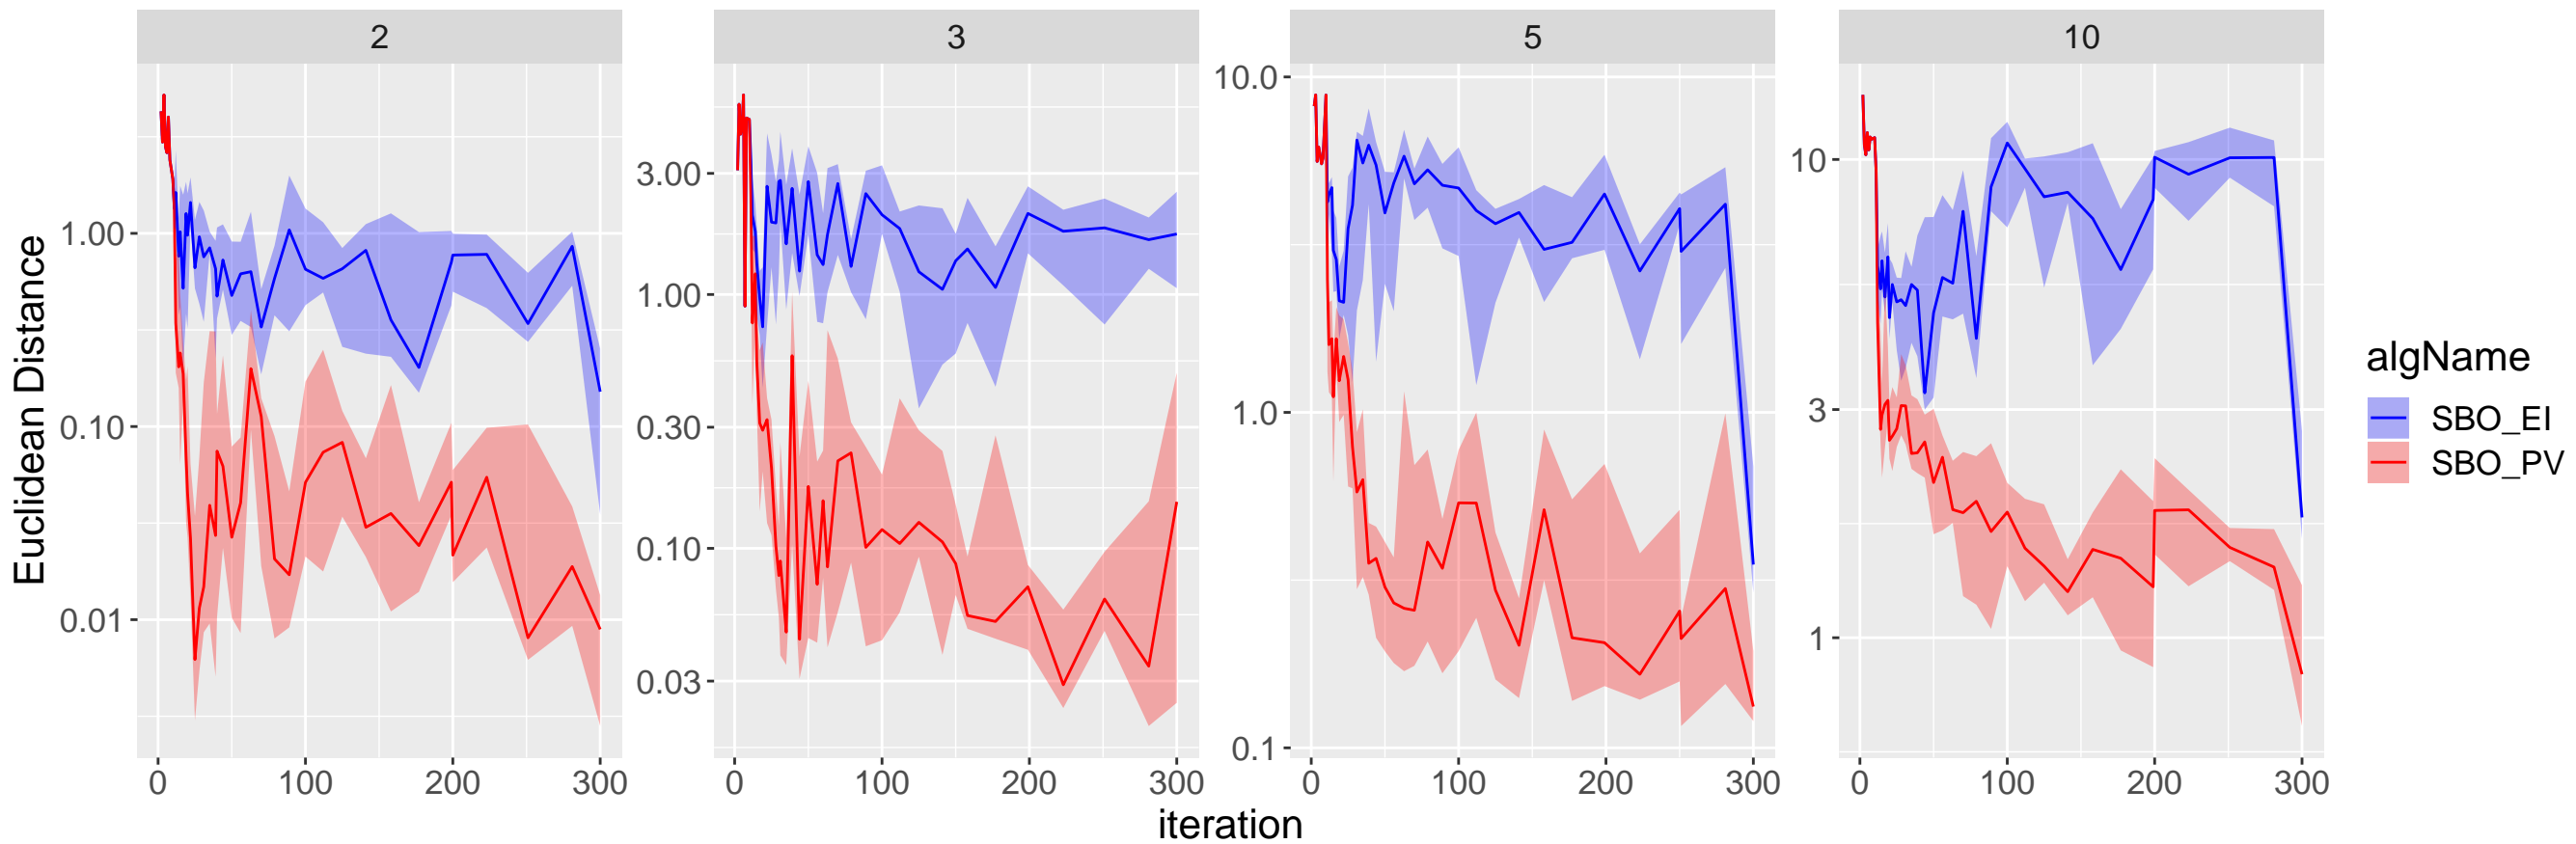

# Different Powers

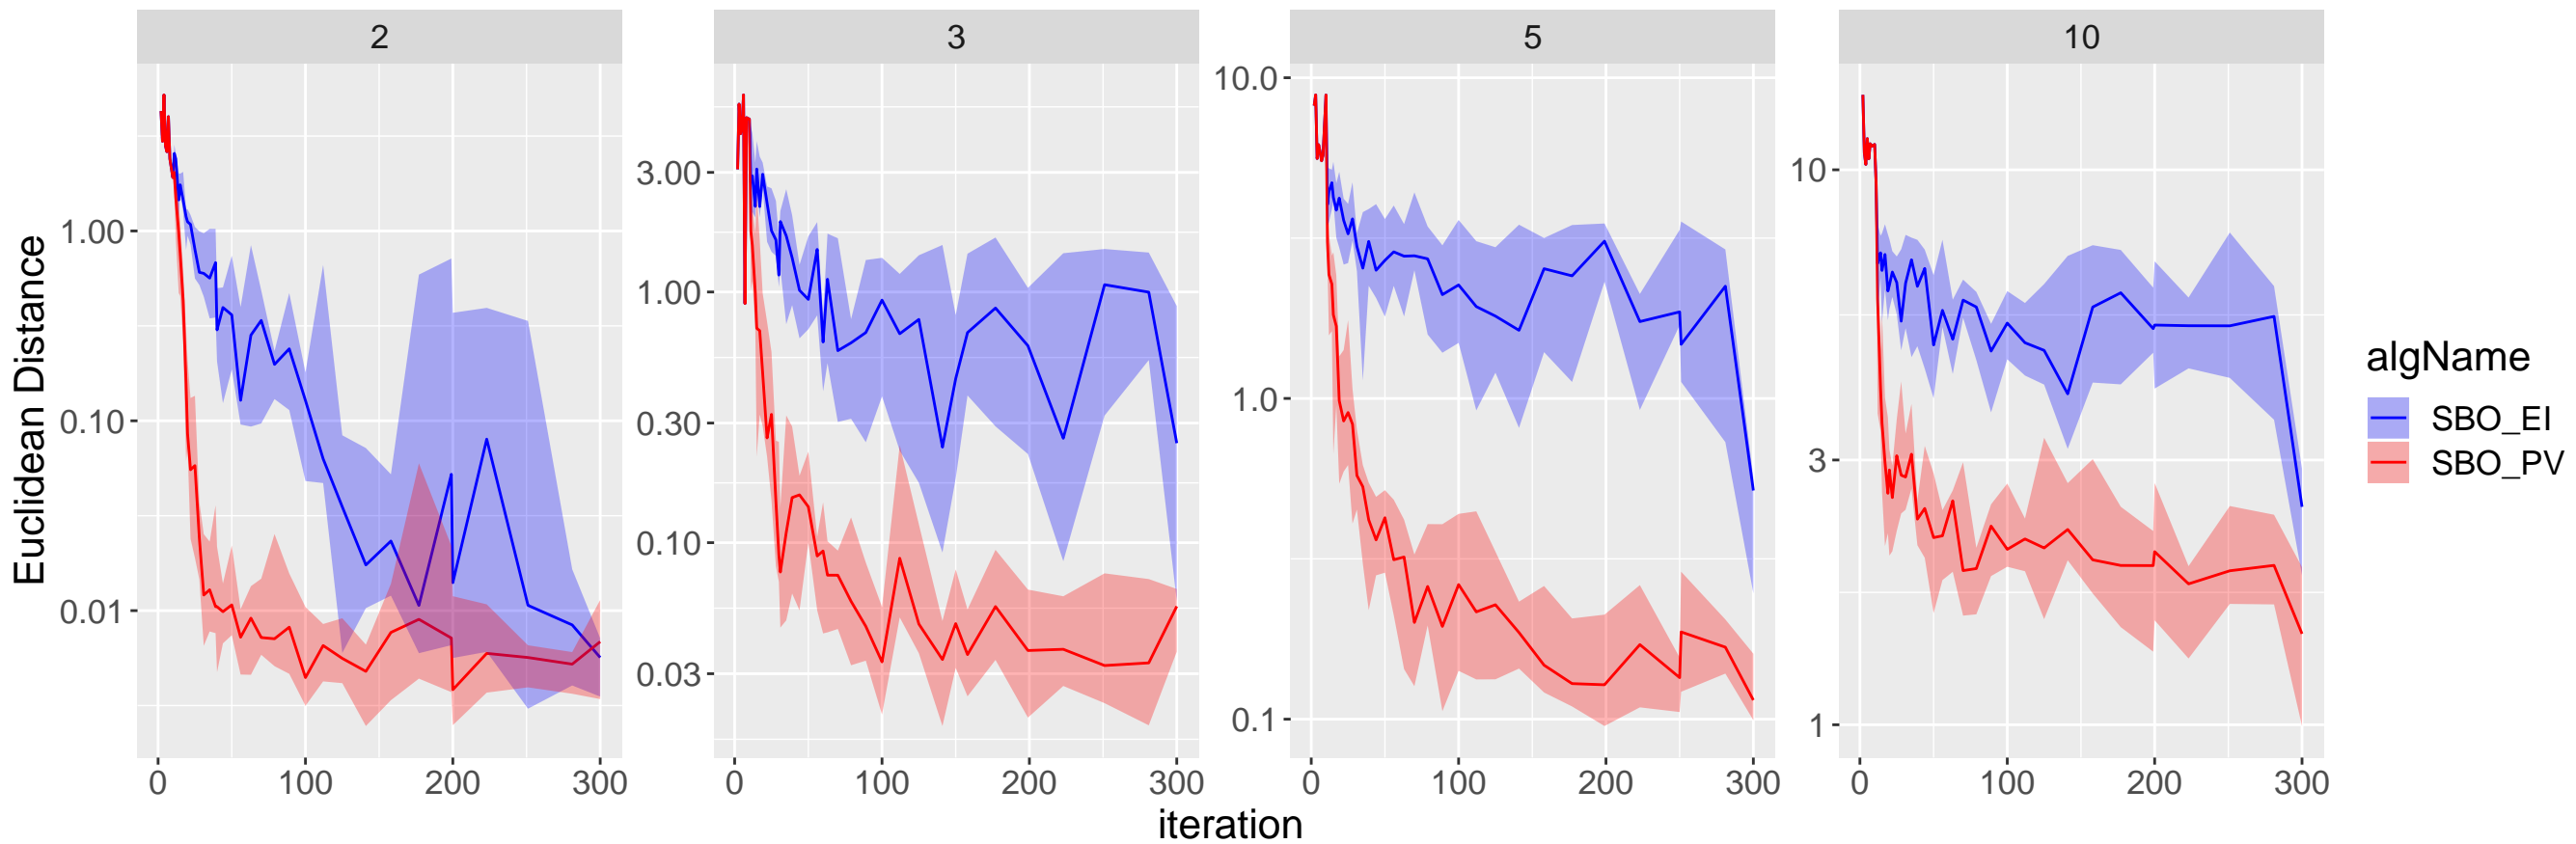

# Rastrigin

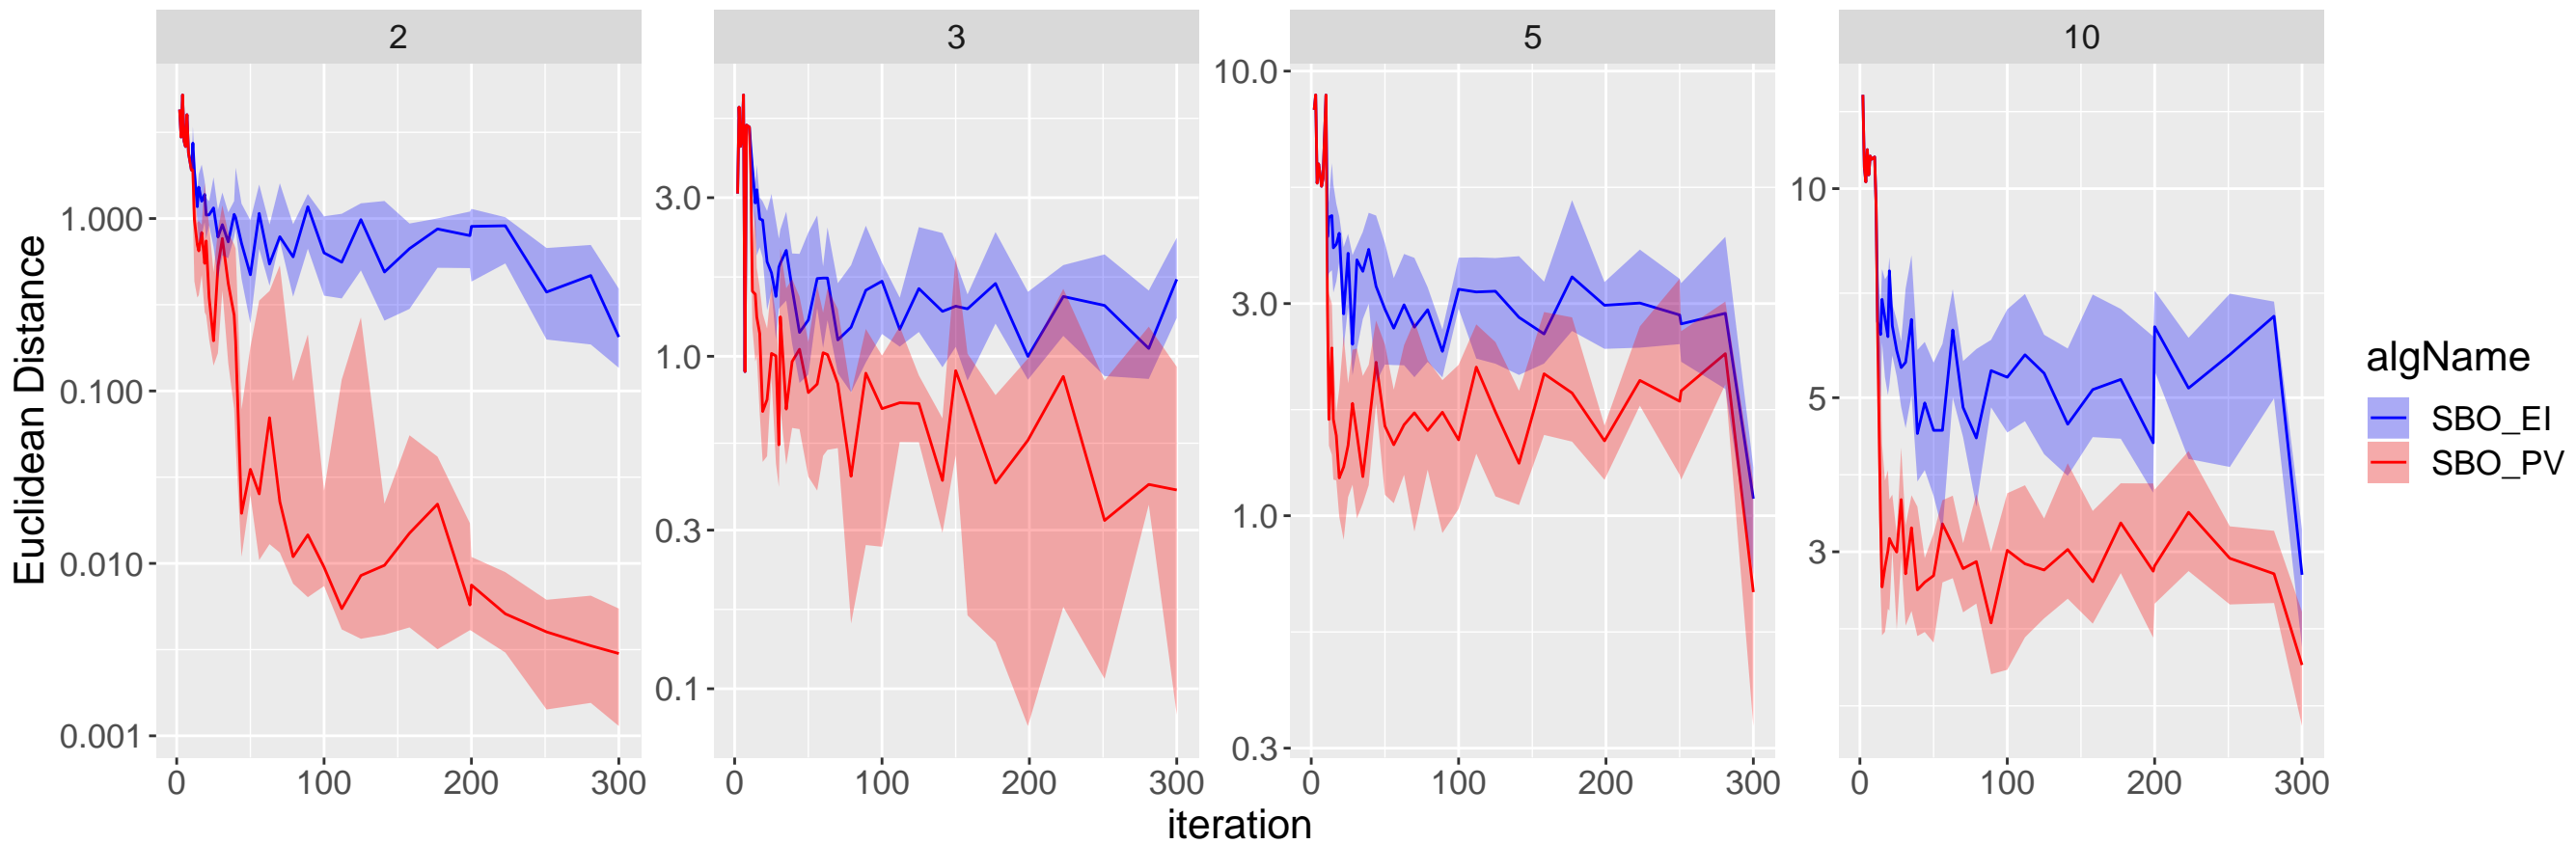

# Weierstrass

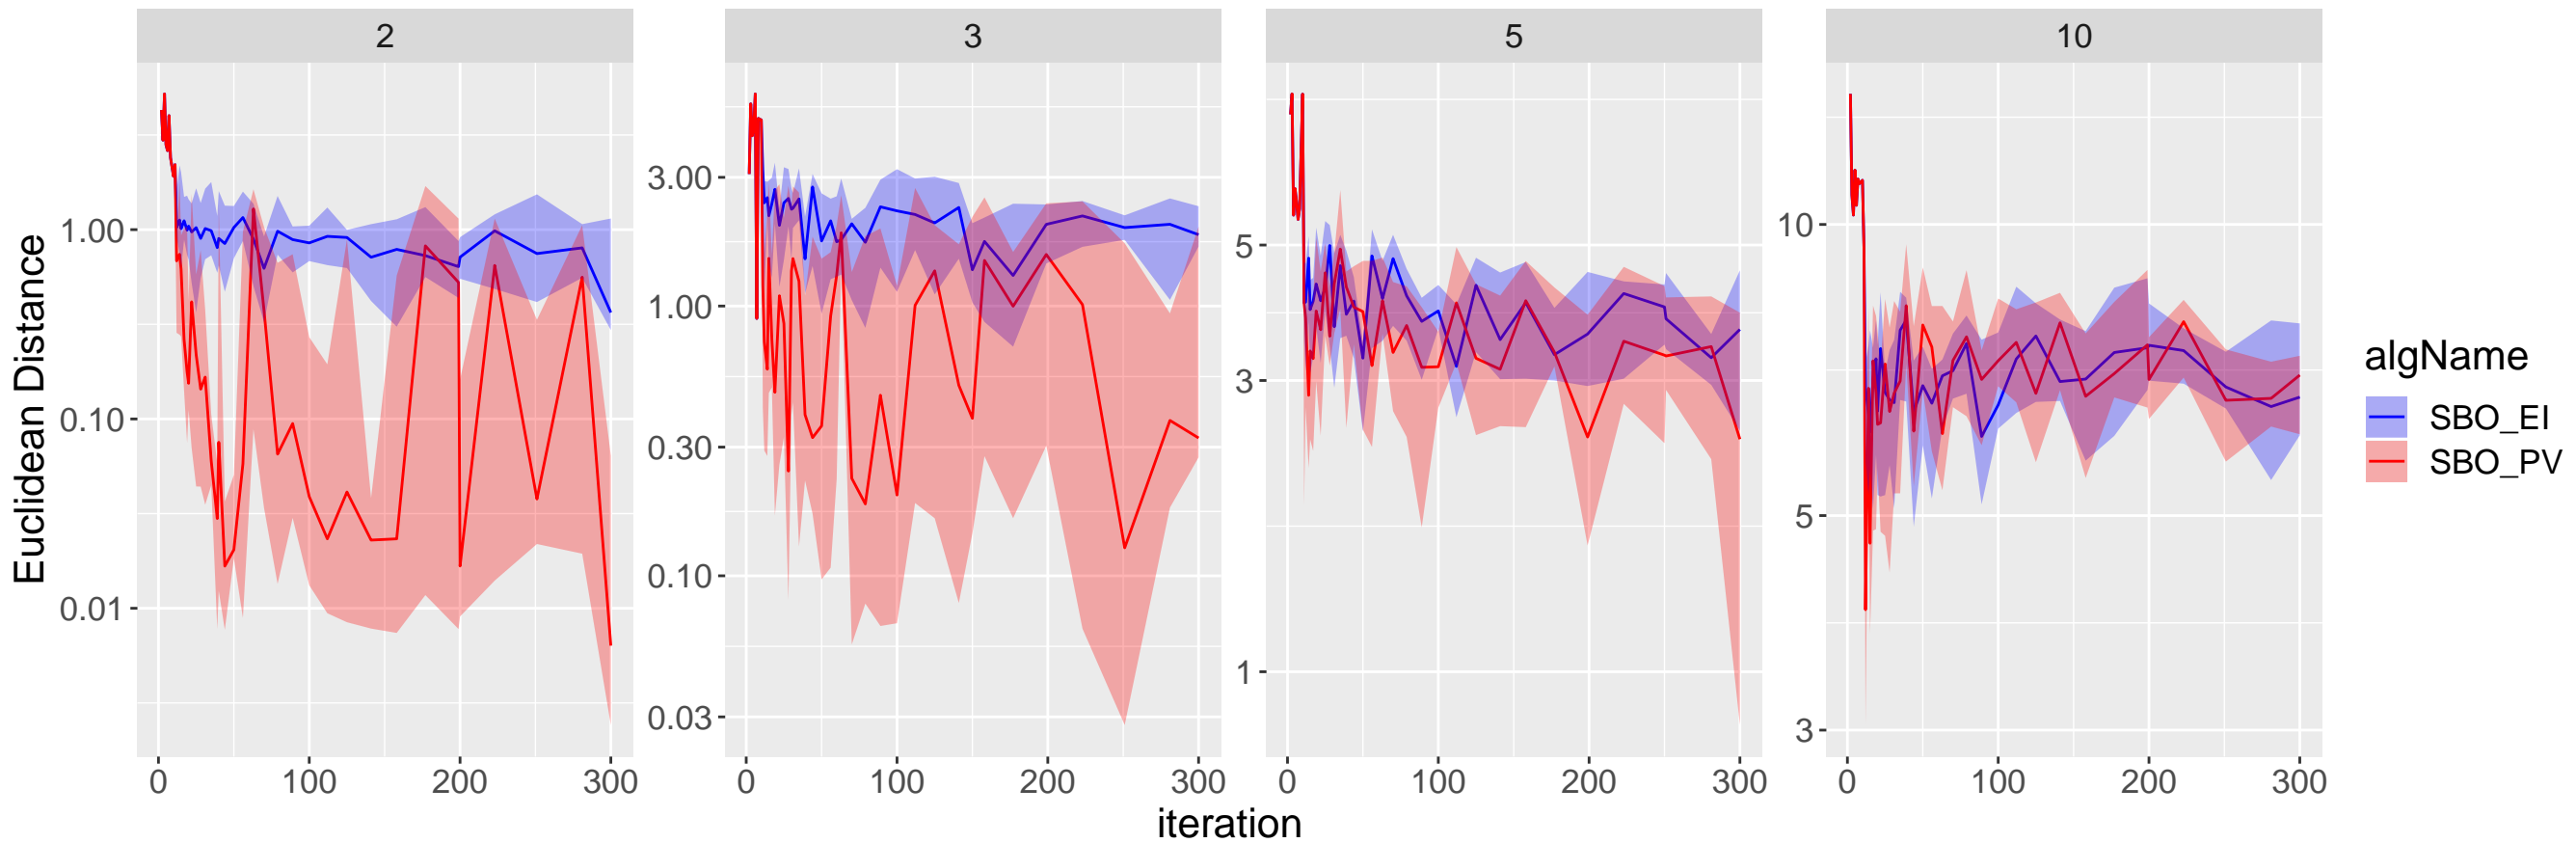



# Schaffers F7

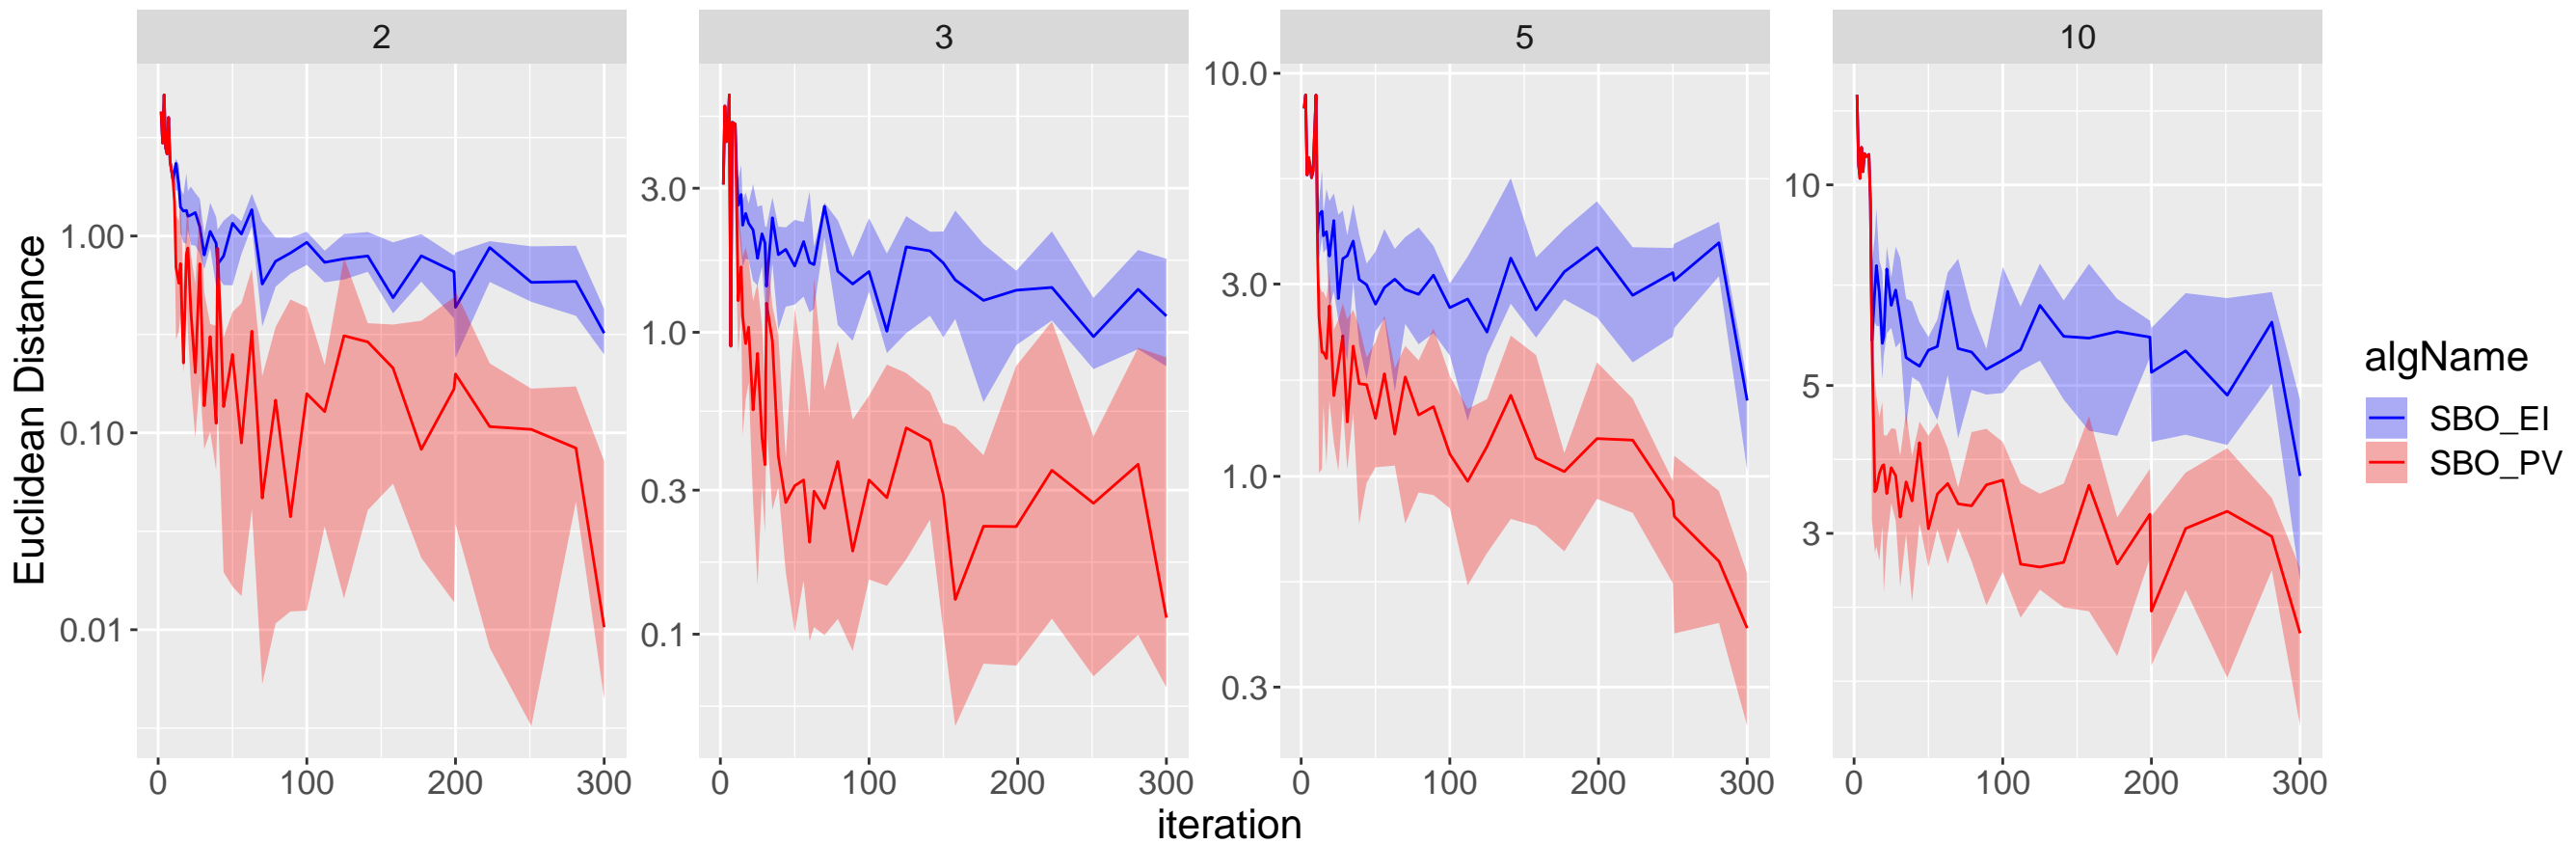

# Schaffers F7

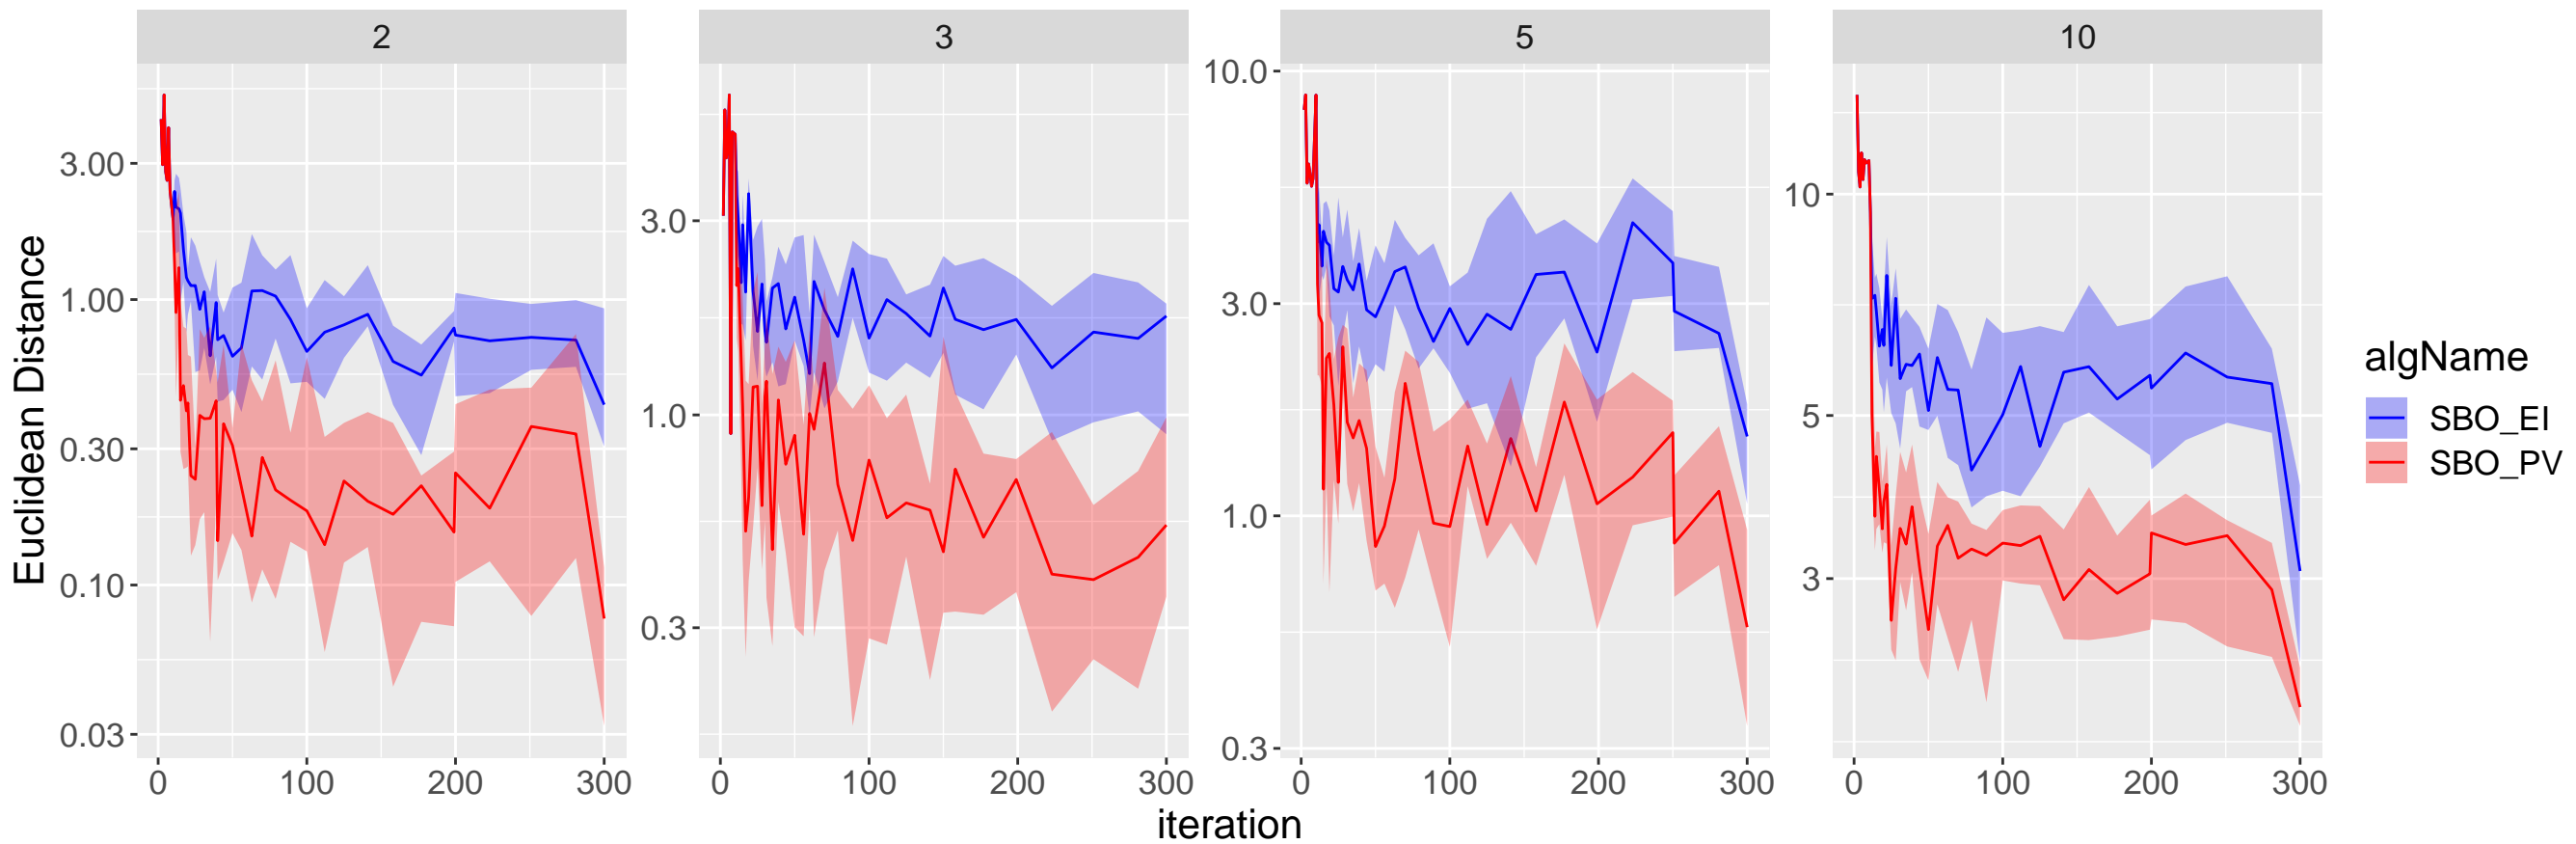

# Griwank-Rosenbrock

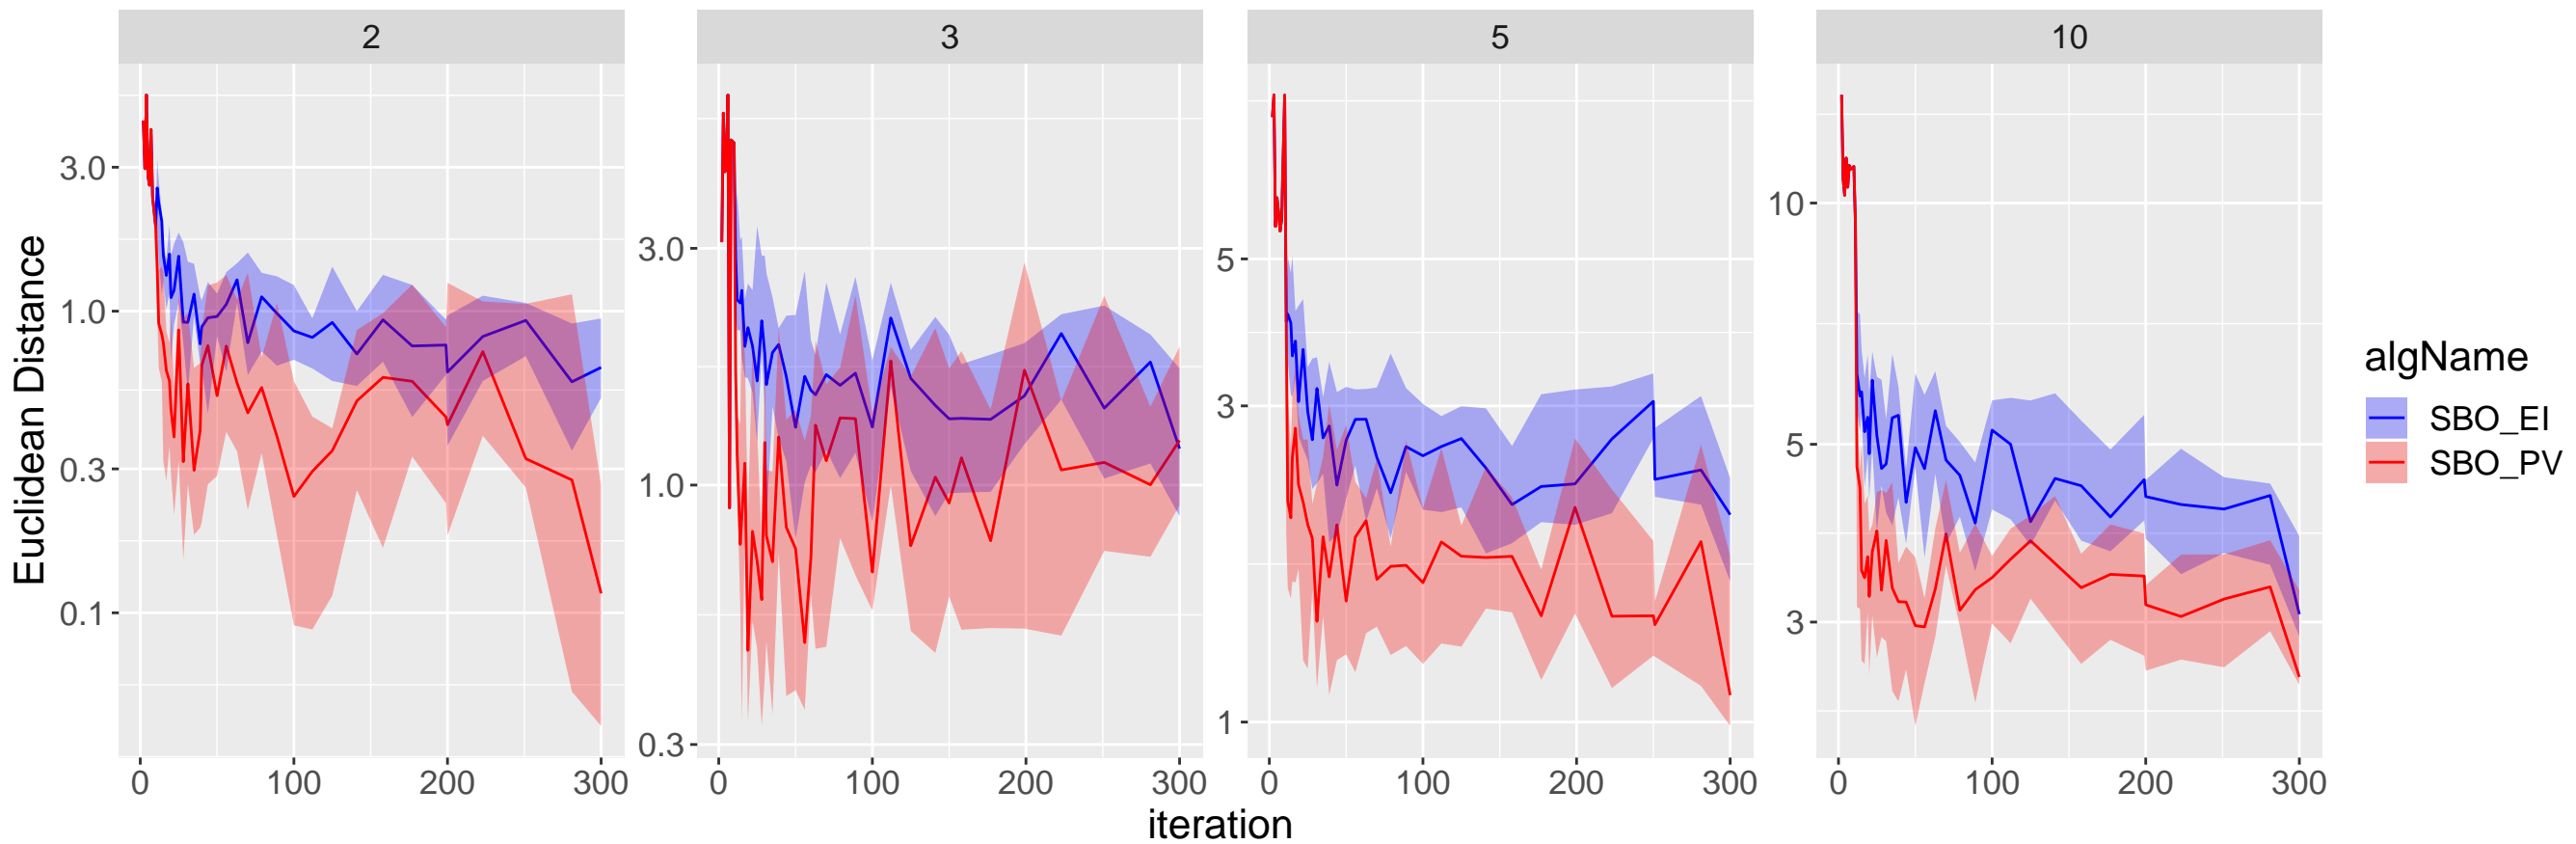

# Schwefel

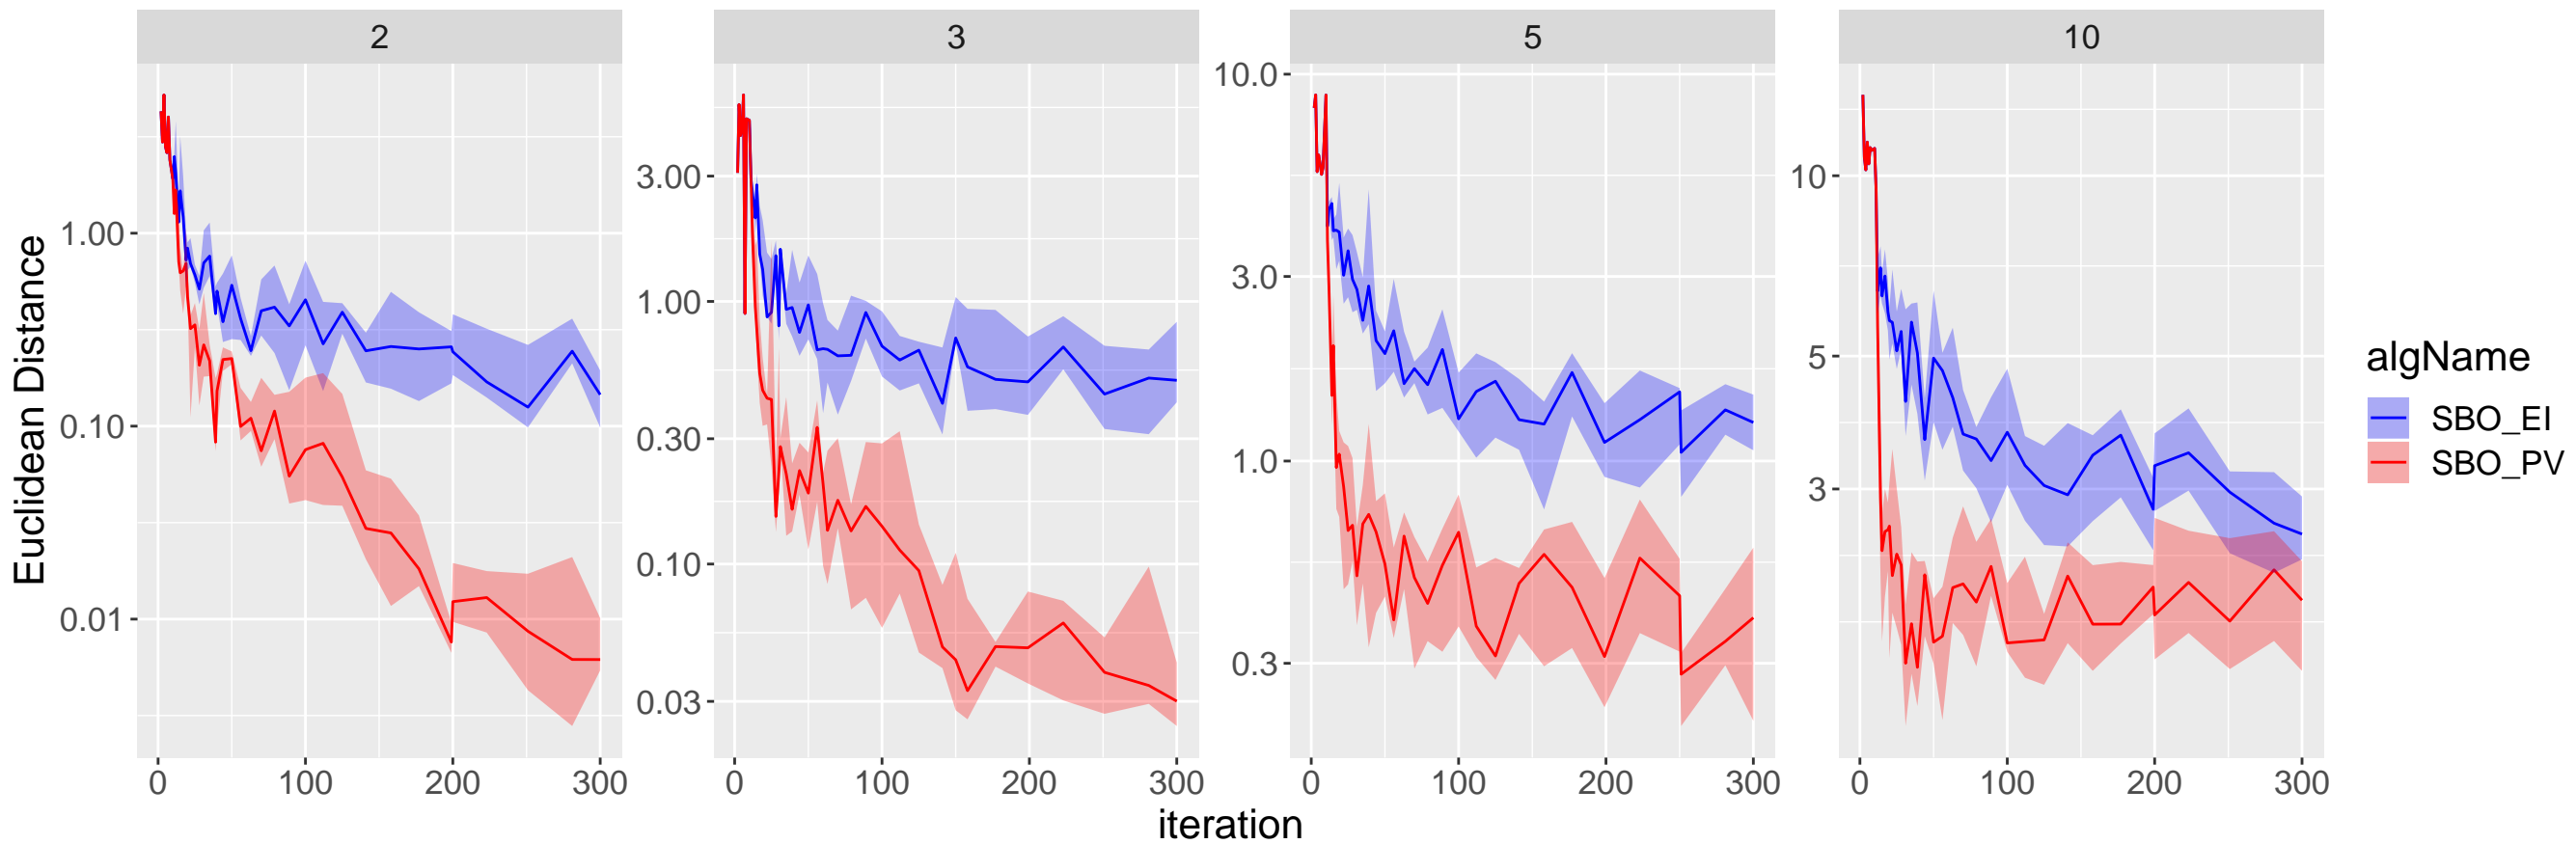

# Gallagher Gaussian 101-me Peaks

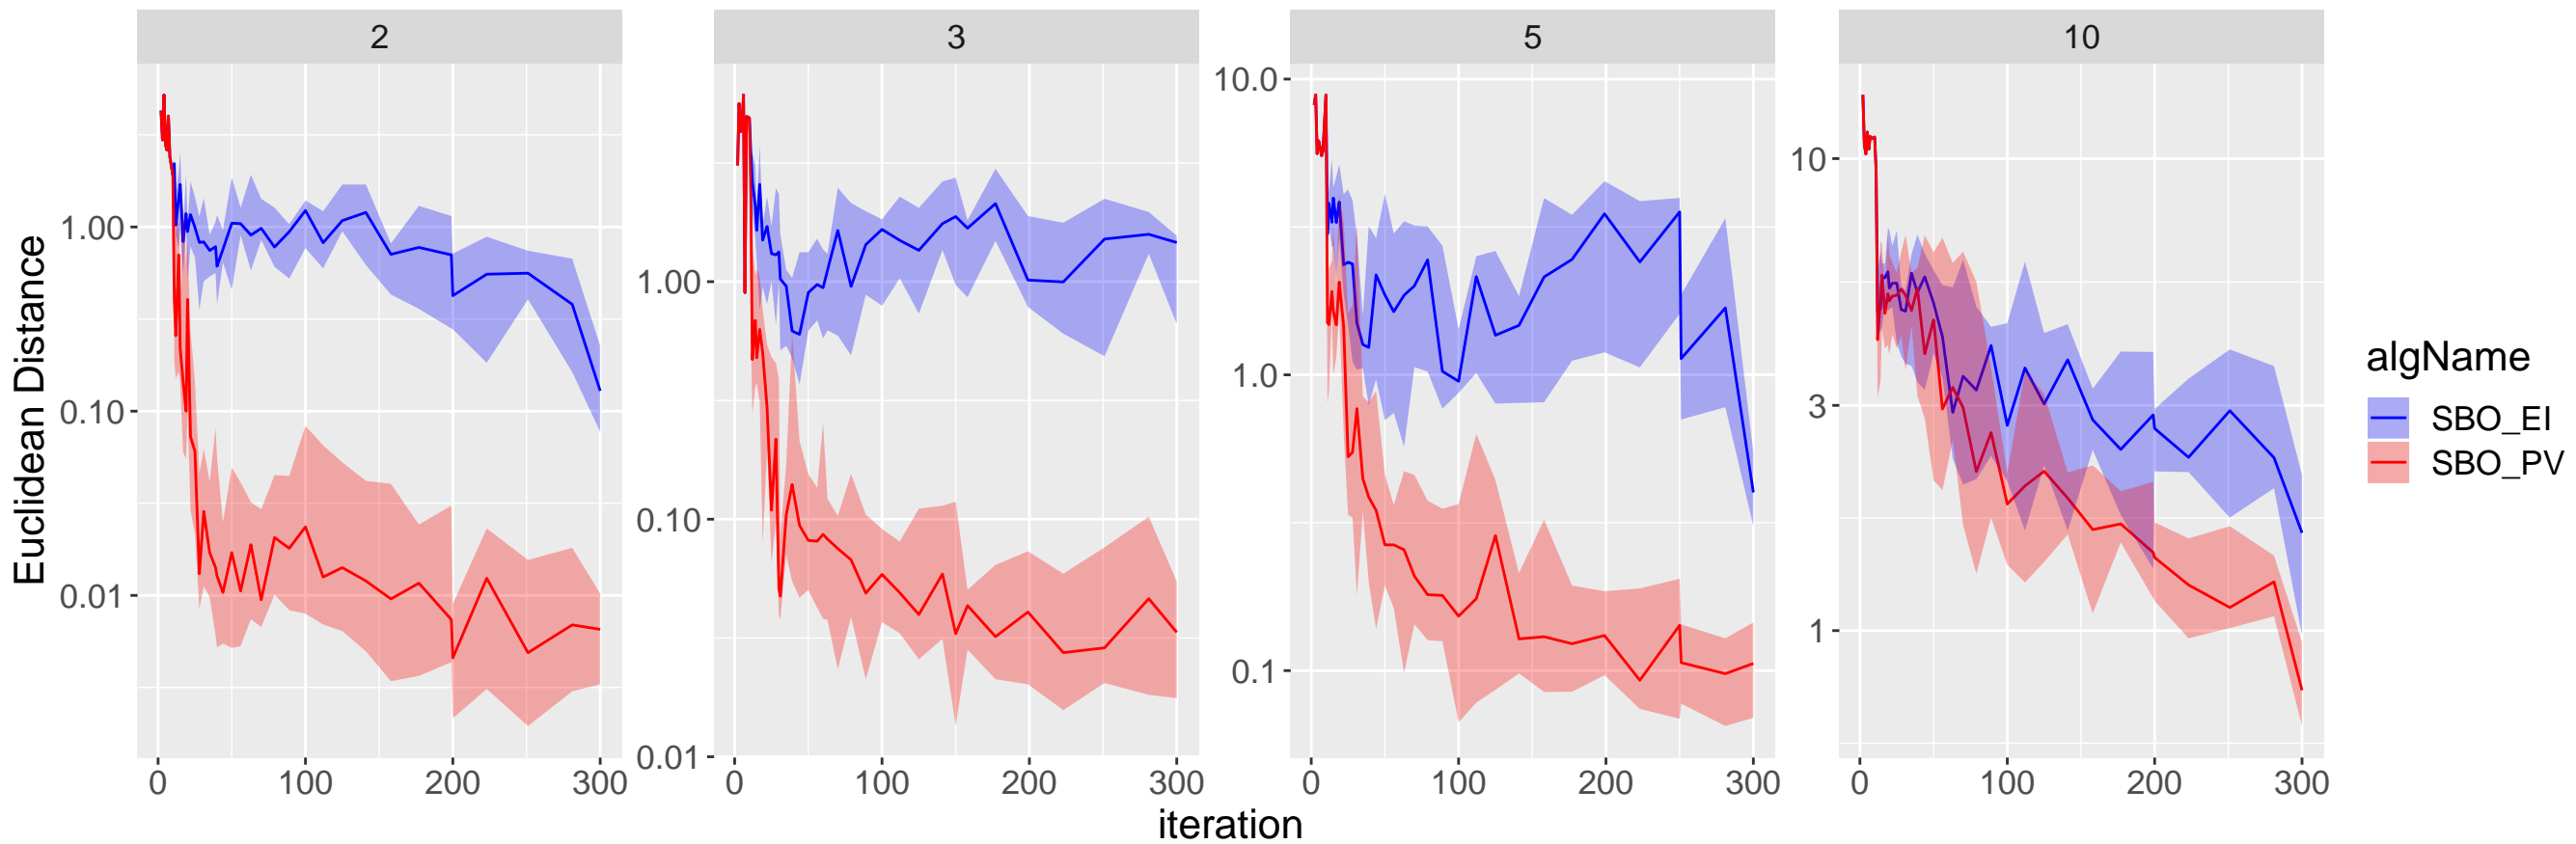

# Gallagher Gaussian 21-hi Peaks

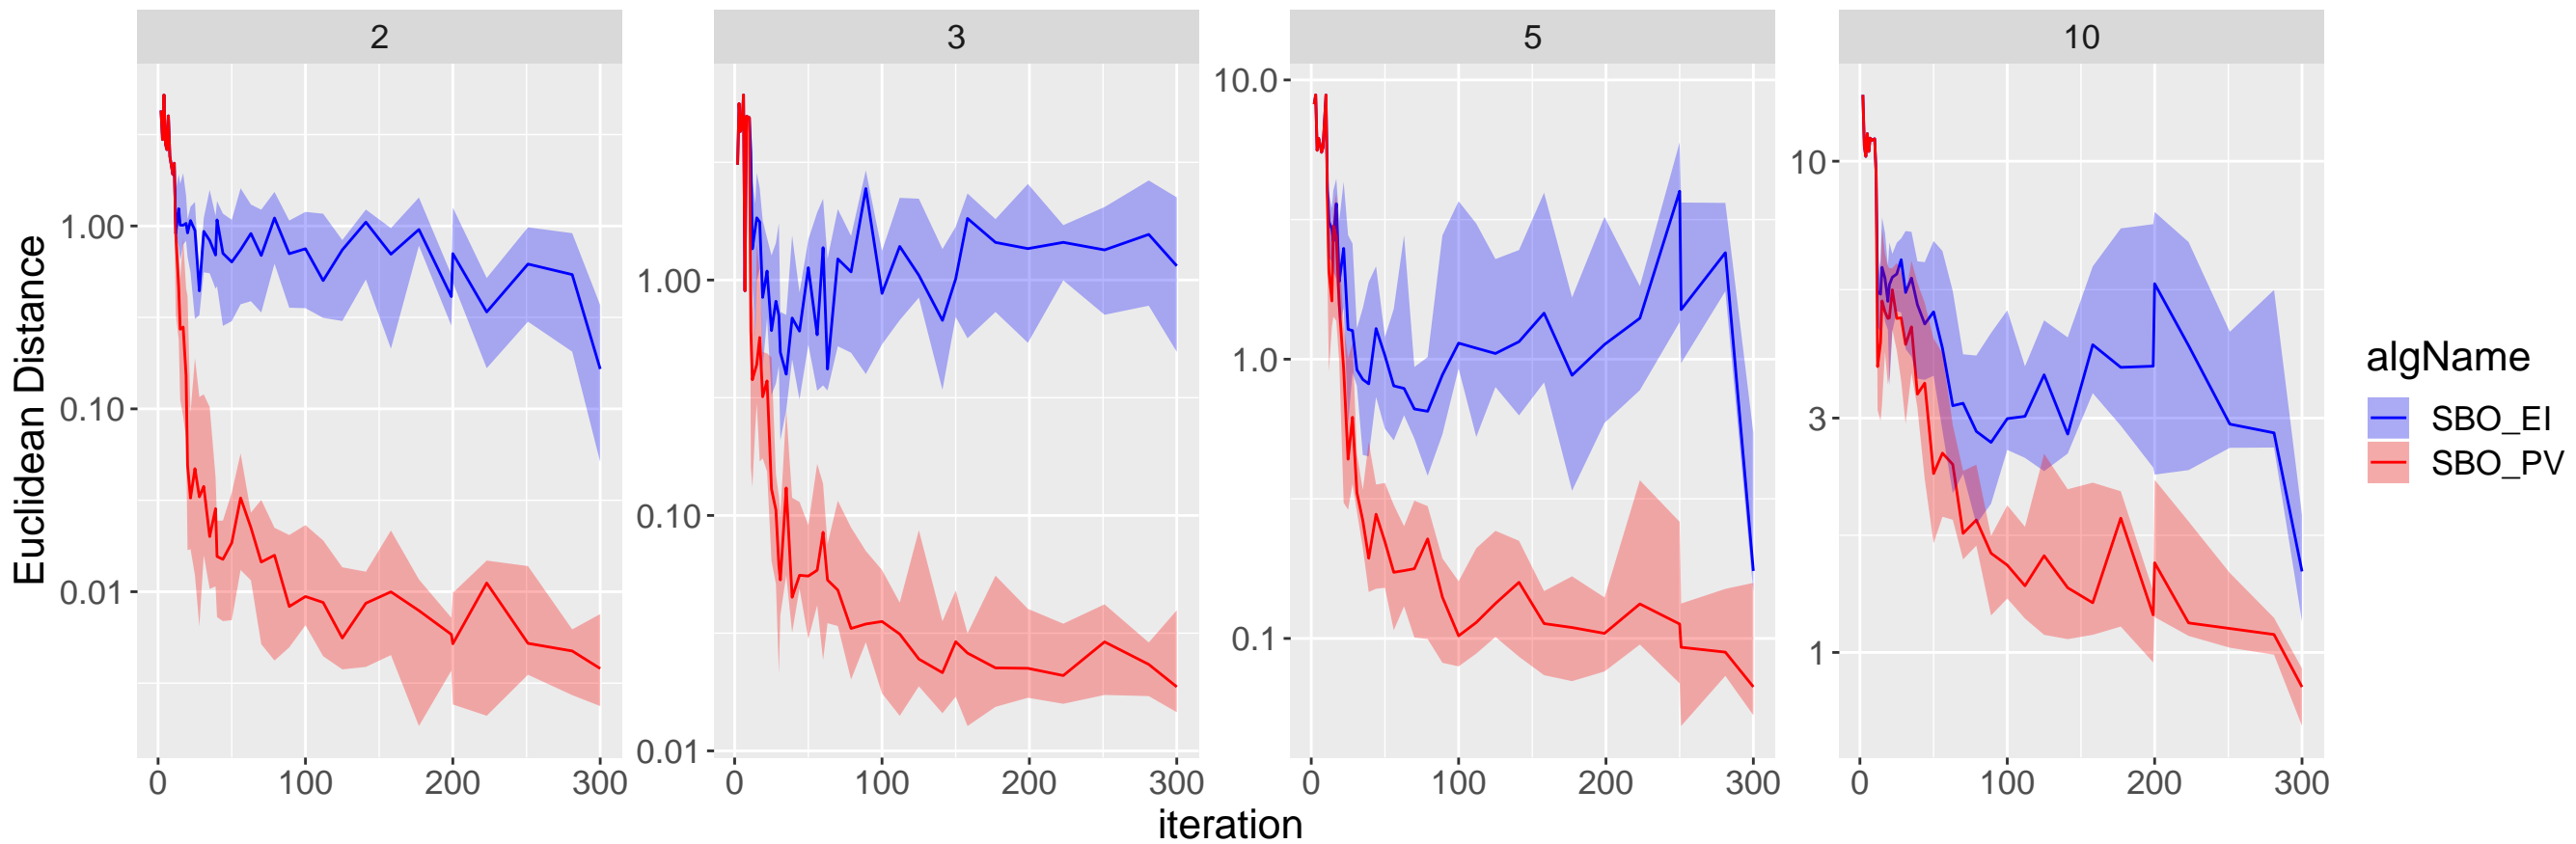

# Katsuura

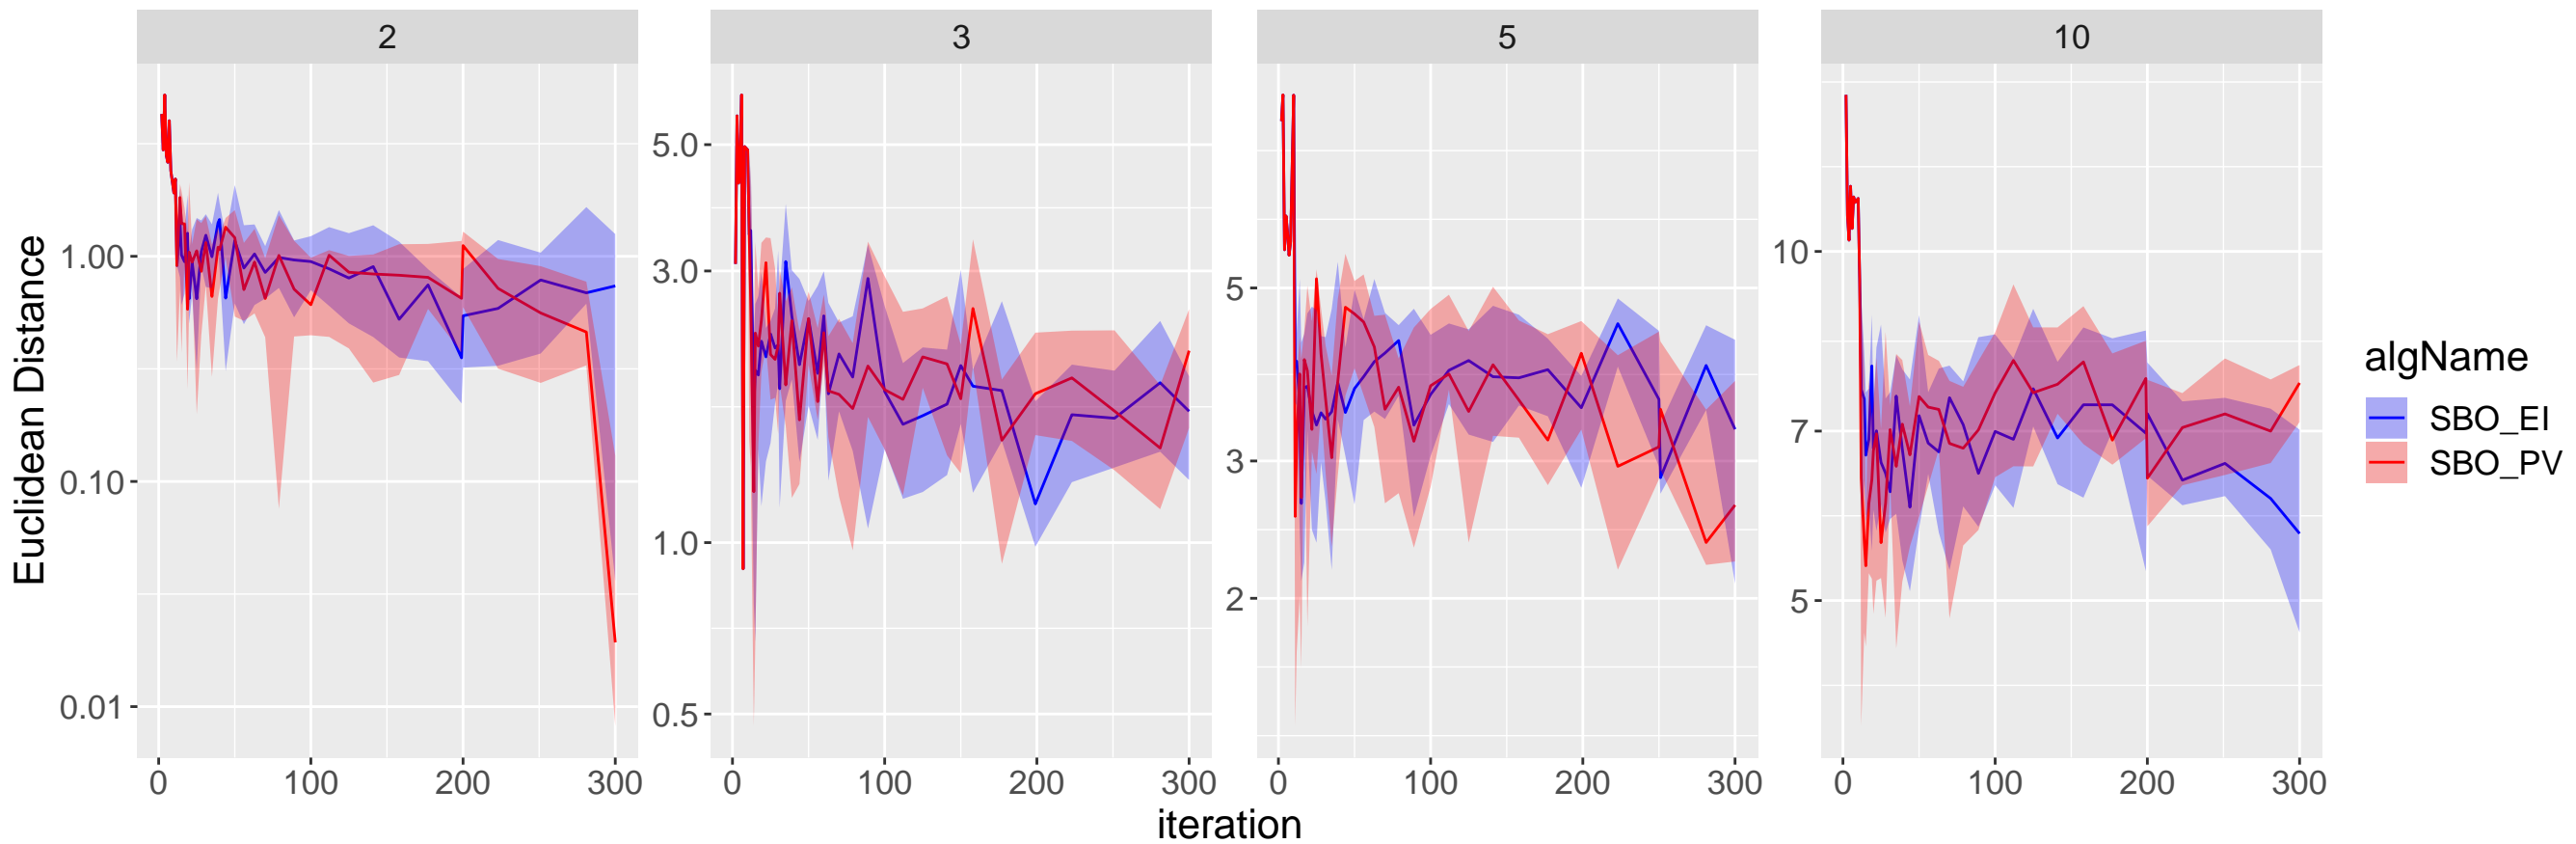

# Lunacek bi-Rastrigin

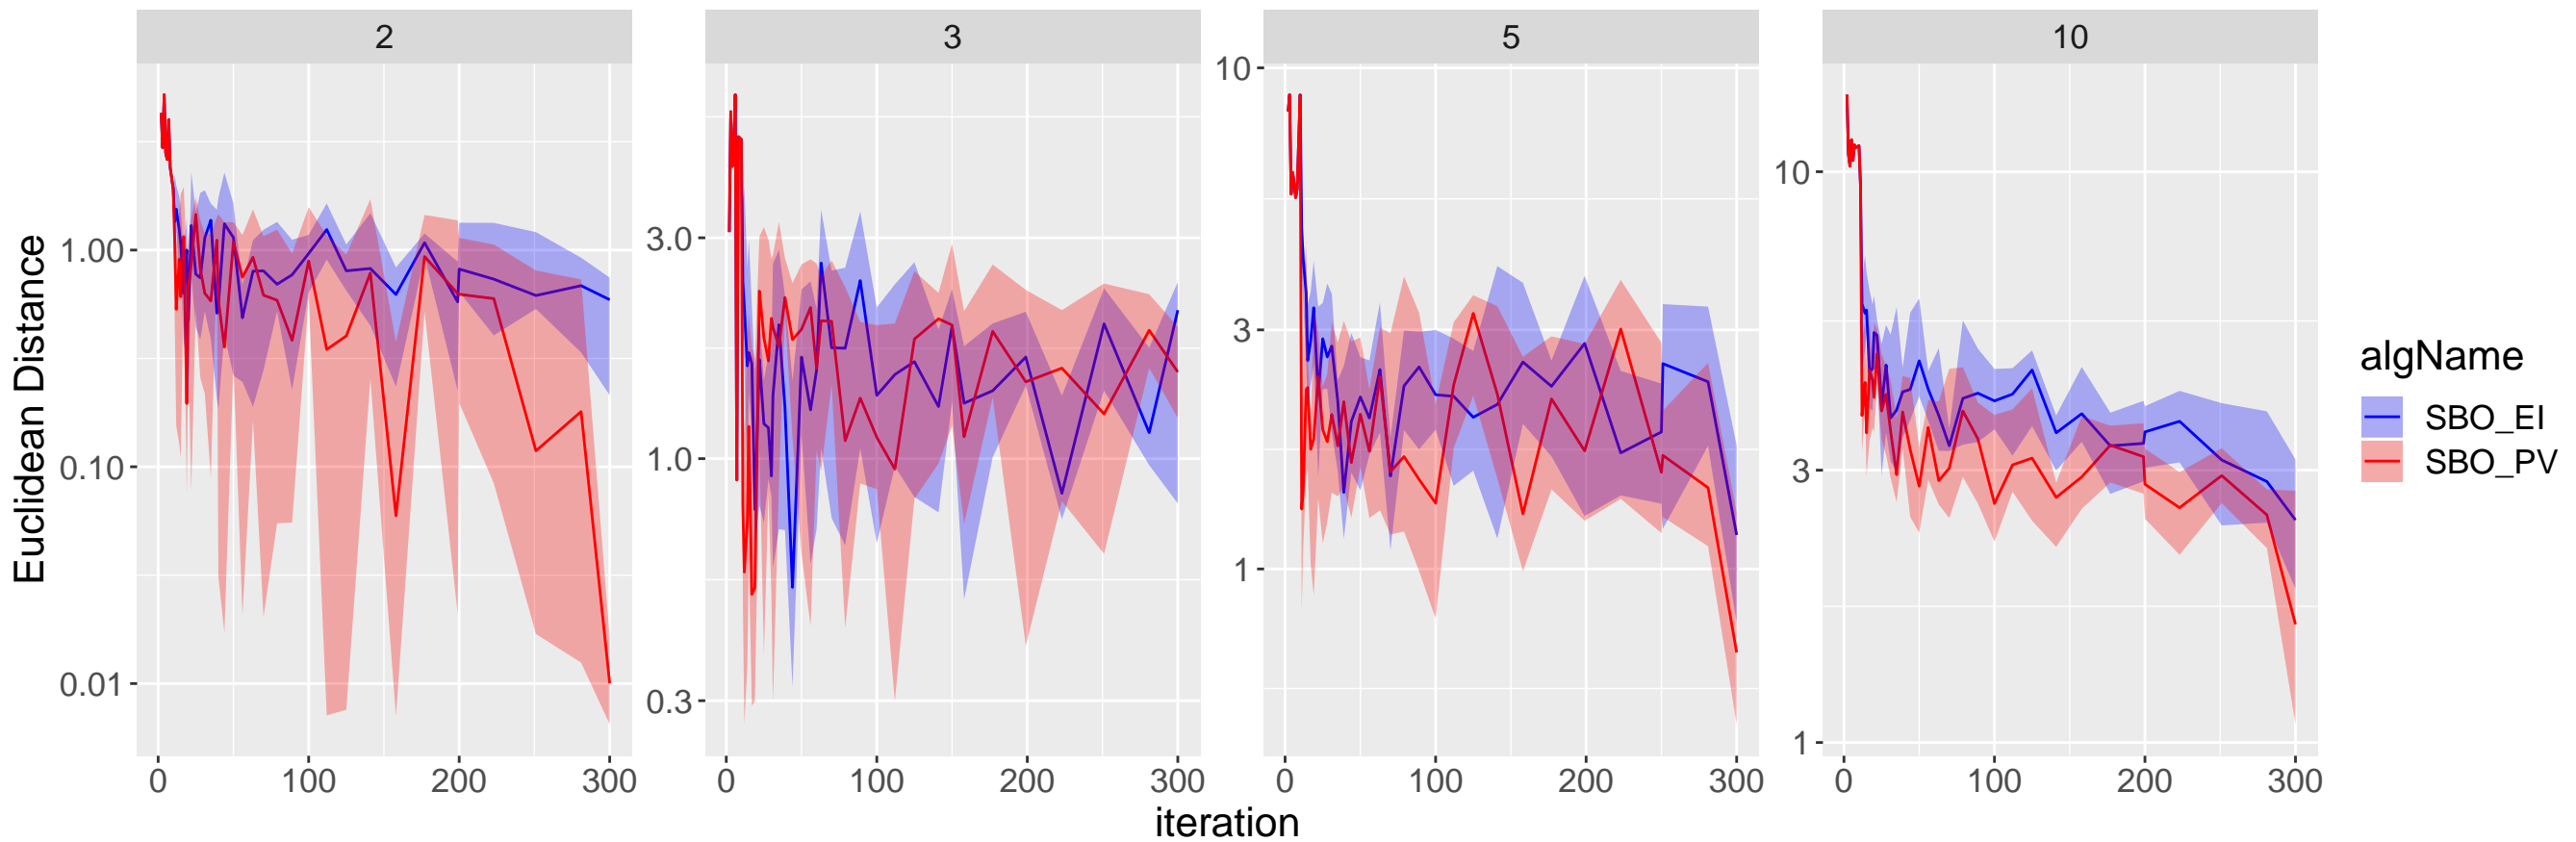

Supplement: Supplementary file 3 [file pathDistanceMLRonBBOB.pdf]
